# Supplementary material for: 3DeformRS: Certifying Spatial Deformations on Point Clouds
Source: arXiv:2204.05687 source file (2022-04-12)
Supplement: Supplementary file 1 [file supp_qualitative.tex]

\begin{figure*}
    \centering
    \begin{subfigure}[t]{0.325\linewidth}
        \includegraphics[width=\linewidth]{example-image-a}\\
        \resizebox{\linewidth}{!}{
        \begin{tabular}{c|c|c|c} \toprule
    		PointNet      & PointNet++     & DGCNN        & CurveNet     \\	\midrule
    		\cmark~Plane  & \cmark~Plane   & \xmark~Chair & \xmark~Table \\ \bottomrule
    	\end{tabular}}
        \caption{\textbf{$z-$Rotation}}
        \label{fig:QualitativeRotation}
    \end{subfigure}
    \begin{subfigure}[t]{0.325\linewidth}
        \includegraphics[width=\linewidth]{example-image-a}\\
        \resizebox{\linewidth}{!}{
        \begin{tabular}{c|c|c|c} \toprule
    		PointNet      & PointNet++     & DGCNN        & CurveNet     \\	\midrule
    		\cmark~Plane  & \cmark~Plane   & \xmark~Chair & \xmark~Table \\ \bottomrule
    	\end{tabular}}
        \caption{\textbf{$z-$Rotation}}
        \label{fig:QualitativeRotation}
    \end{subfigure}
    \begin{subfigure}[t]{0.325\linewidth}
        \includegraphics[width=\linewidth]{example-image-a}\\
        \resizebox{\linewidth}{!}{
        \begin{tabular}{c|c|c|c} \toprule
    		PointNet      & PointNet++     & DGCNN        & CurveNet     \\	\midrule
    		\cmark~Plane  & \cmark~Plane   & \xmark~Chair & \xmark~Table \\ \bottomrule
    	\end{tabular}}
        \caption{\textbf{$z-$Rotation}}
        \label{fig:QualitativeRotation}
    \end{subfigure}
    \begin{subfigure}[t]{0.325\linewidth}
        \includegraphics[width=\linewidth]{example-image-a}\\
        \resizebox{\linewidth}{!}{
        \begin{tabular}{c|c|c|c} \toprule
    		PointNet      & PointNet++     & DGCNN        & CurveNet     \\	\midrule
    		\cmark~Plane  & \cmark~Plane   & \xmark~Chair & \xmark~Table \\ \bottomrule
    	\end{tabular}}
        \caption{\textbf{$z-$Rotation}}
        \label{fig:QualitativeRotation}
    \end{subfigure}
    \begin{subfigure}[t]{0.325\linewidth}
        \includegraphics[width=\linewidth]{example-image-a}\\
        \resizebox{\linewidth}{!}{
        \begin{tabular}{c|c|c|c} \toprule
    		PointNet      & PointNet++     & DGCNN        & CurveNet     \\	\midrule
    		\cmark~Plane  & \cmark~Plane   & \xmark~Chair & \xmark~Table \\ \bottomrule
    	\end{tabular}}
        \caption{\textbf{$z-$Rotation}}
        \label{fig:QualitativeRotation}
    \end{subfigure}
    \begin{subfigure}[t]{0.325\linewidth}
        \includegraphics[width=\linewidth]{example-image-a}\\
        \resizebox{\linewidth}{!}{
        \begin{tabular}{c|c|c|c} \toprule
    		PointNet      & PointNet++     & DGCNN        & CurveNet     \\	\midrule
    		\cmark~Plane  & \cmark~Plane   & \xmark~Chair & \xmark~Table \\ \bottomrule
    	\end{tabular}}
        \caption{\textbf{$z-$Rotation}}
        \label{fig:QualitativeRotation}
    \end{subfigure}
    \begin{subfigure}[t]{0.325\linewidth}
        \includegraphics[width=\linewidth]{example-image-a}\\
        \resizebox{\linewidth}{!}{
        \begin{tabular}{c|c|c|c} \toprule
    		PointNet      & PointNet++     & DGCNN        & CurveNet     \\	\midrule
    		\cmark~Plane  & \cmark~Plane   & \xmark~Chair & \xmark~Table \\ \bottomrule
    	\end{tabular}}
        \caption{\textbf{$z-$Rotation}}
        \label{fig:QualitativeRotation}
    \end{subfigure}
    \begin{subfigure}[t]{0.325\linewidth}
        \includegraphics[width=\linewidth]{example-image-a}\\
        \resizebox{\linewidth}{!}{
        \begin{tabular}{c|c|c|c} \toprule
    		PointNet      & PointNet++     & DGCNN        & CurveNet     \\	\midrule
    		\cmark~Plane  & \cmark~Plane   & \xmark~Chair & \xmark~Table \\ \bottomrule
    	\end{tabular}}
        \caption{\textbf{$z-$Rotation}}
        \label{fig:QualitativeRotation}
    \end{subfigure}
    \begin{subfigure}[t]{0.325\linewidth}
        \includegraphics[width=\linewidth]{example-image-a}\\
        \resizebox{\linewidth}{!}{
        \begin{tabular}{c|c|c|c} \toprule
    		PointNet      & PointNet++     & DGCNN        & CurveNet     \\	\midrule
    		\cmark~Plane  & \cmark~Plane   & \xmark~Chair & \xmark~Table \\ \bottomrule
    	\end{tabular}}
        \caption{\textbf{$z-$Rotation}}
        \label{fig:QualitativeRotation}
    \end{subfigure}
    \begin{subfigure}[t]{0.325\linewidth}
        \includegraphics[width=\linewidth]{example-image-a}\\
        \resizebox{\linewidth}{!}{
        \begin{tabular}{c|c|c|c} \toprule
    		PointNet      & PointNet++     & DGCNN        & CurveNet     \\	\midrule
    		\cmark~Plane  & \cmark~Plane   & \xmark~Chair & \xmark~Table \\ \bottomrule
    	\end{tabular}}
        \caption{\textbf{$z-$Rotation}}
        \label{fig:QualitativeRotation}
    \end{subfigure}
    \label{fig:Qualitative}
    \caption{Qualitative results for different spatial deformations.}
\end{figure*}

% \begin{table*}
% 	\begin{minipage}{0.5\linewidth}
% 		\caption{Student Database}
% 		\label{table:student}
% 		\centering
% 		\begin{tabular}{lrr}
% 			\toprule
% 			Student          & h/week & Grade \\
% 			\midrule
% 			Ada Lovelace     & 2      & A \\
% 			Linus Thorvalds  & 8      & A \\
% 			Bruce Willis     & 12     & F \\
% 			Richard Stallman & 10     & B \\
% 			Grace Hopper     & 12     & A \\
% 			Alan Turing      & 8      & C \\
% 			Bill Gates       & 6      & D \\
% 			Steve Jobs       & 4      & E \\
% 			\bottomrule
% 		\end{tabular}
% 	\end{minipage}\hfill
% 	\begin{minipage}{0.45\linewidth}
% 		\centering
% 		\includegraphics[width=40mm]{example-image-a}
% 		\captionof{figure}{2-D scatterplot of the Student Database}
% 		\label{ }
% 	\end{minipage}
% \end{table*}
