# Supplementary material for: 3DeformRS: Certifying Spatial Deformations on Point Clouds
Source: arXiv:2204.05687 source file (2022-04-12)
Supplement: Supplementary file 2 [file supp_ScanObjectNN_curves_with_sigmas.tex]

\begin{figure}[h]
    \centering
    \includegraphics[width=\linewidth]{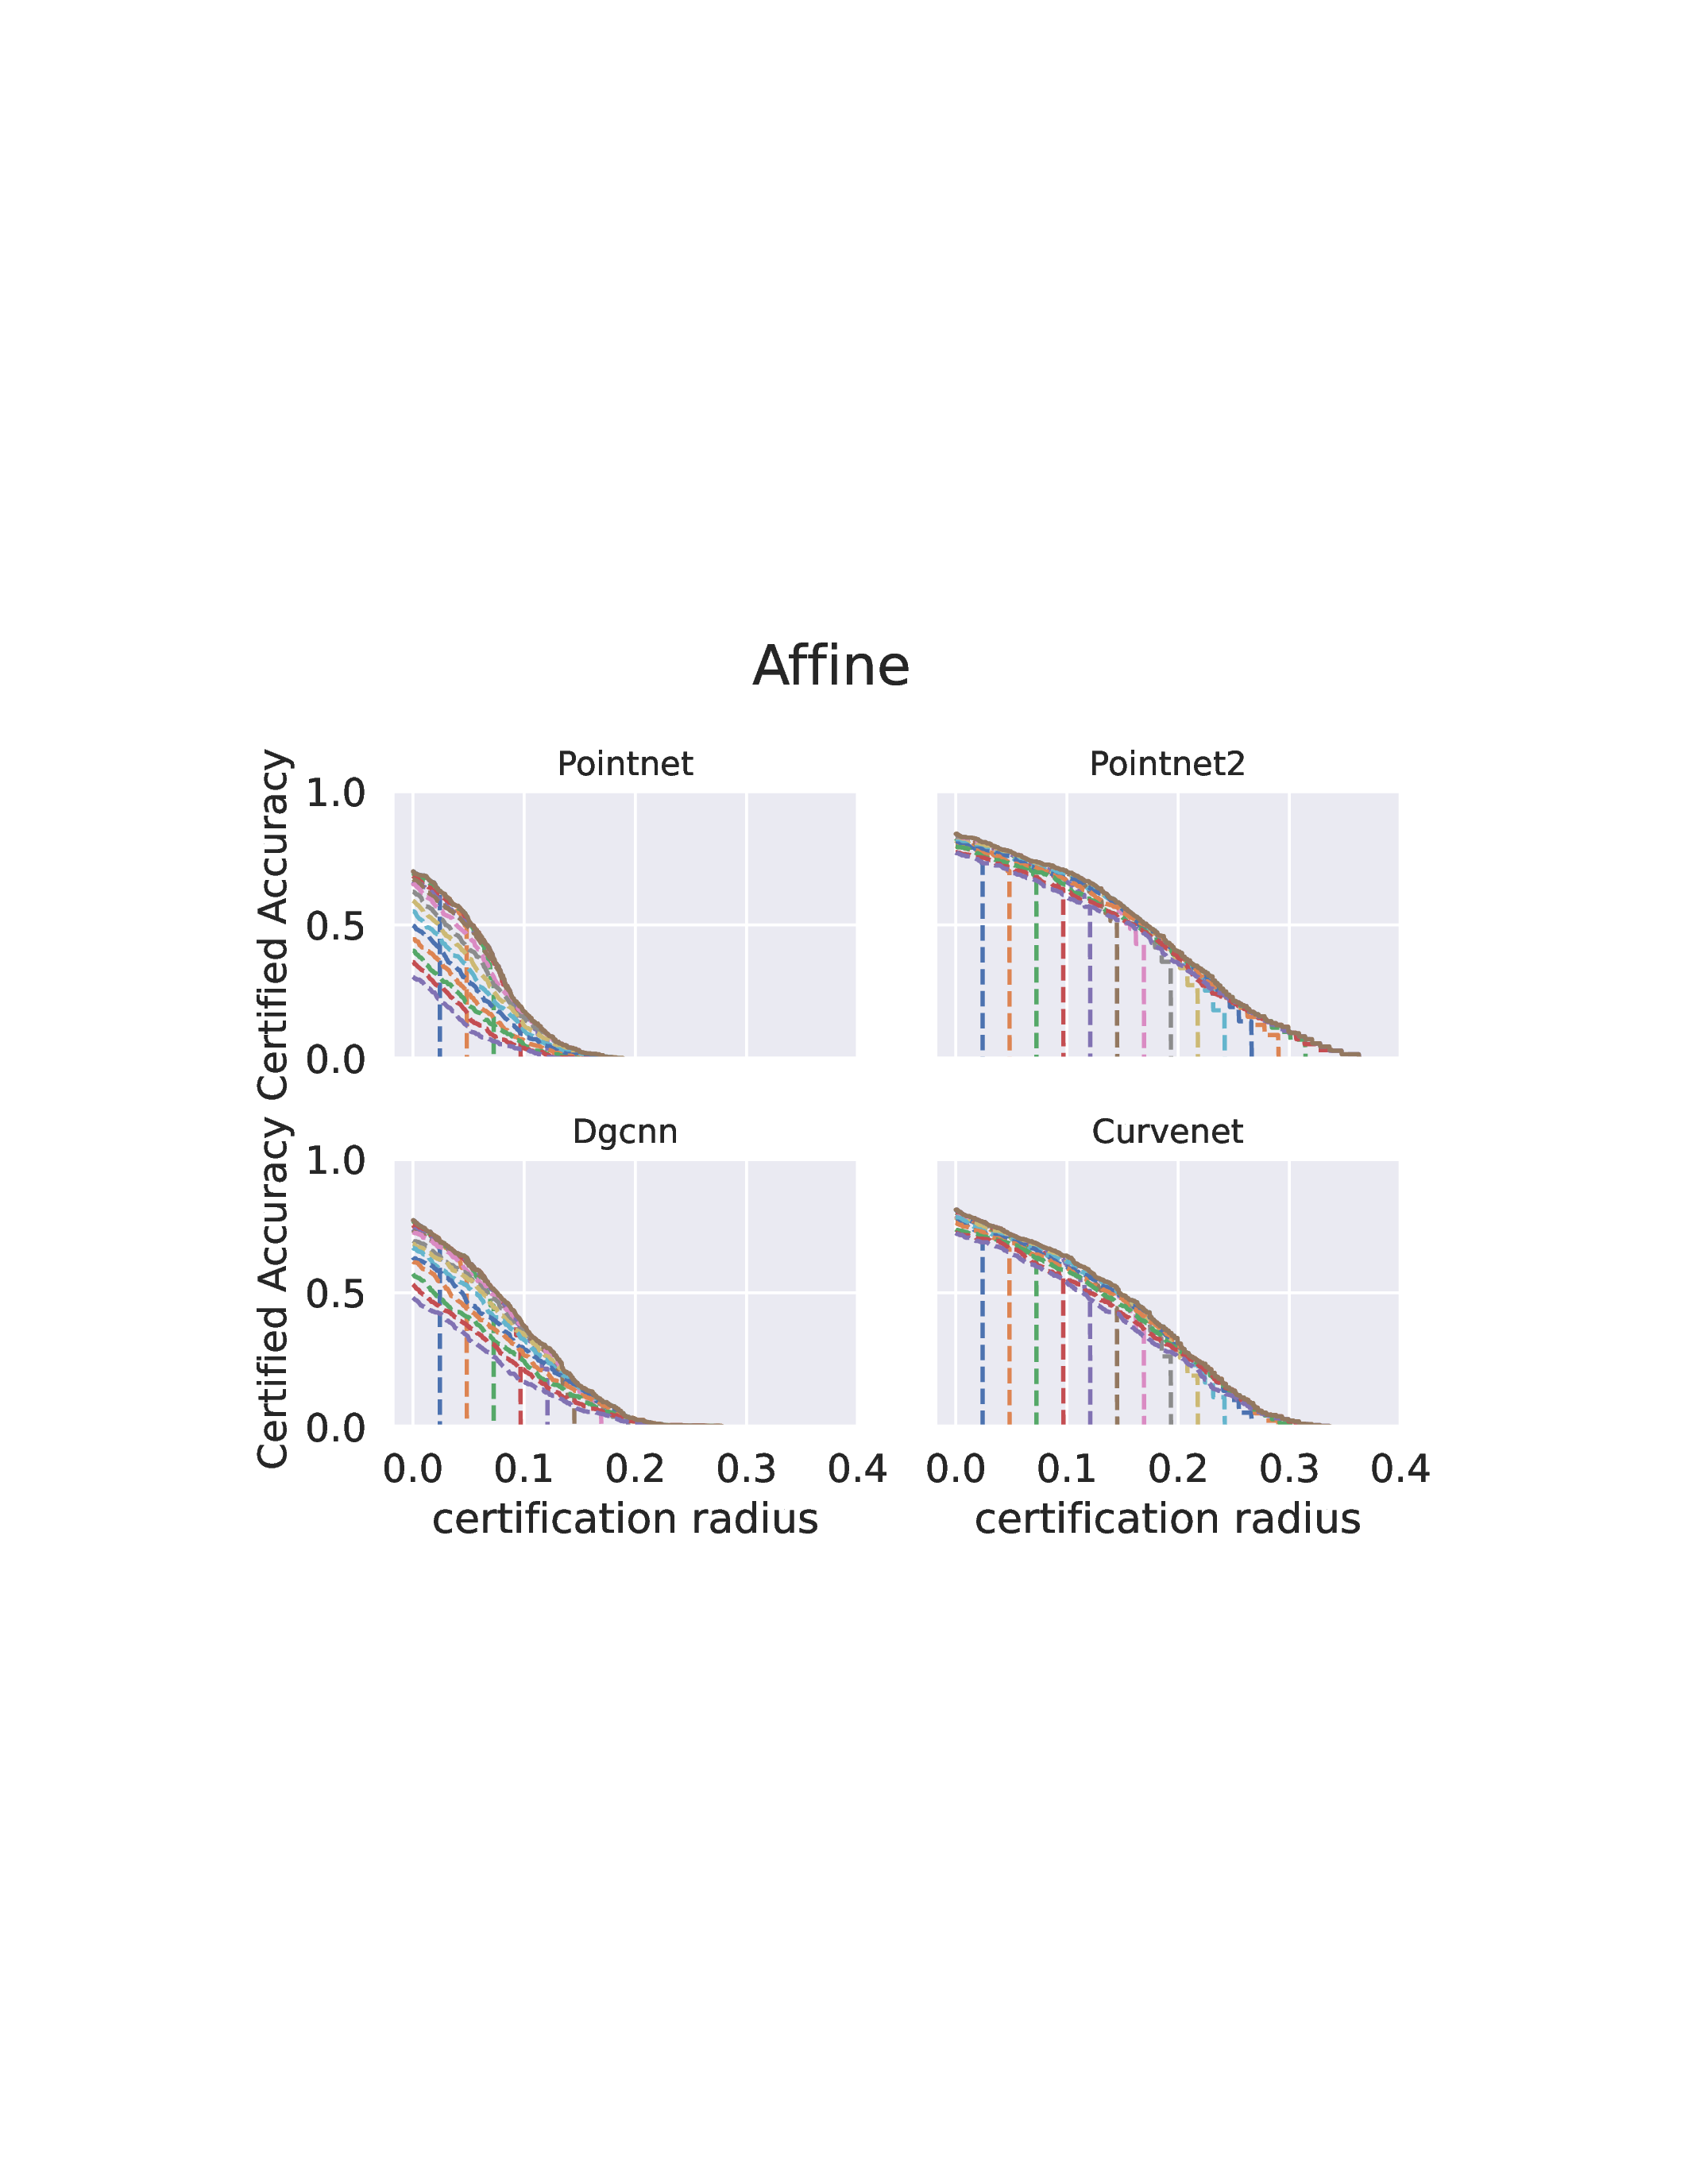}
    \includegraphics[width=\linewidth]{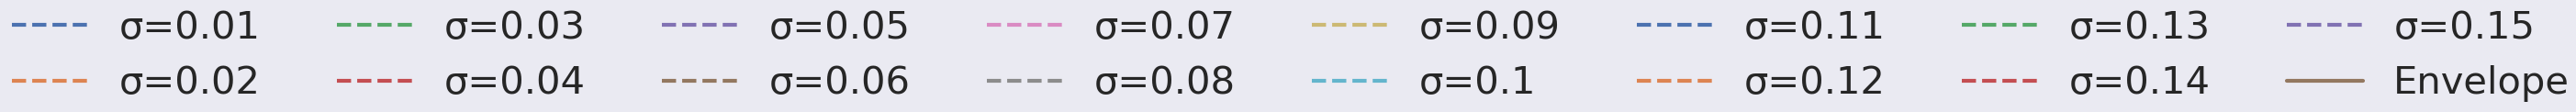}
    \caption{Certified Accuracy against Affine deformations for PointNet, PointNet++, DGCNN and CurveNet with the respective $\sigma$ values explored}
    \label{fig:SuppScanObjectNNAffine}
\end{figure}

\begin{figure}[h]
    \centering
    \includegraphics[width=\linewidth]{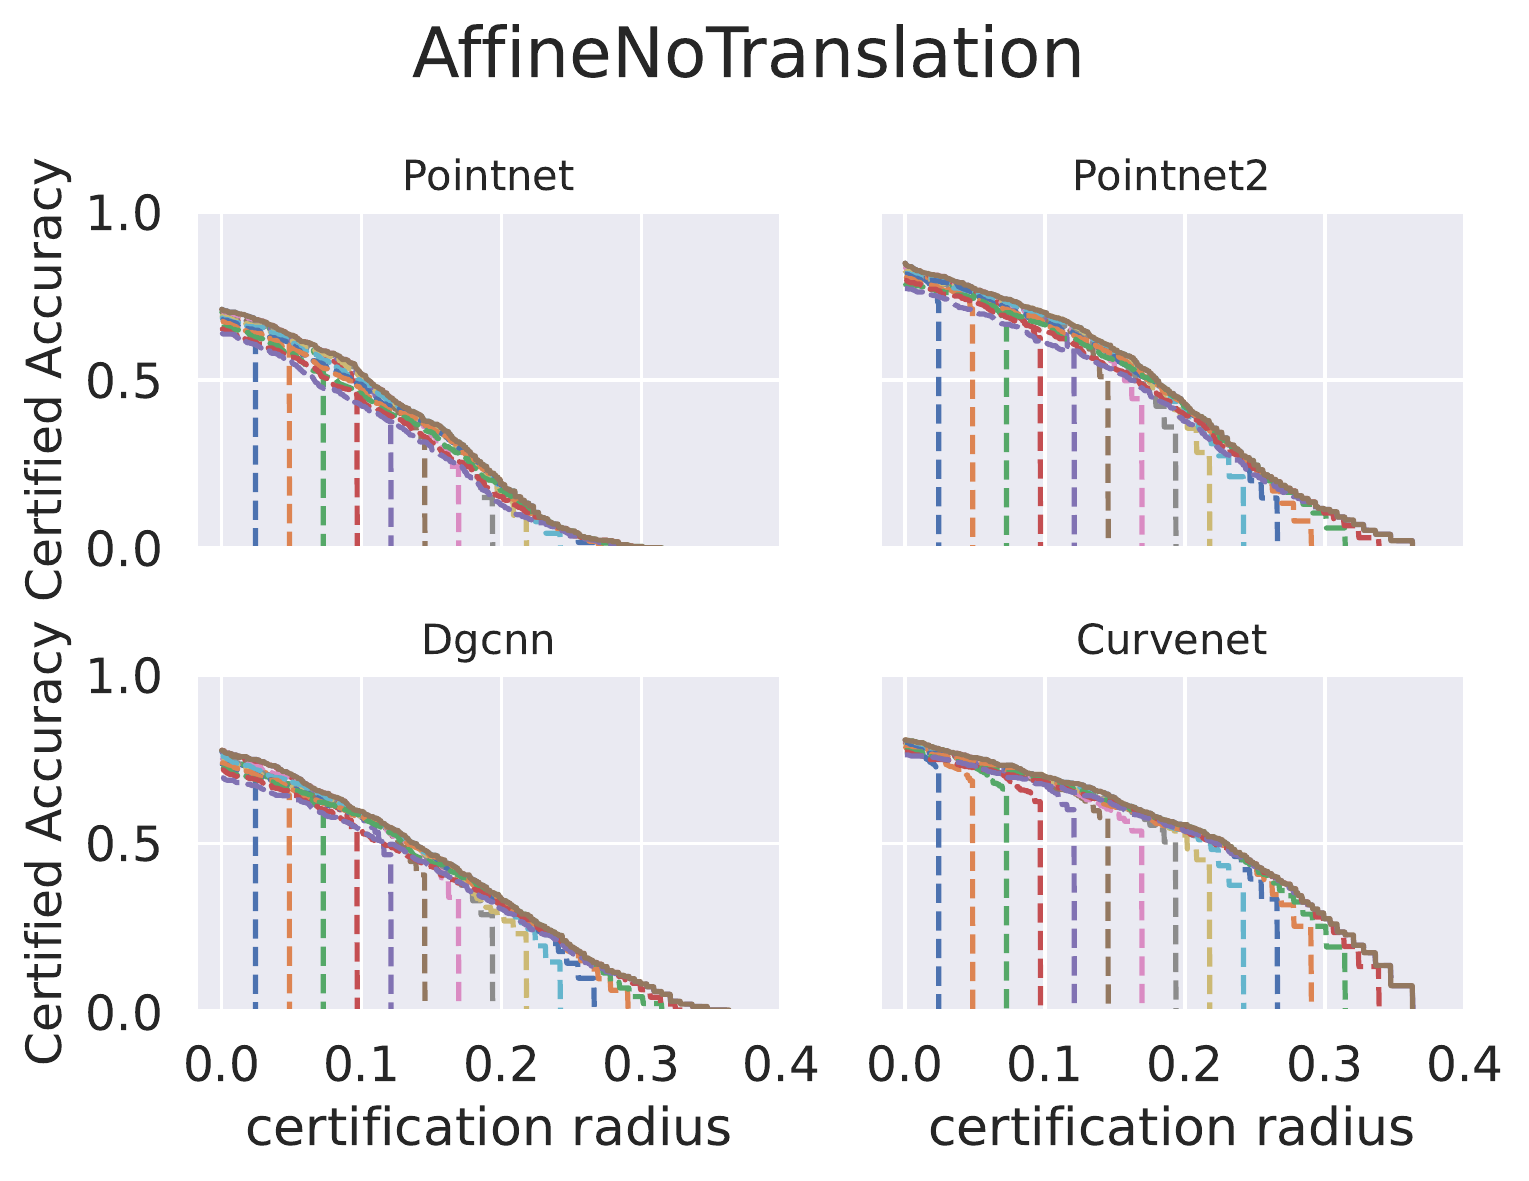}
    \includegraphics[width=\linewidth]{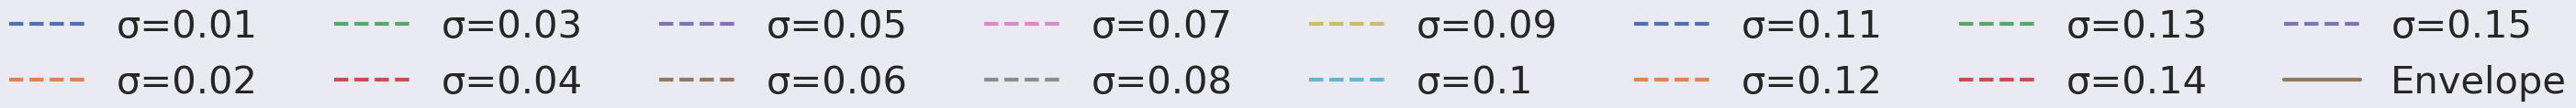}
    \caption{Certified Accuracy against Affine (NT) deformations for PointNet, PointNet++, DGCNN and CurveNet with the respective $\sigma$ values explored}
    \label{fig:SuppScanObjectNNAffineNT}
\end{figure}

\begin{figure}[h]
    \centering
    \includegraphics[width=\linewidth]{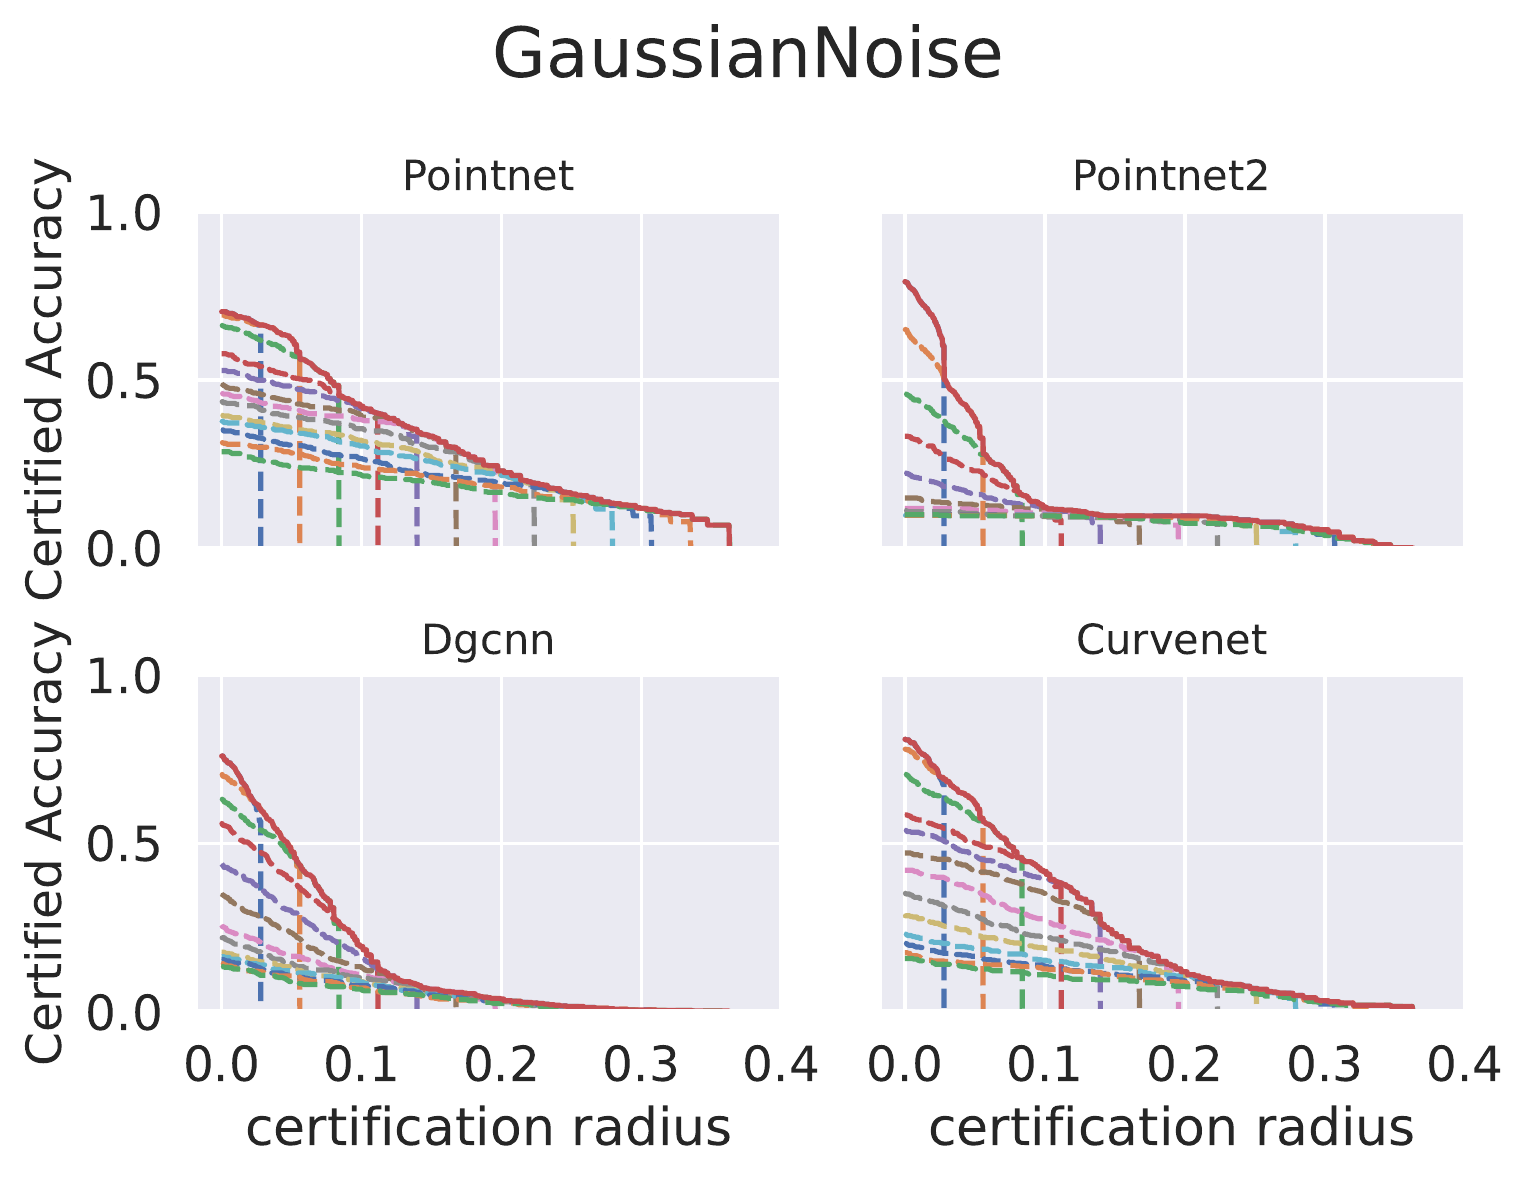}
    \includegraphics[width=\linewidth]{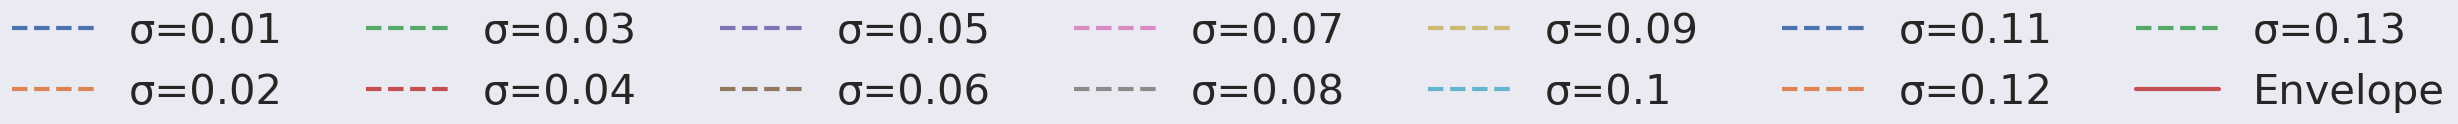}
    \caption{Certified Accuracy against Gaussian Noise deformations for PointNet, PointNet++, DGCNN and CurveNet with the respective $\sigma$ values explored}
    \label{fig:SuppScanObjectNNGaussianNoise}
\end{figure}

\begin{figure}[h]
    \centering
    \includegraphics[width=\linewidth]{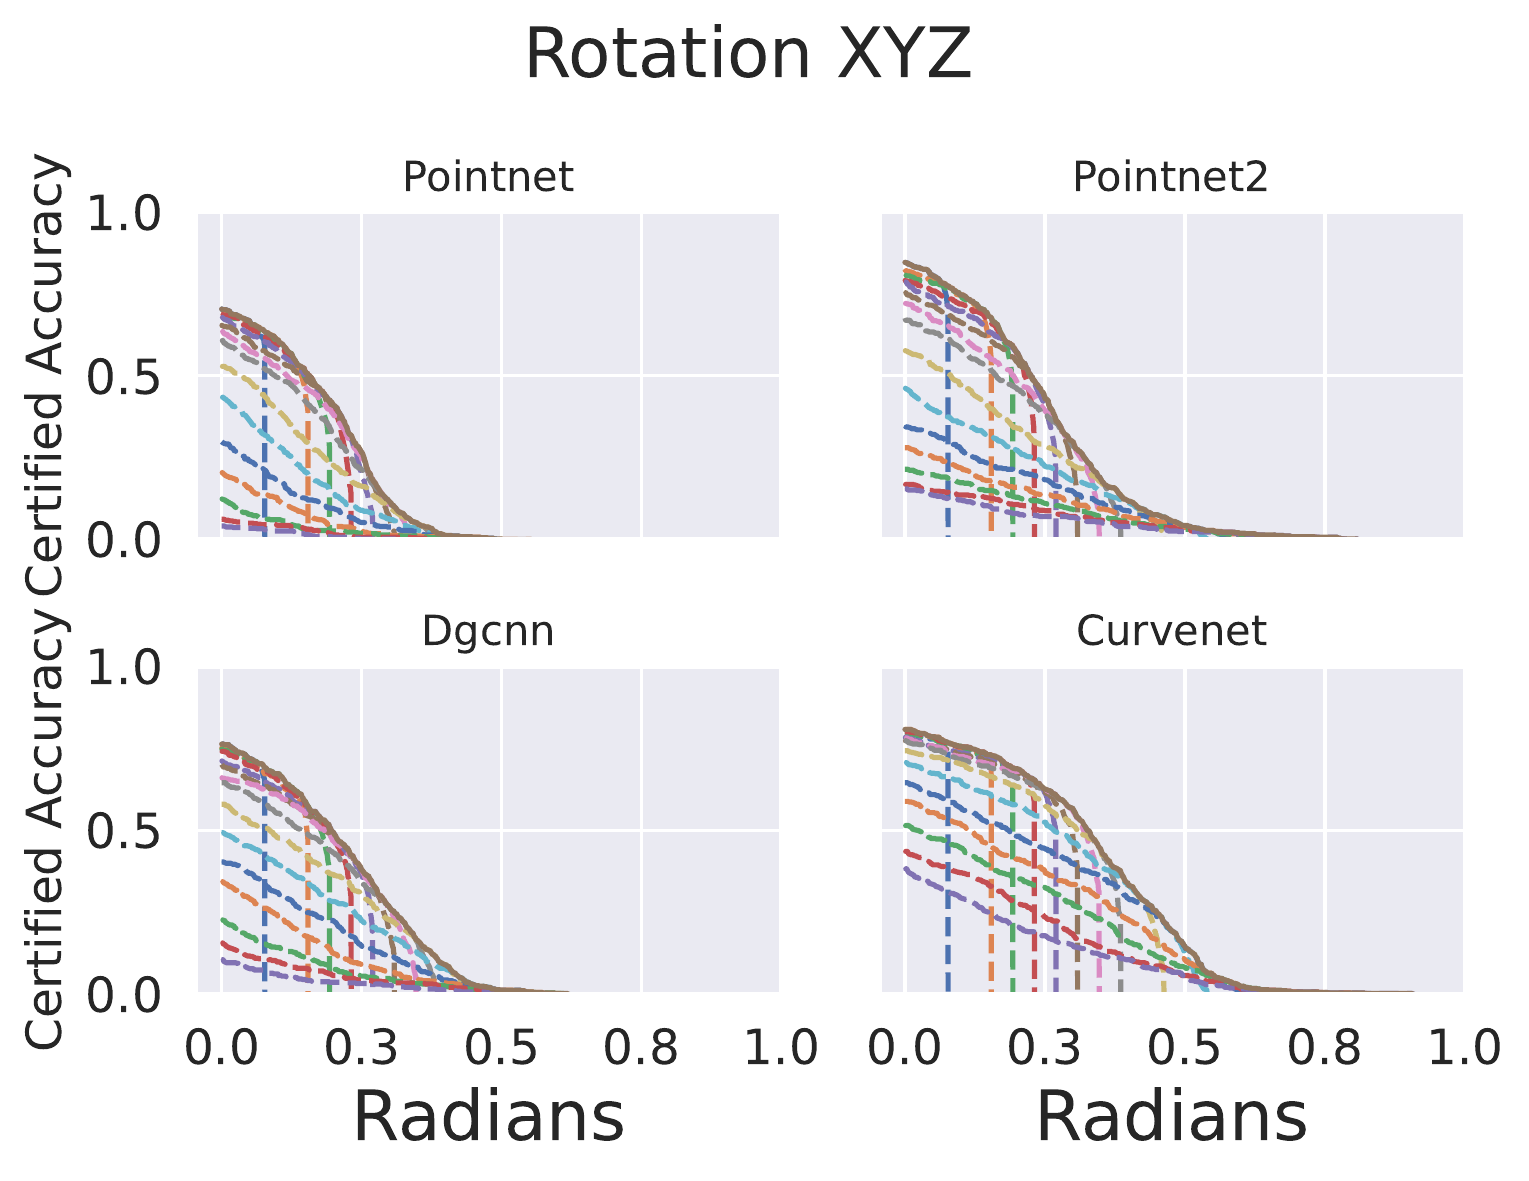}
    \includegraphics[width=\linewidth]{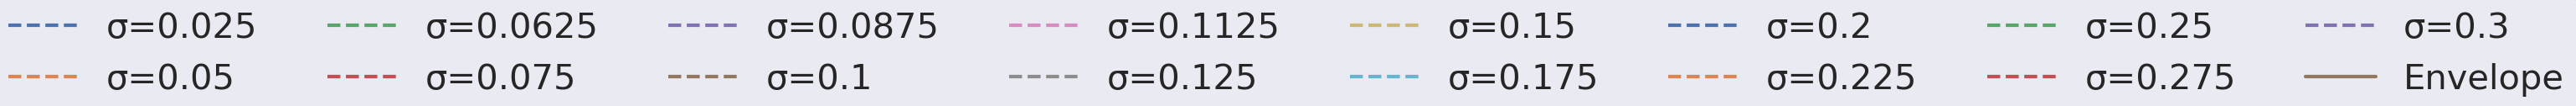}
    \caption{Certified Accuracy against Rotation XYZ deformations for PointNet, PointNet++, DGCNN and CurveNet with the respective $\sigma$ values explored}
    \label{fig:SuppScanObjectNNRotXYZ}
\end{figure}

\begin{figure}[h]
    \centering
    \includegraphics[width=\linewidth]{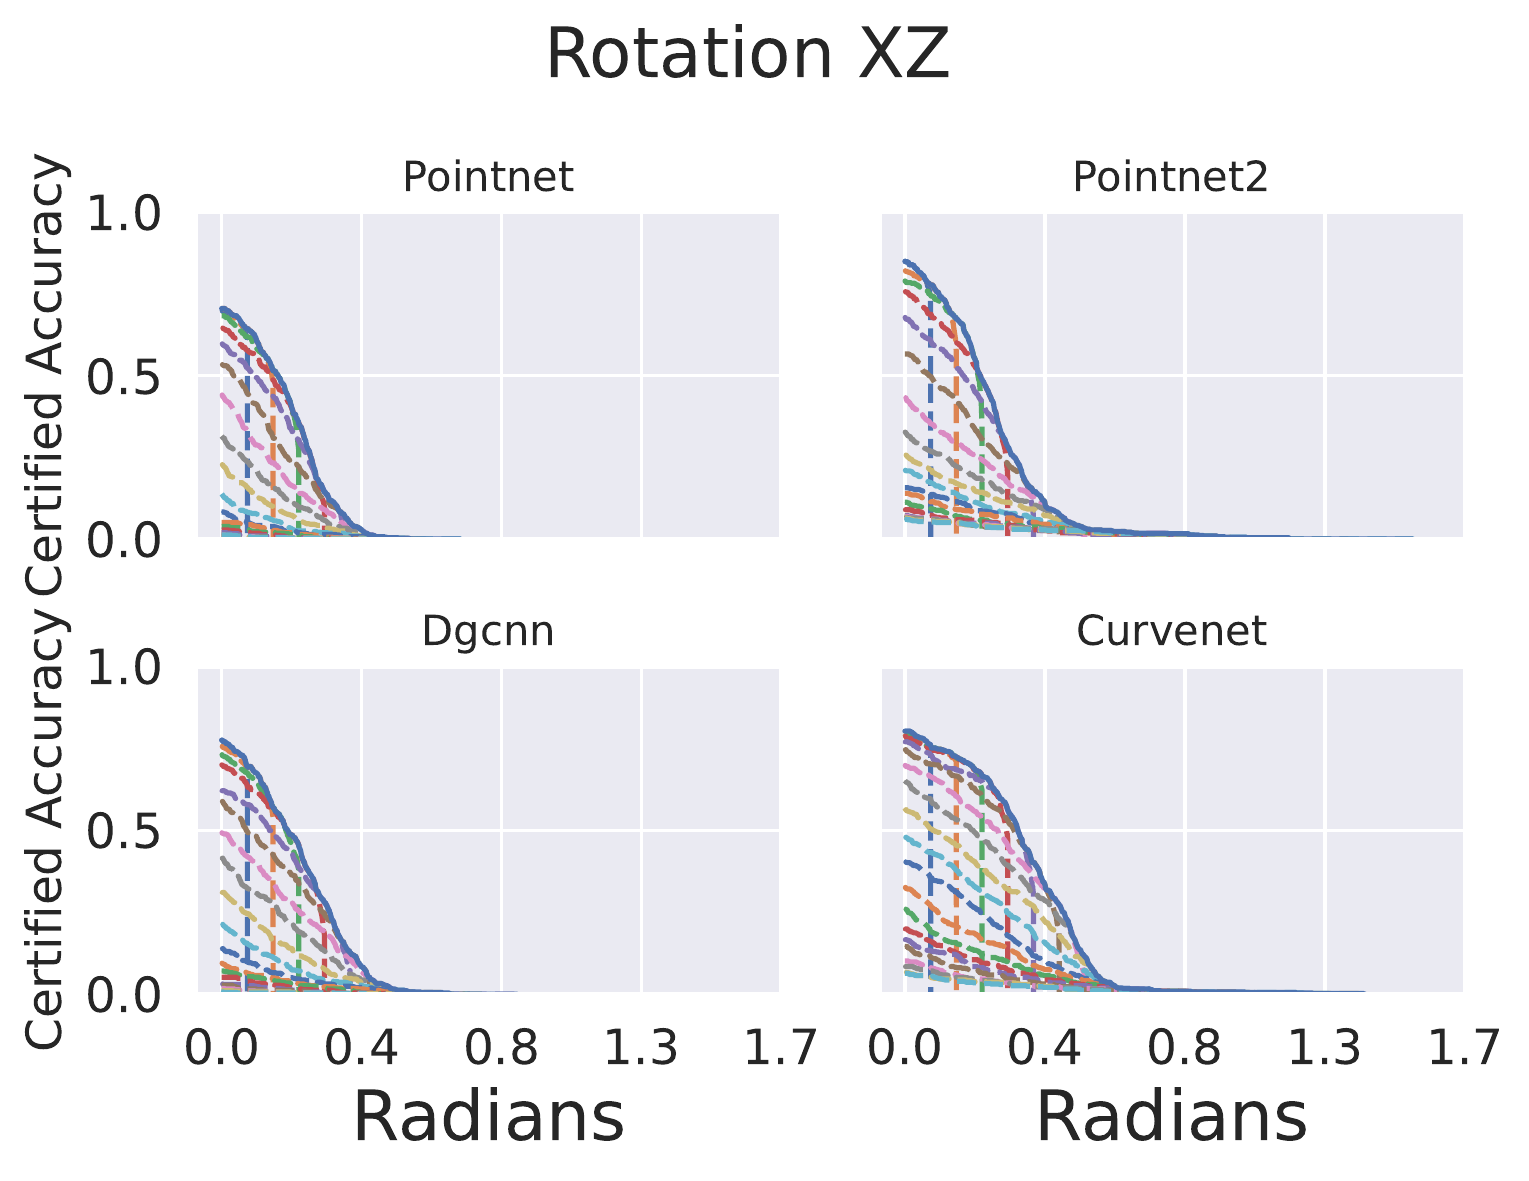}
    \includegraphics[width=\linewidth]{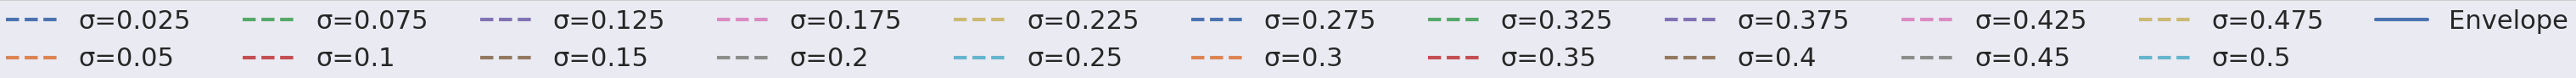}
    \caption{Certified Accuracy against Rotation XZ deformations for PointNet, PointNet++, DGCNN and CurveNet with the respective $\sigma$ values explored}
    \label{fig:SuppScanObjectNNRotXZ}
\end{figure}

\begin{figure}[h]
    \centering
    \includegraphics[width=\linewidth]{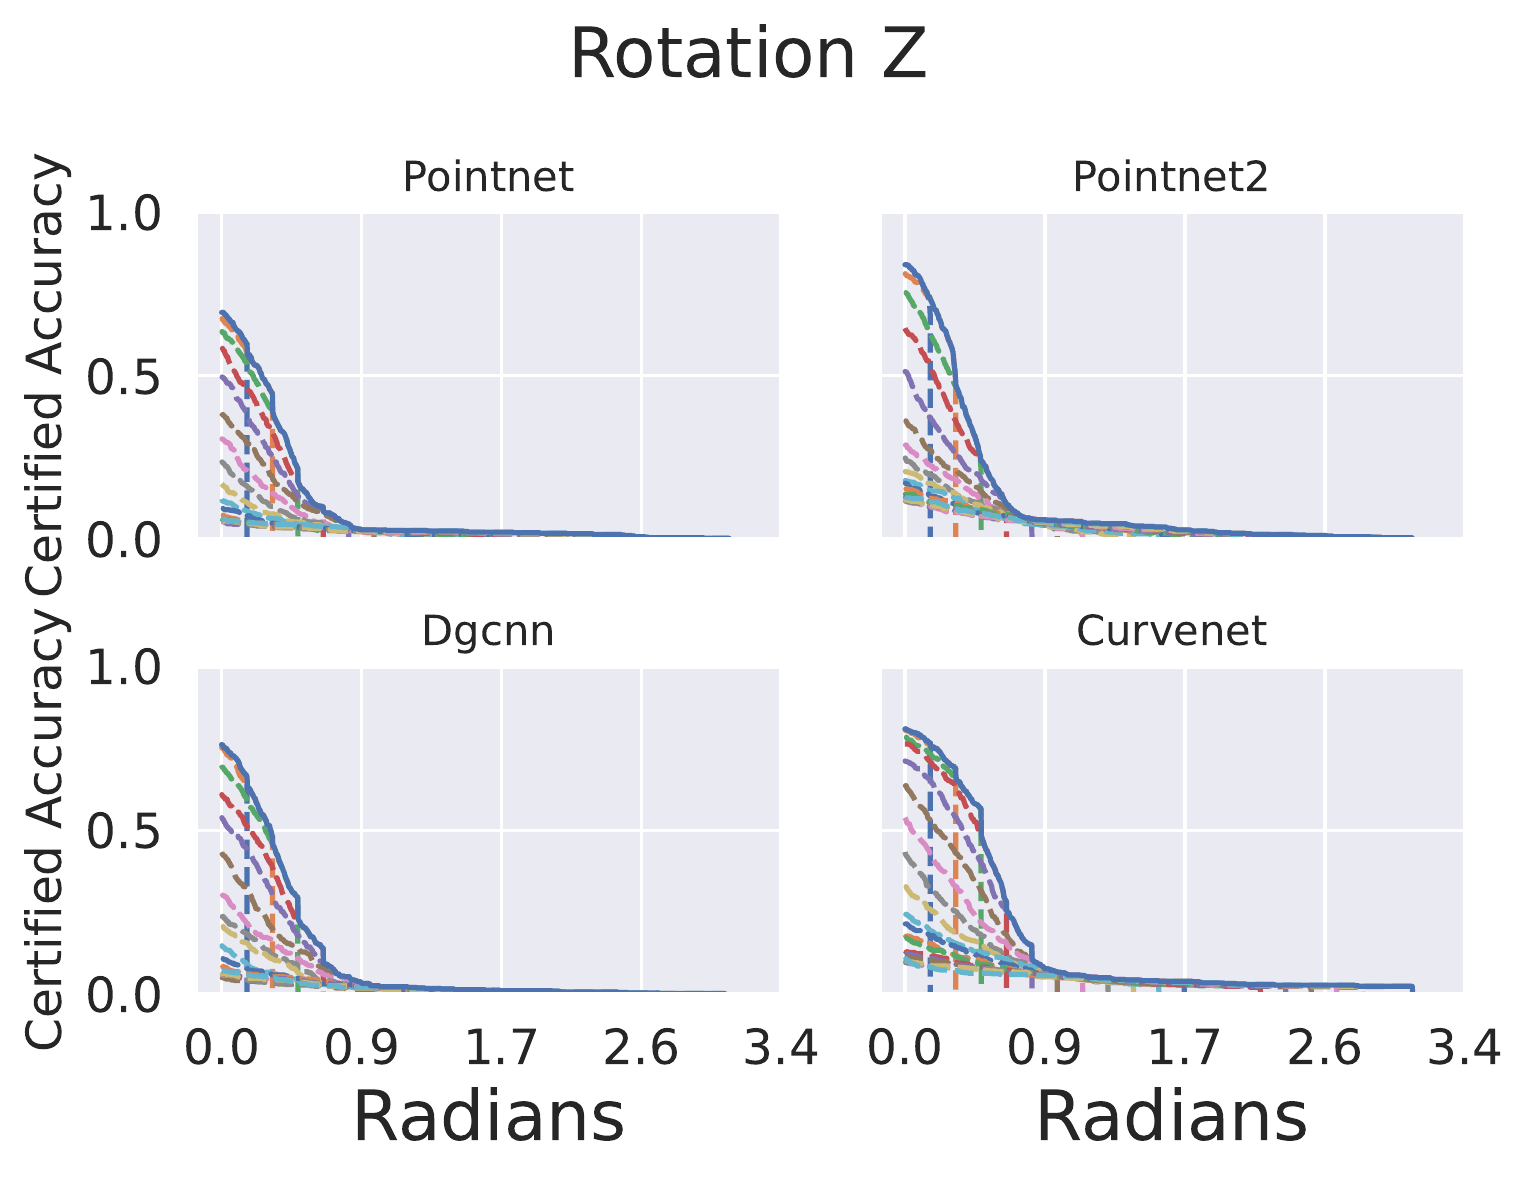}
    \includegraphics[width=\linewidth]{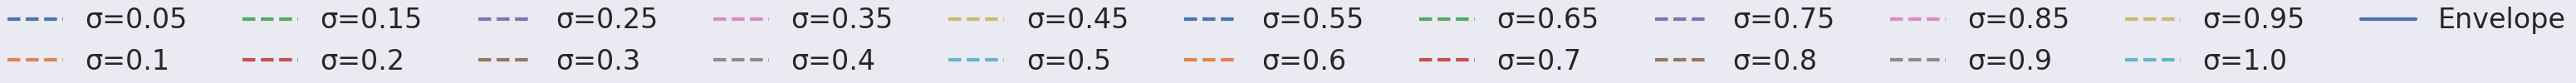}
    \caption{Certified Accuracy against Rotation Z deformations for PointNet, PointNet++, DGCNN and CurveNet with the respective $\sigma$ values explored}
    \label{fig:SuppScanObjectNNRotZ}
\end{figure}

\begin{figure}[h]
    \centering
    \includegraphics[width=\linewidth]{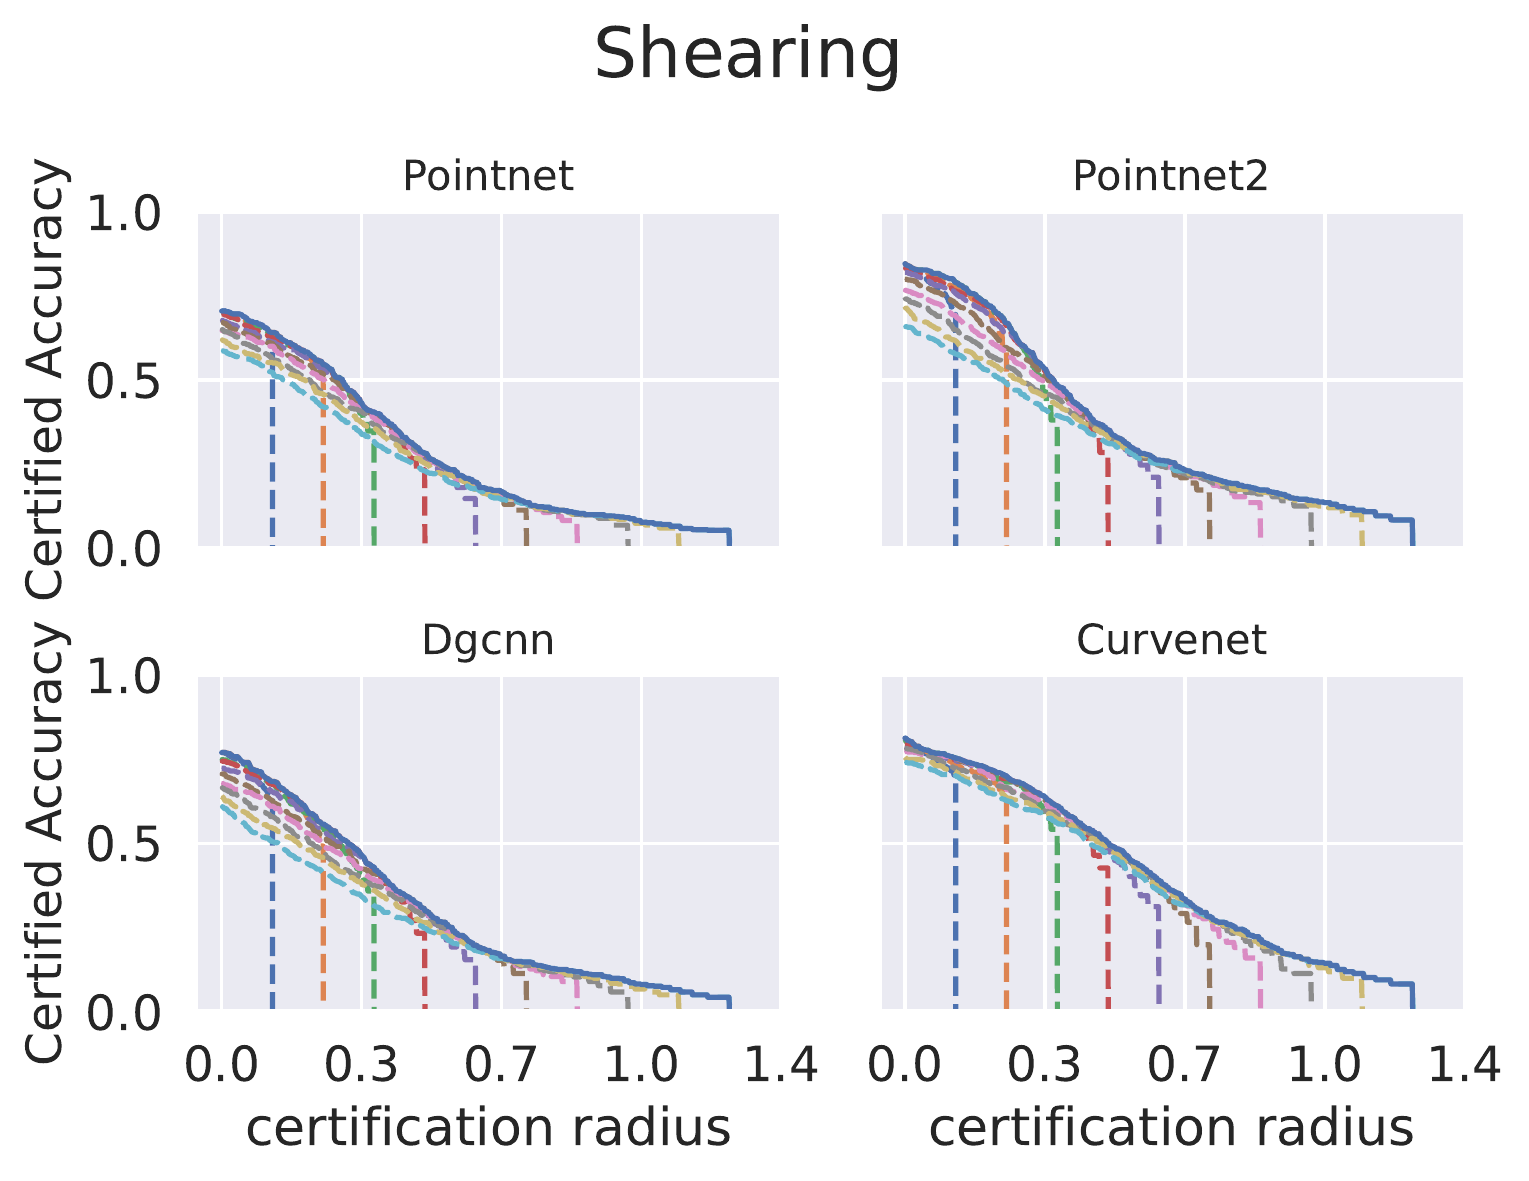}
    \includegraphics[width=\linewidth]{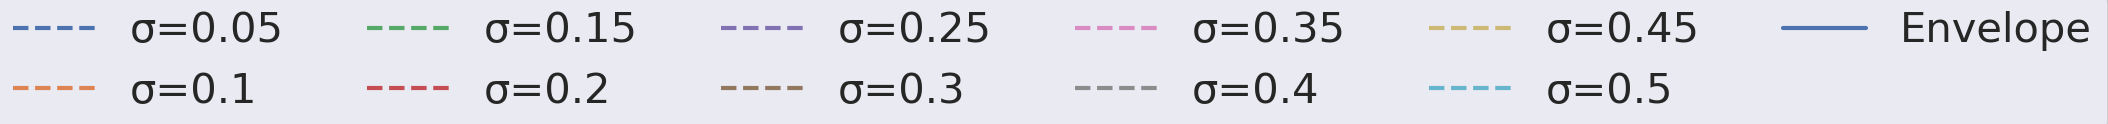}
    \caption{Certified Accuracy against Shearing deformations for PointNet, PointNet++, DGCNN and CurveNet with the respective $\sigma$ values explored}
    \label{fig:SuppScanObjectNNShearing}
\end{figure}

\begin{figure}[h]
    \centering
    \includegraphics[width=\linewidth]{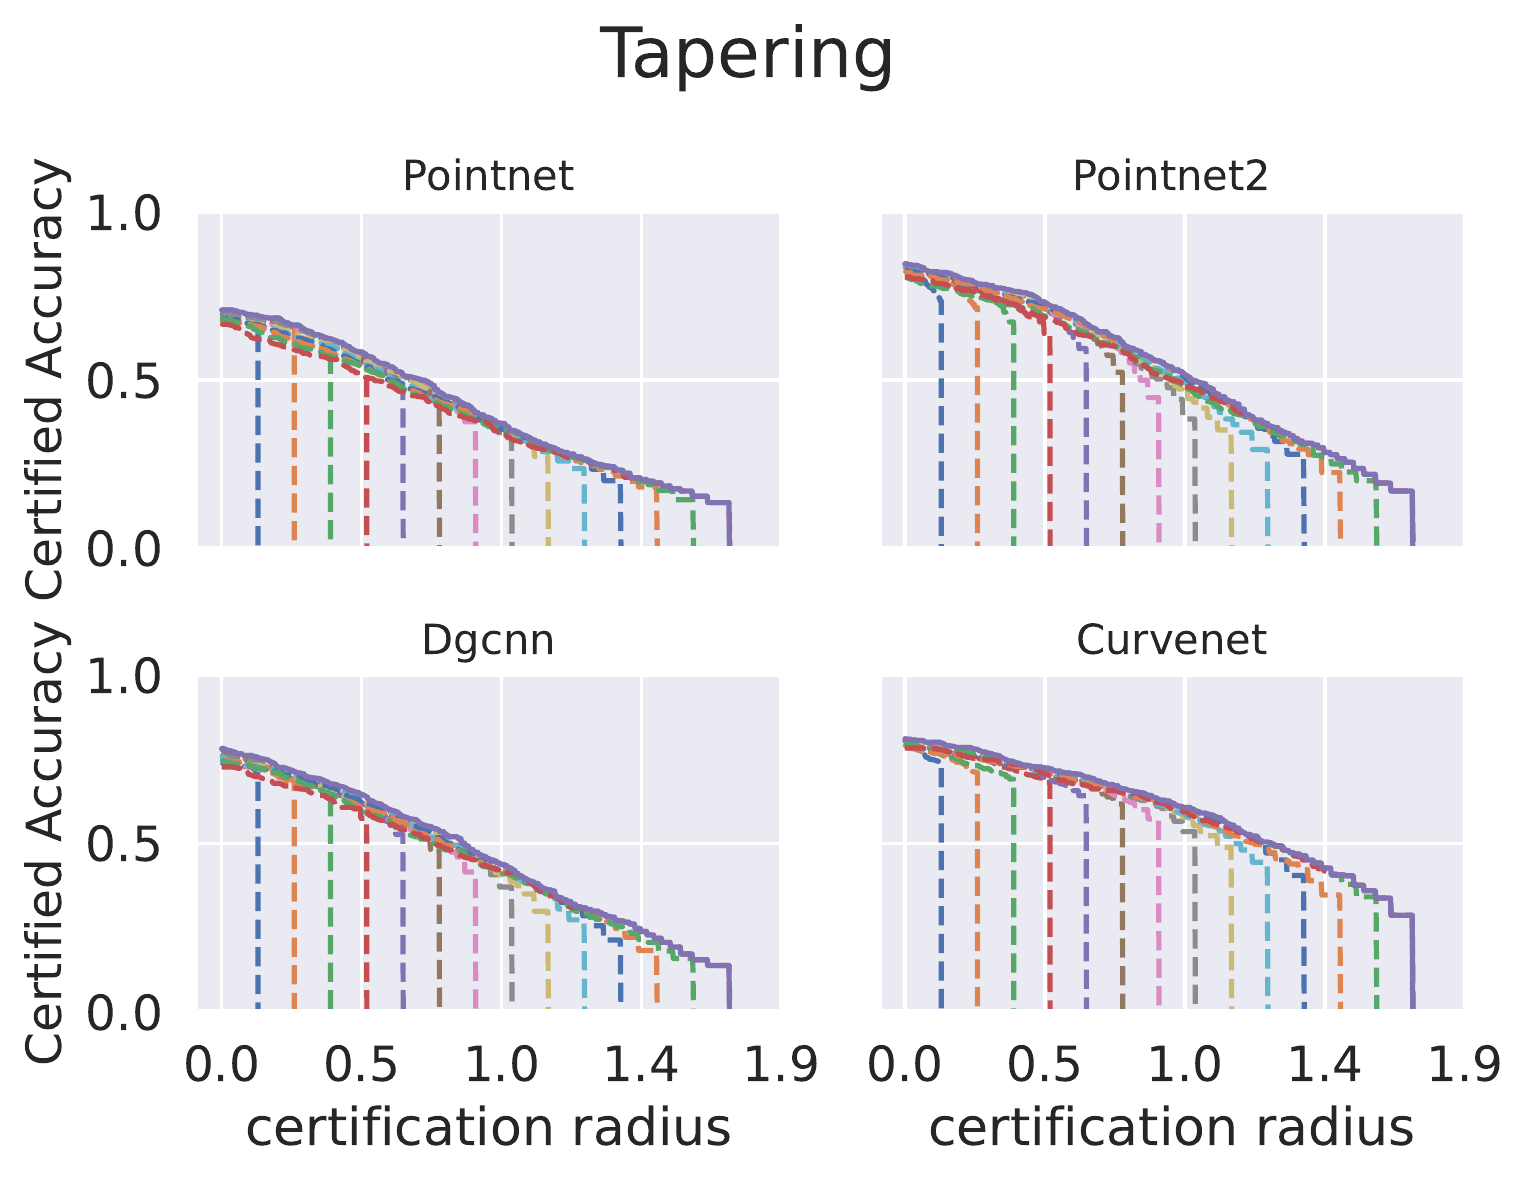}
    \includegraphics[width=\linewidth]{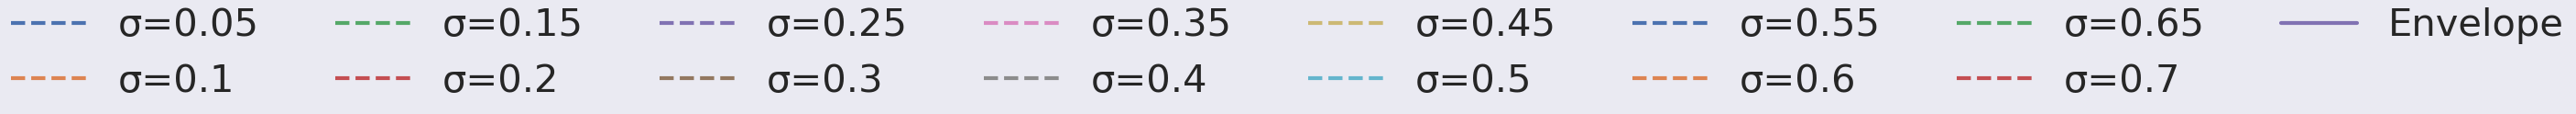}
    \caption{Certified Accuracy against Tapering deformations for PointNet, PointNet++, DGCNN and CurveNet with the respective $\sigma$ values explored}
    \label{fig:SuppScanObjectNNTapering}
\end{figure}

\begin{figure}[h]
    \centering
    \includegraphics[width=\linewidth]{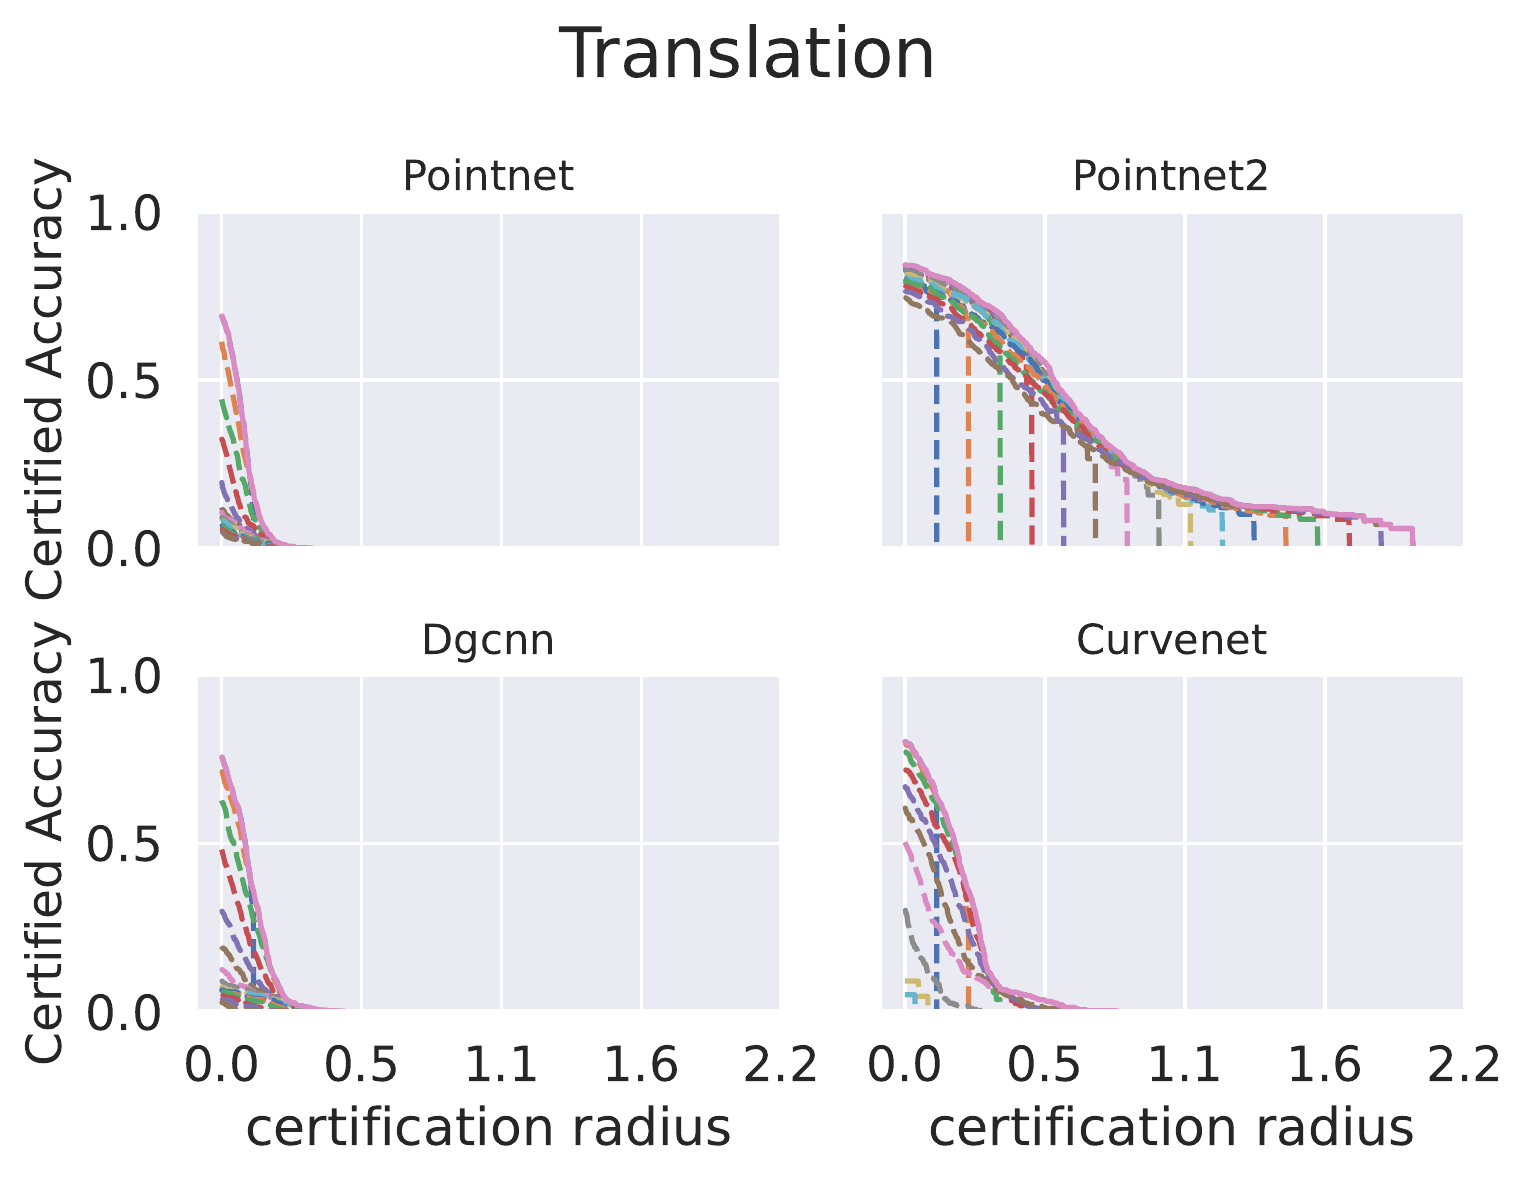}
    \includegraphics[width=\linewidth]{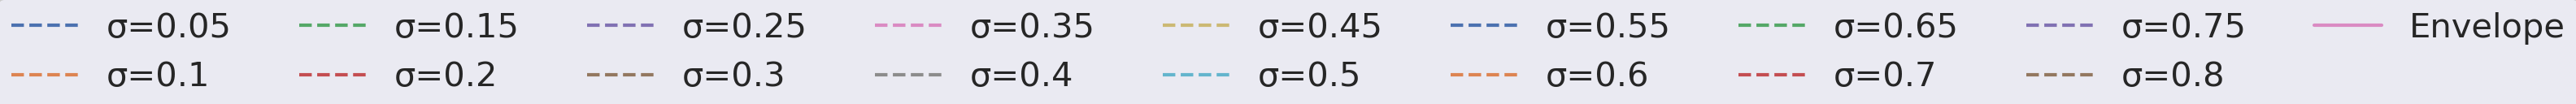}
    \caption{Certified Accuracy against Translation for PointNet, PointNet++, DGCNN and CurveNet with the respective $\sigma$ values explored}
    \label{fig:SuppScanObjectNNTranslation}
\end{figure}

\begin{figure}[h]
    \centering
    \includegraphics[width=\linewidth]{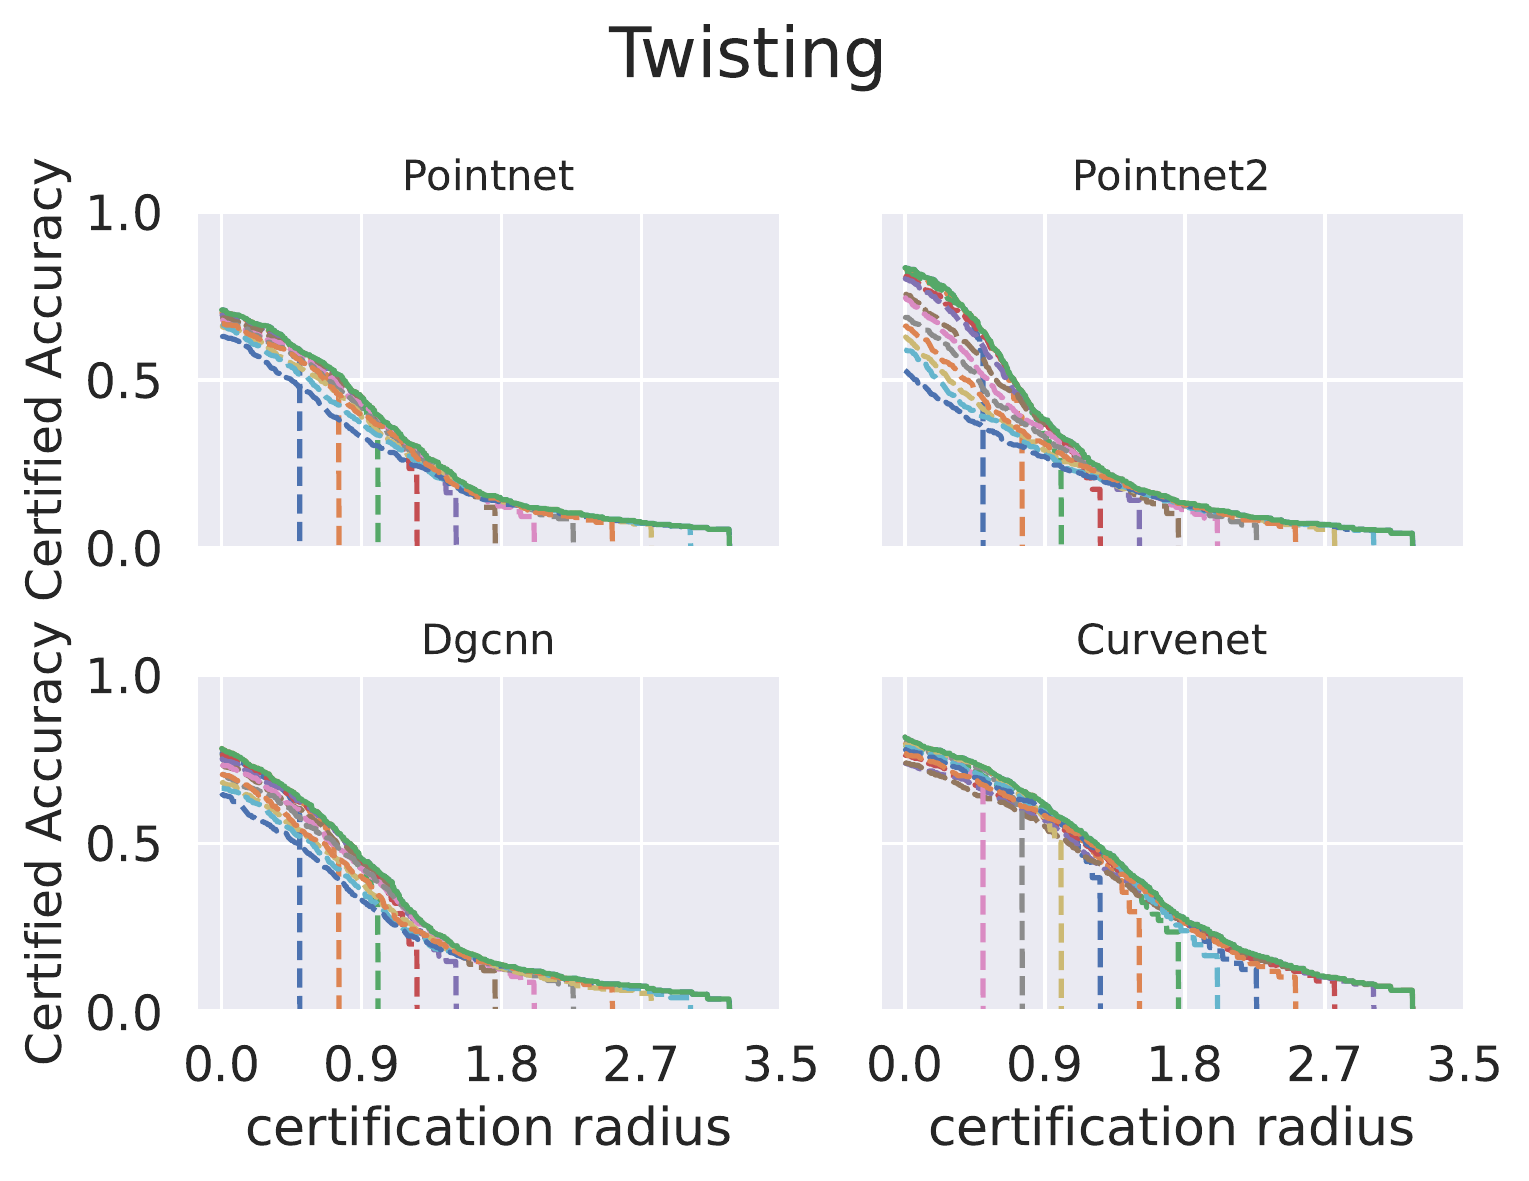}
    \includegraphics[width=\linewidth]{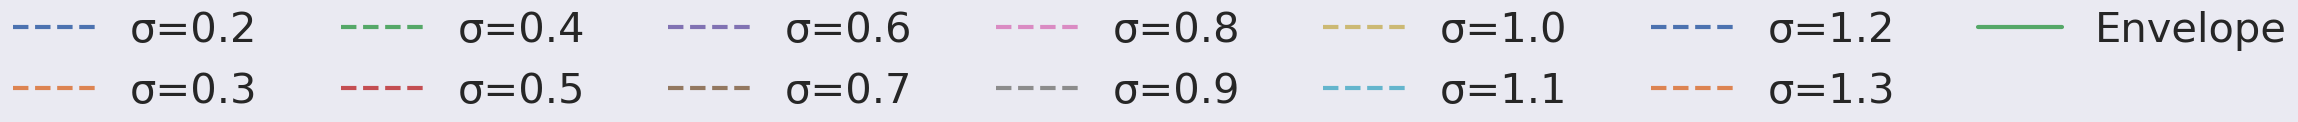}
    \caption{Certified Accuracy against Twisting deformations for PointNet, PointNet++, DGCNN and CurveNet with the respective $\sigma$ values explored}
    \label{fig:SuppScanObjectNNTwisting}
\end{figure}

\begin{figure*}[h]
    \centering
    \includegraphics[width=0.45\linewidth,trim=0 0 0 1.5cm, clip]{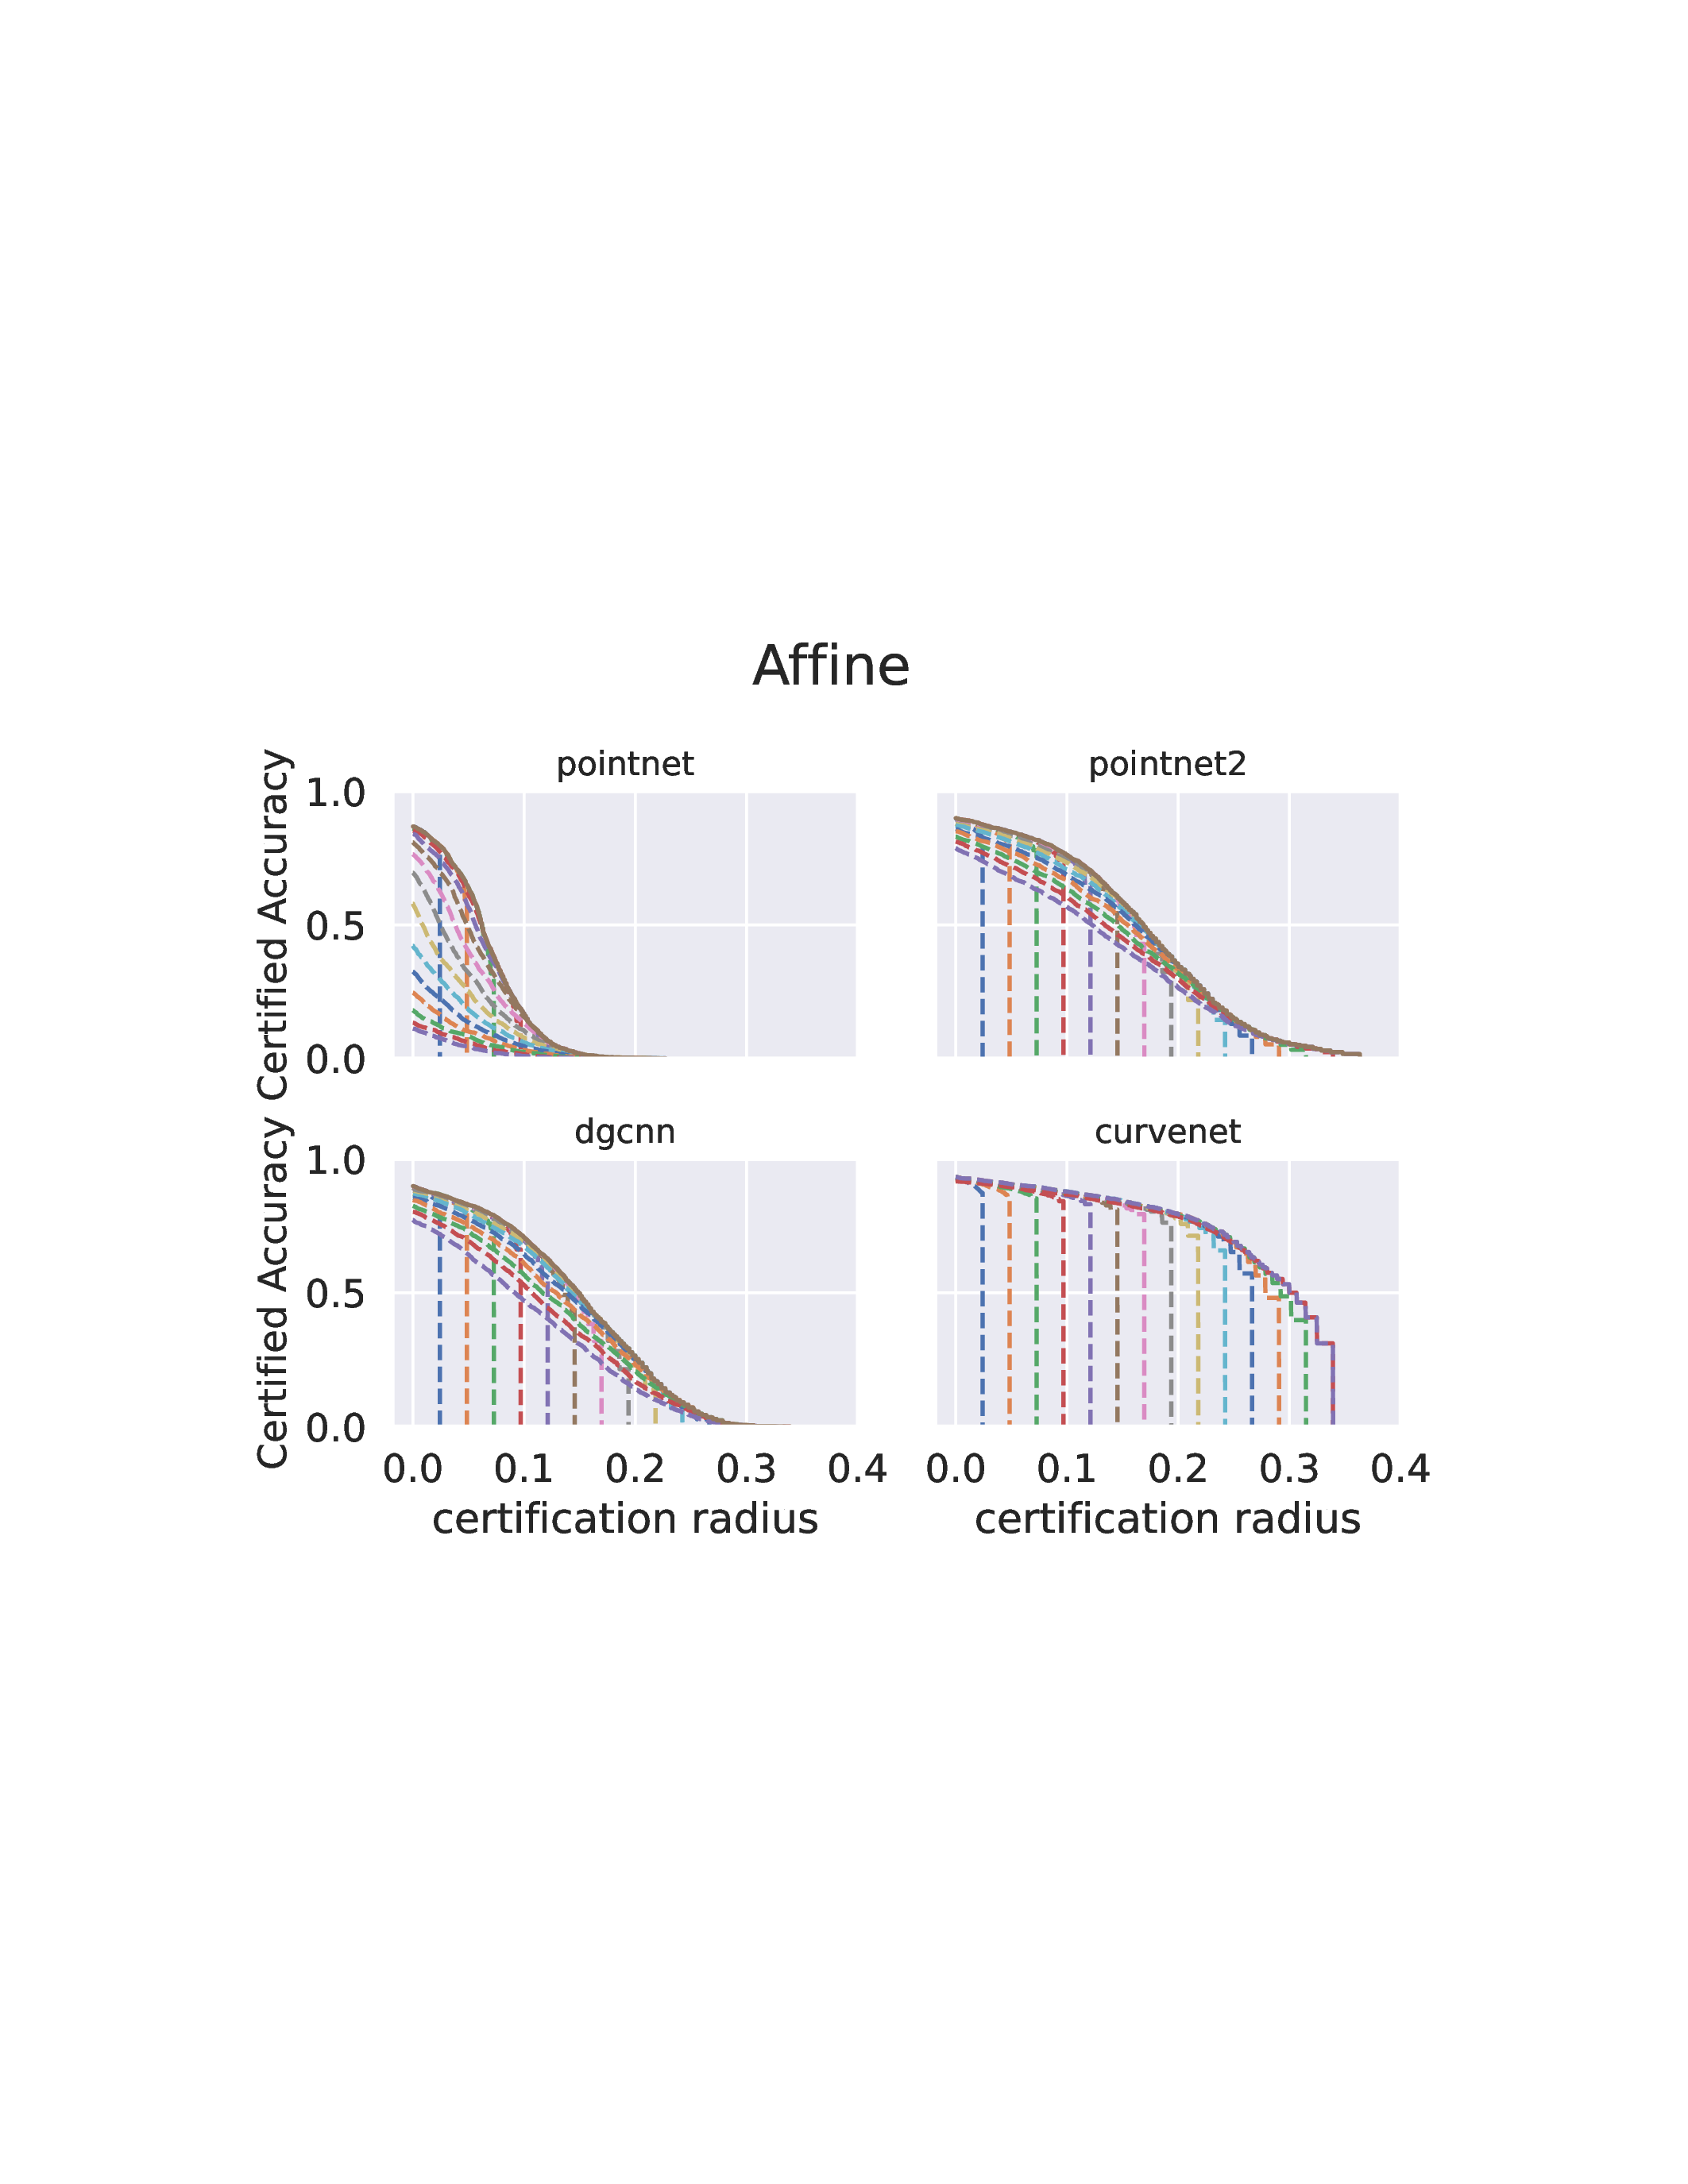}
    \includegraphics[width=0.45\linewidth,trim=0 0 0 1.5cm, clip]{images/SigmaExplicitResults/ScanObjectNN/Affine.eps}\\
    \includegraphics[width=0.80\linewidth,trim=0 0 0 1.5cm, clip]{images/SigmaExplicitResults/Legends/AffineLegend.png}\\
    \caption{Affine}
    \label{fig:SuppScanObjectNN}
\end{figure*}

\begin{figure*}[h]
    \centering
    \includegraphics[width=0.45\linewidth,trim=0 0 0 1.5cm, clip]{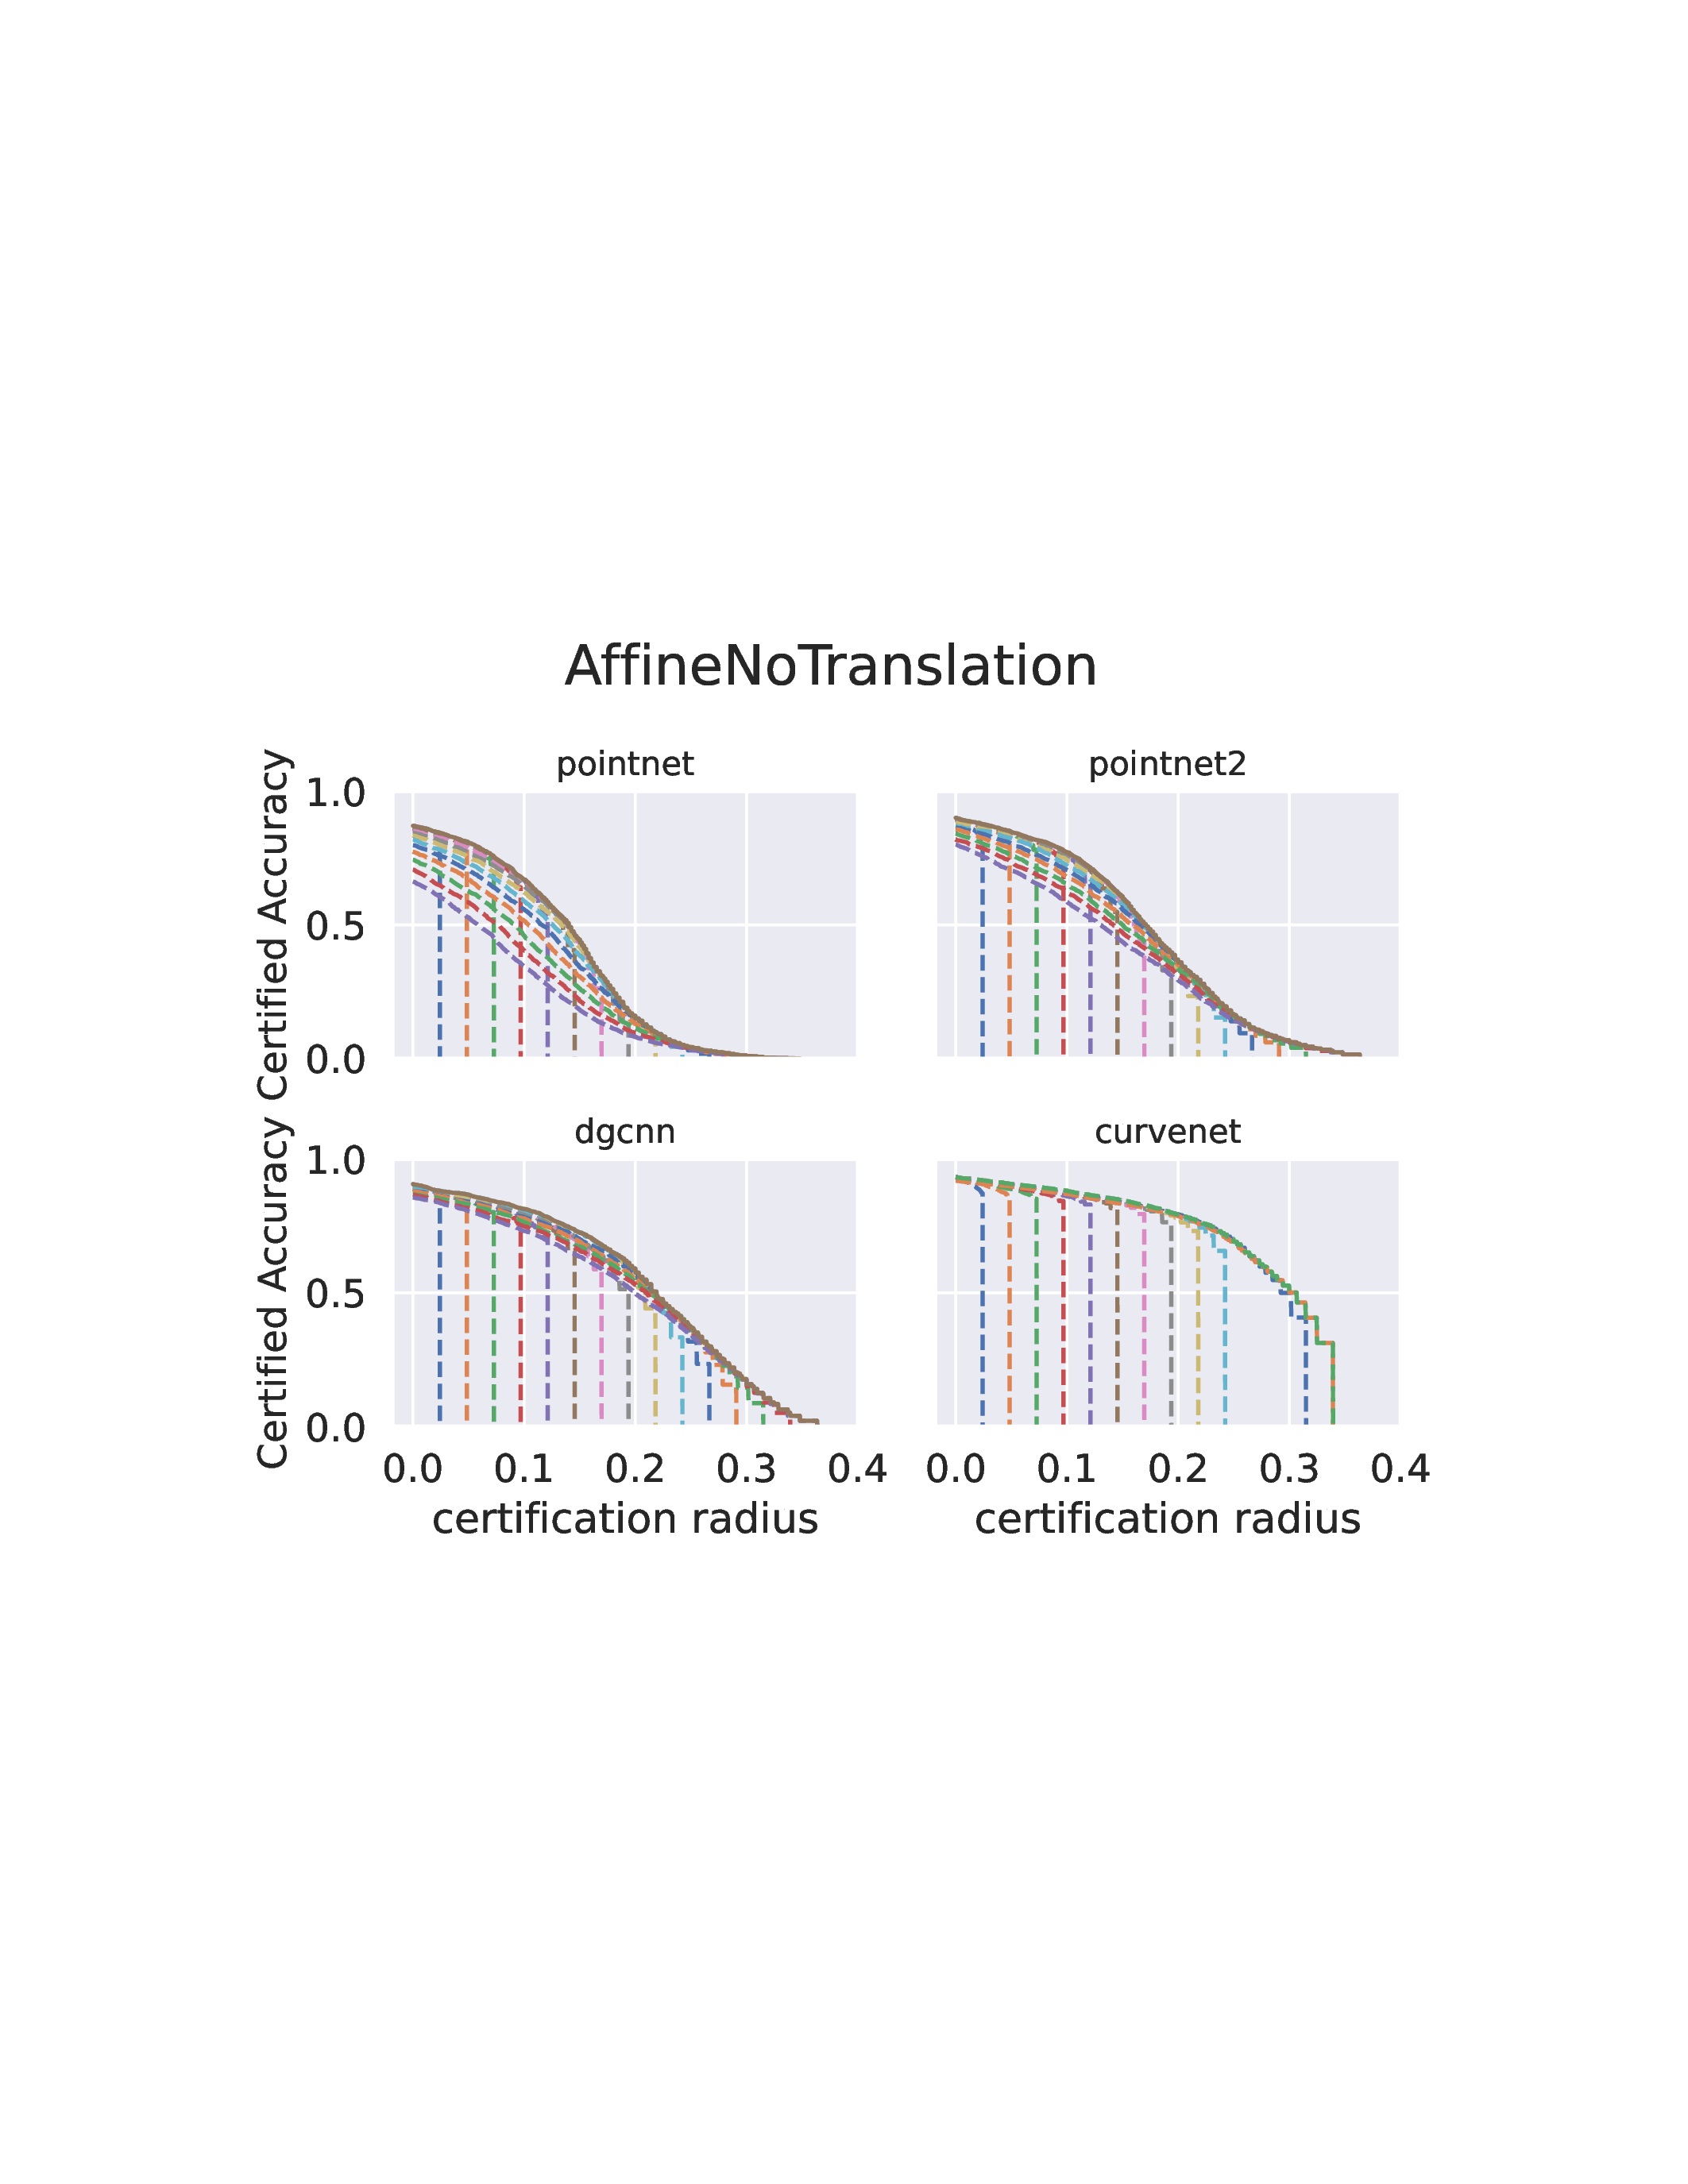}
    \includegraphics[width=0.45\linewidth,trim=0 0 0 1.5cm, clip]{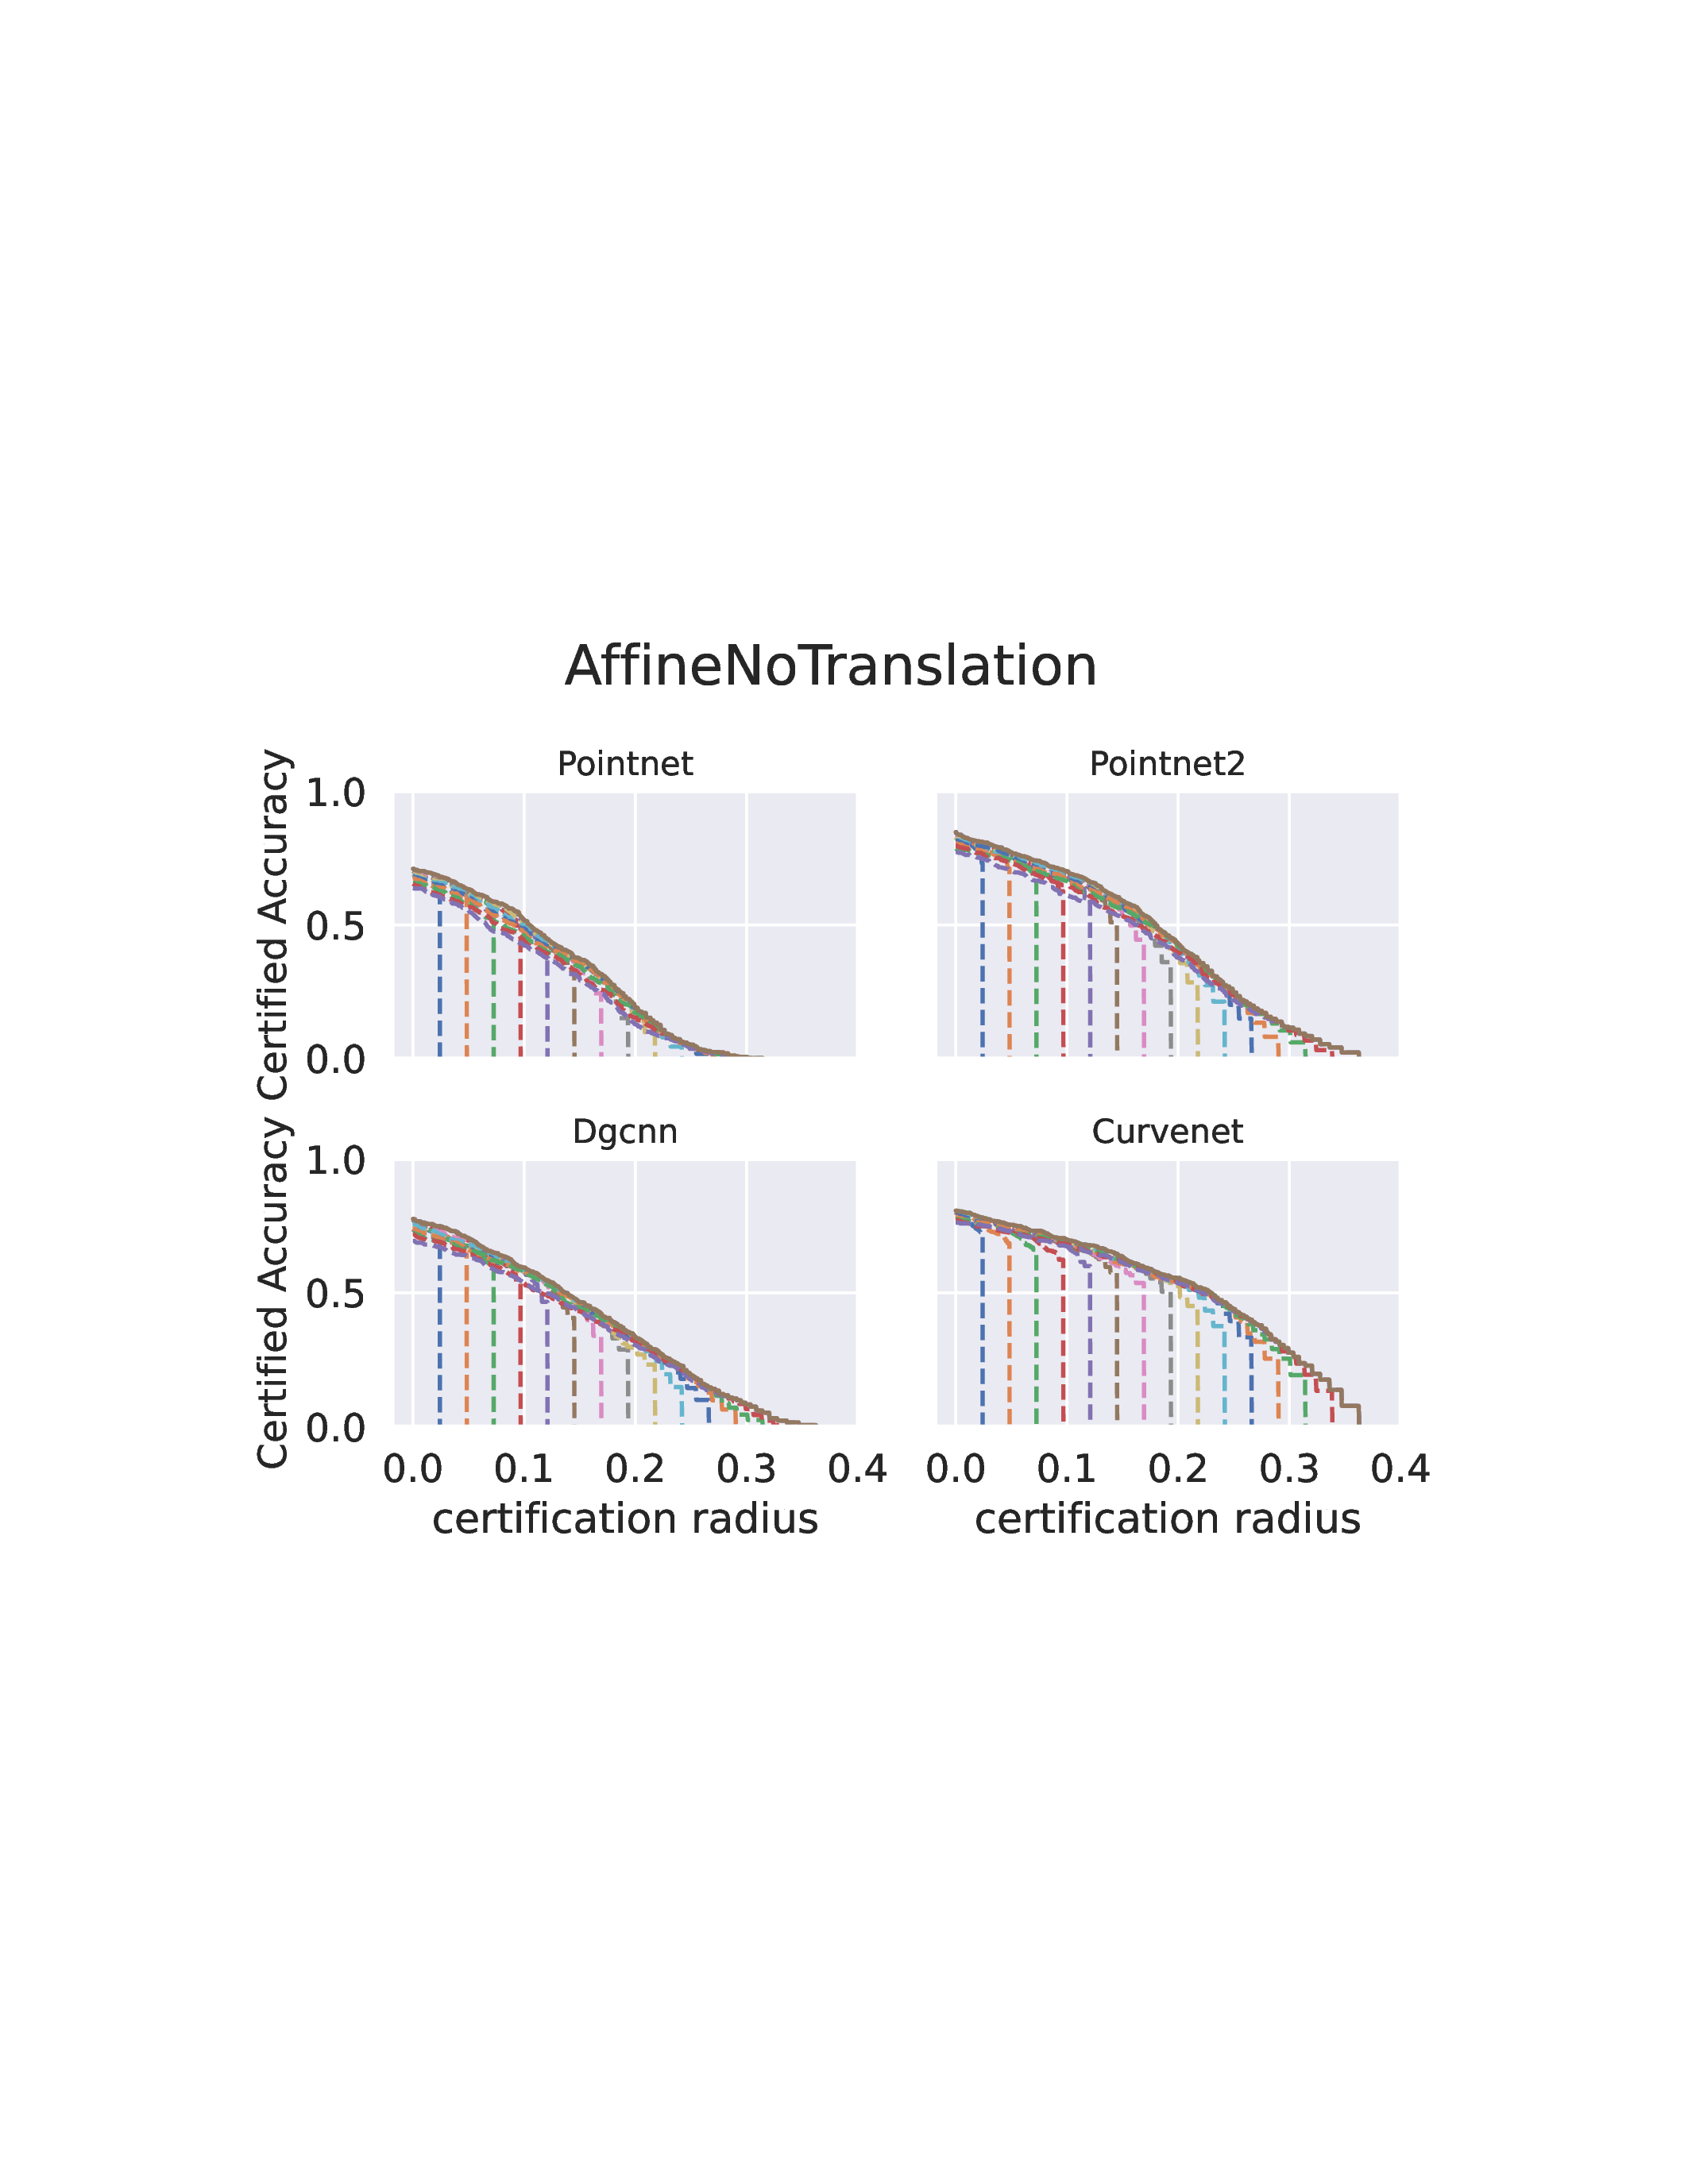}\\
    \includegraphics[width=0.80\linewidth,trim=0 0 0 1.5cm, clip]{images/SigmaExplicitResults/Legends/AffineNoTranslationLegend.png}\\
    \caption{Affine}
    \label{fig:SuppScanObjectNN}
\end{figure*}

\begin{figure*}[h]
    \centering
    \includegraphics[width=0.45\linewidth,trim=0 0 0 1.5cm, clip]{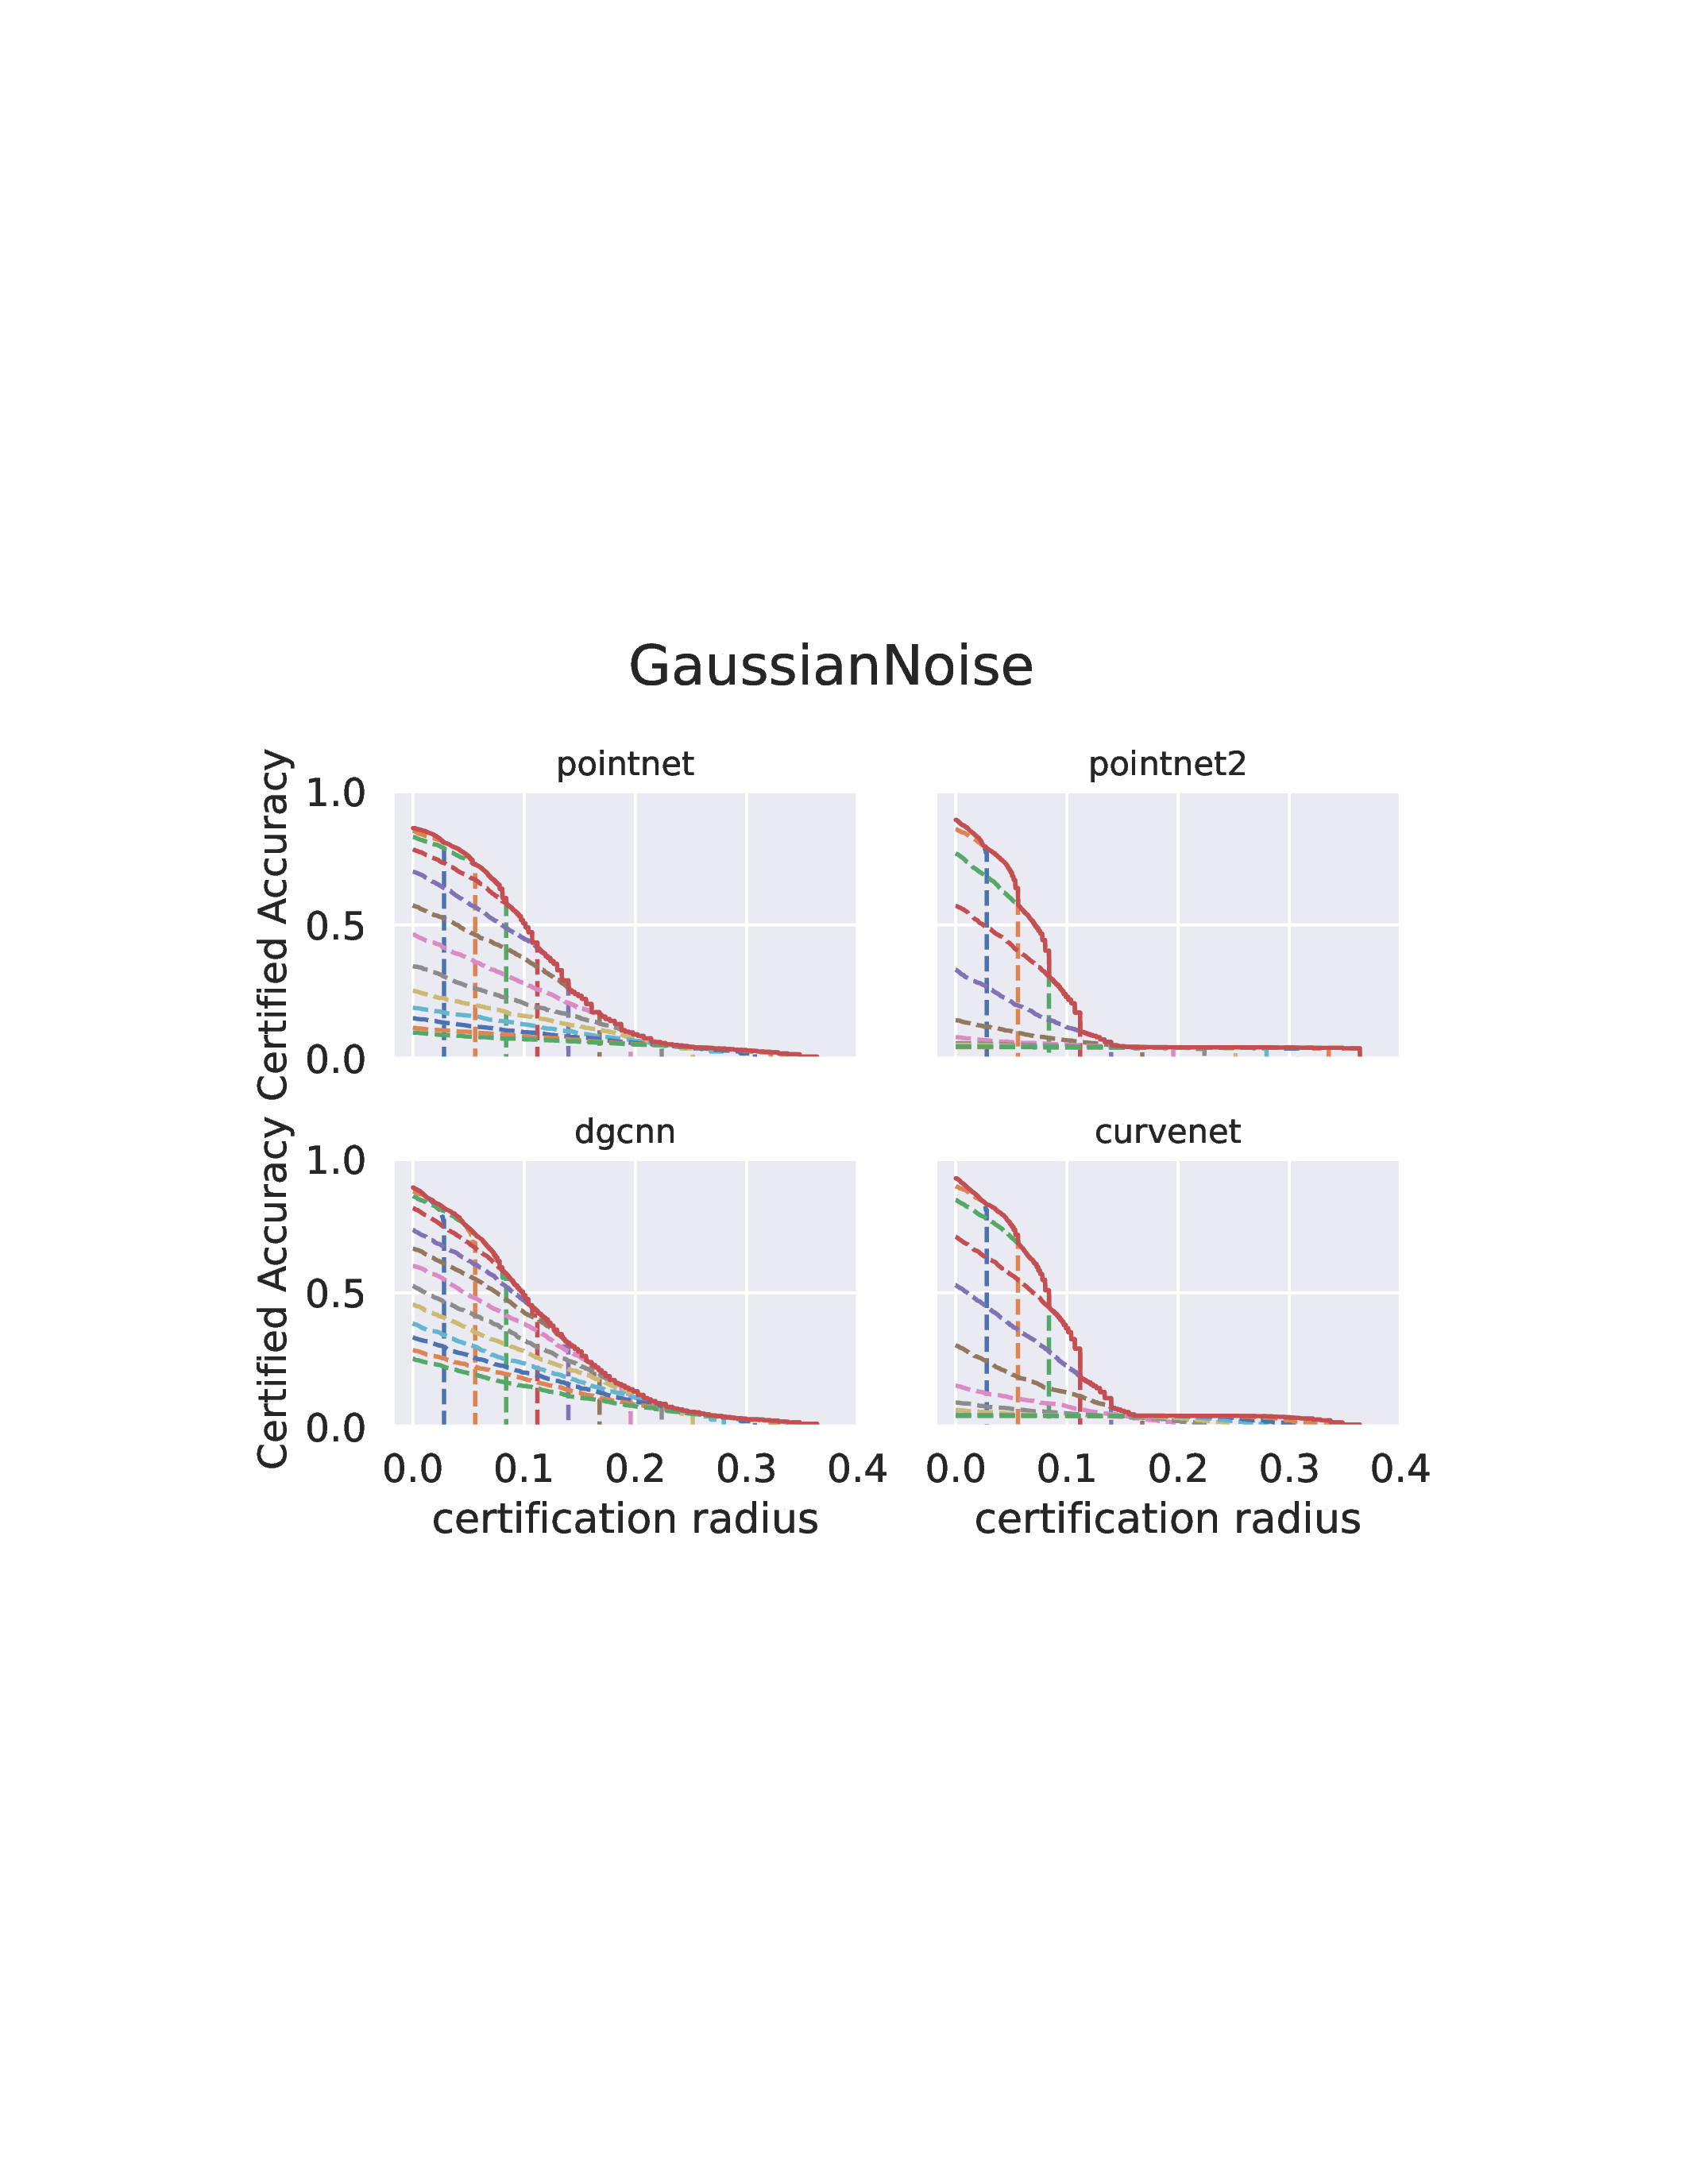}
    \includegraphics[width=0.45\linewidth,trim=0 0 0 1.5cm, clip]{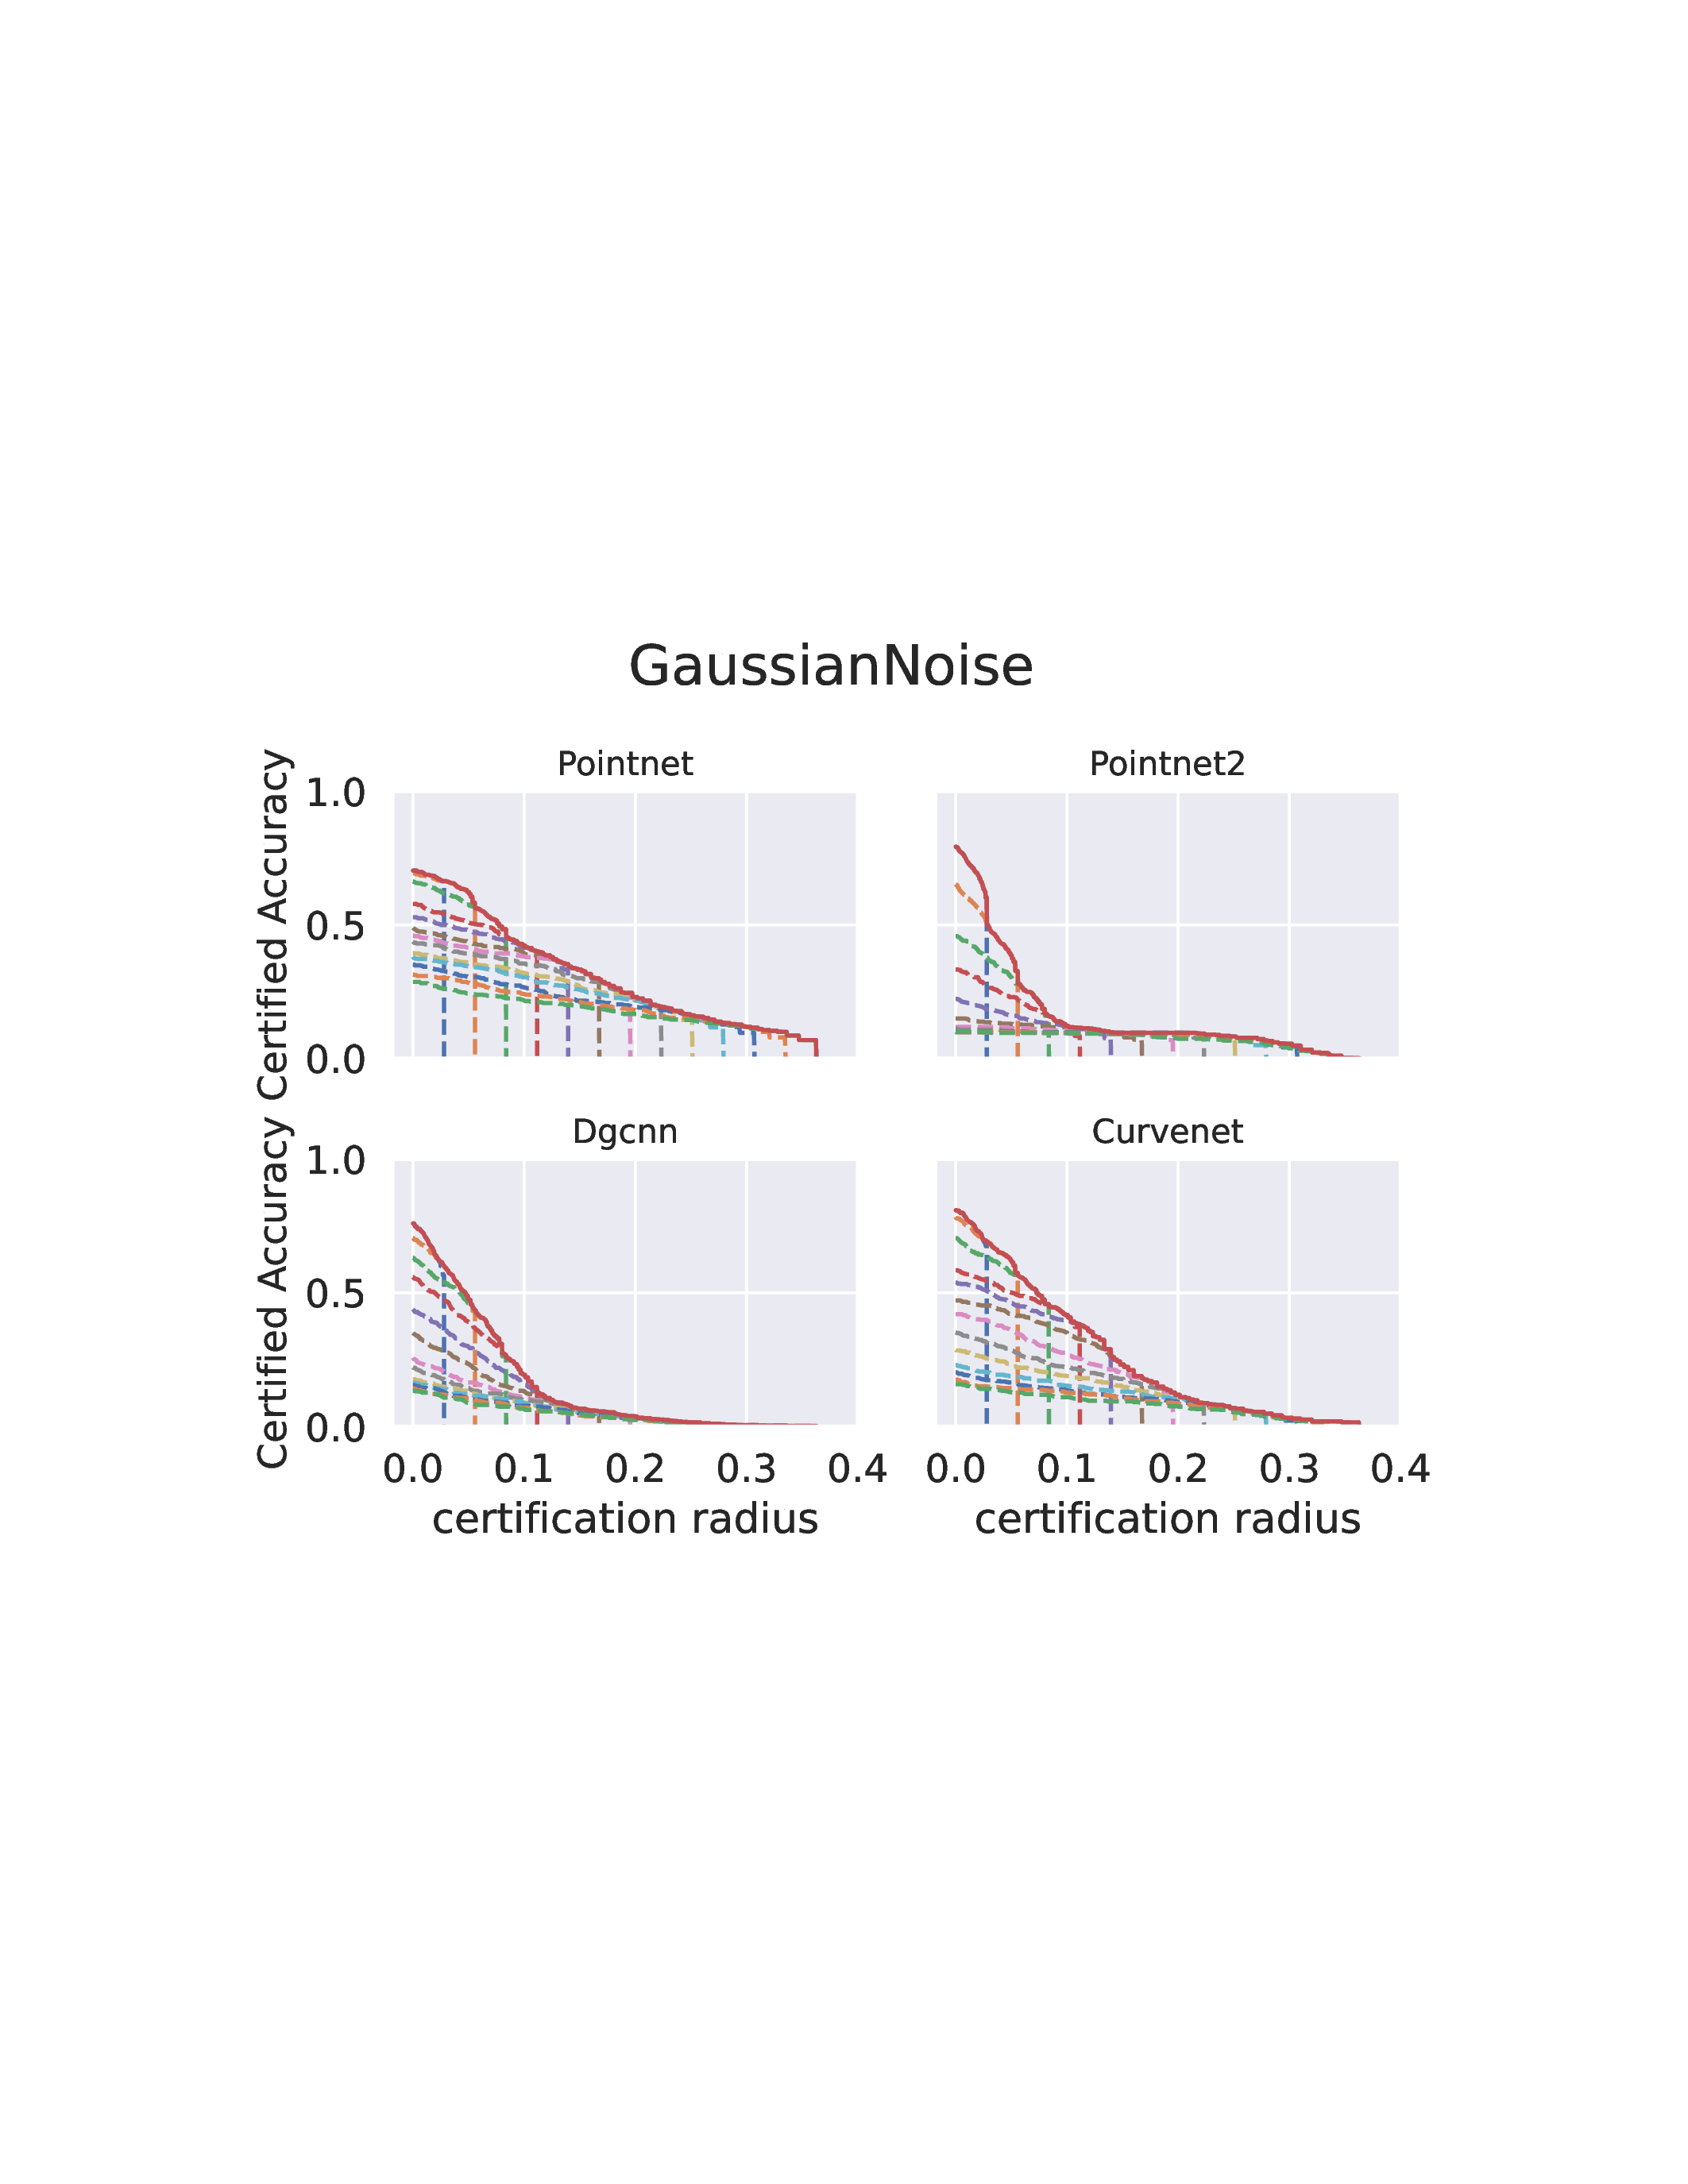}\\
    \includegraphics[width=0.80\linewidth,trim=0 0 0 1.5cm, clip]{images/SigmaExplicitResults/Legends/GaussianNoiseLegend.png}\\
    \caption{Affine}
    \label{fig:SuppScanObjectNN}
\end{figure*}

% \begin{figure*}[h]
%     \centering
%     % \includegraphics[width=0.45\linewidth]{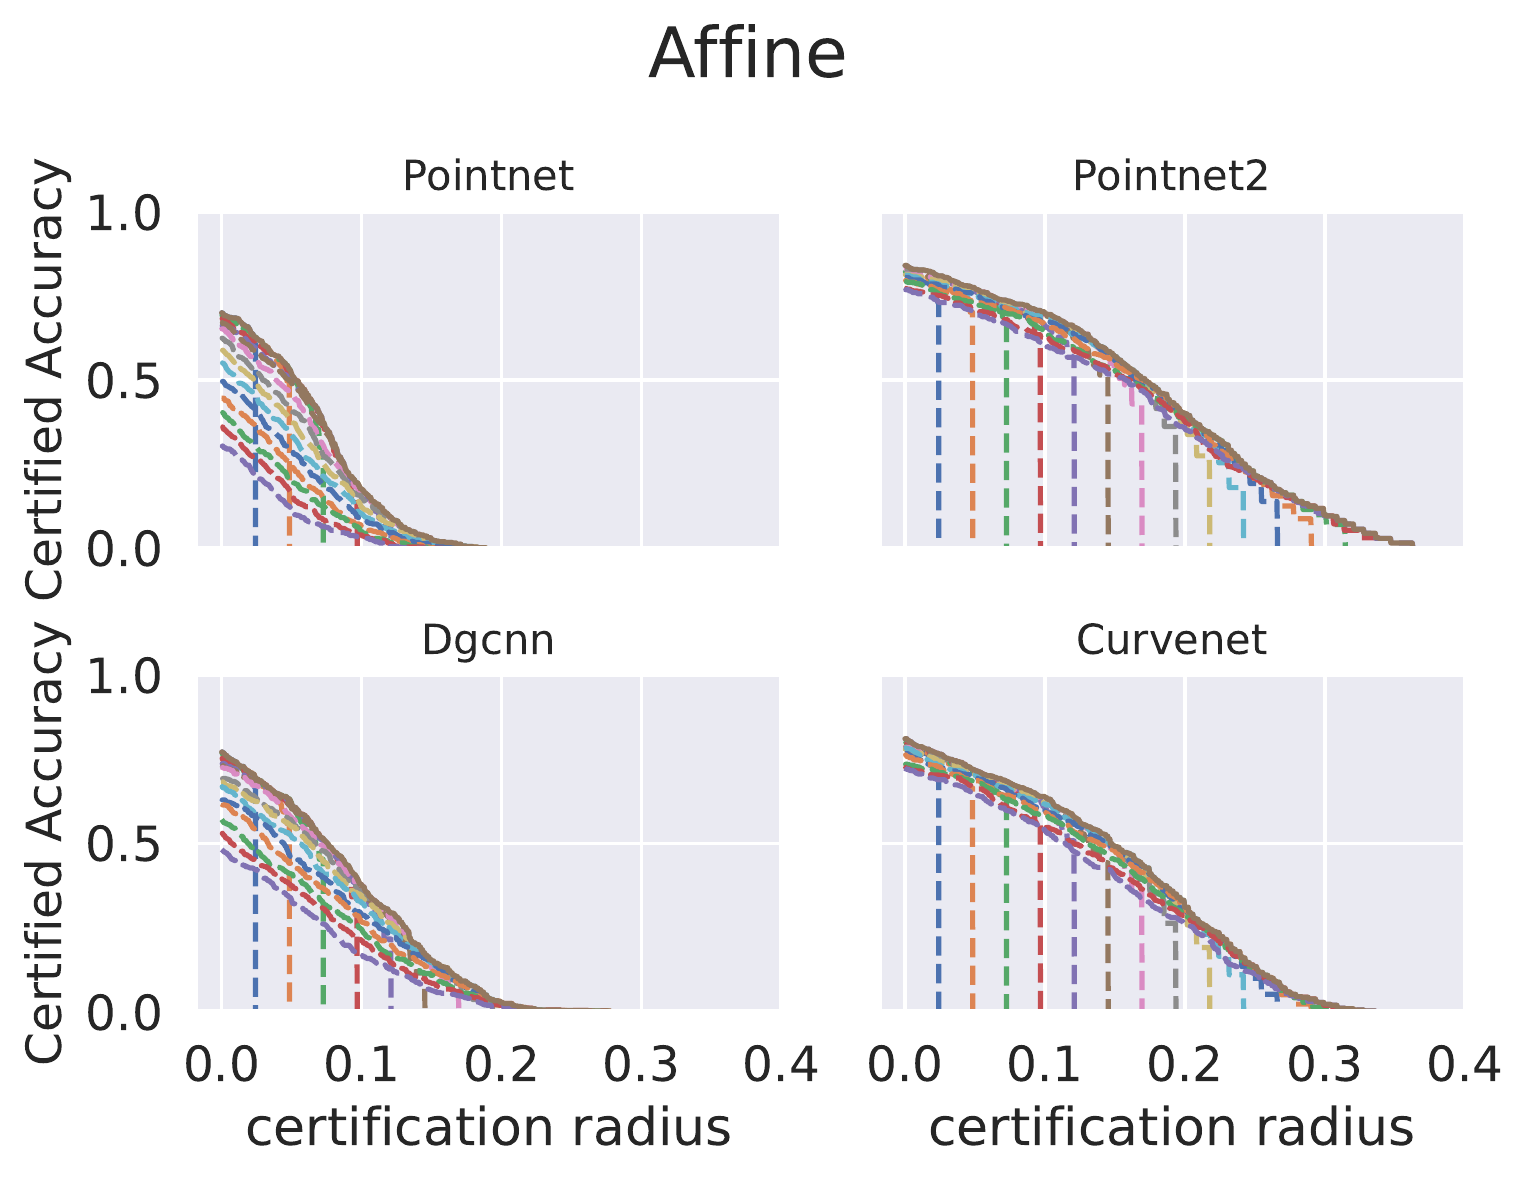}
%     % \includegraphics[width=0.45\linewidth]{images/SigmaExplicitResults/ScanObjectNN/AffineNoTranslation.pdf}
%     % \includegraphics[width=0.45\linewidth]{images/SigmaExplicitResults/ScanObjectNN/GaussianNoise.pdf}\\
%     % \includegraphics[width=0.45\linewidth]{images/SigmaExplicitResults/ScanObjectNN/Rotation.pdf}\\
%     % \includegraphics[width=0.45\linewidth]{images/SigmaExplicitResults/ScanObjectNN/RotationXZ.pdf}
%     % \includegraphics[width=0.45\linewidth]{images/SigmaExplicitResults/ScanObjectNN/RotationZ.pdf}\\
%     % \includegraphics[width=0.45\linewidth]{images/SigmaExplicitResults/ScanObjectNN/Shearing.pdf}
%     % \includegraphics[width=0.45\linewidth]{images/SigmaExplicitResults/ScanObjectNN/Tapering.pdf} \\
%     % \includegraphics[width=0.45\linewidth]{images/SigmaExplicitResults/ScanObjectNN/Translation.pdf}
%     % \includegraphics[width=0.45\linewidth]{images/SigmaExplicitResults/ScanObjectNN/Twisting.pdf}
%     \caption{Certified Accuracy against 10 deformations for PointNet, PointNet++, DGCNN and CurveNet with the respective $\sigma$ values explored}
%     \label{fig:SuppScanObjectNN}
% \end{figure*}
