# Supplementary material for: 3DeformRS: Certifying Spatial Deformations on Point Clouds
Source: arXiv:2204.05687 source file (2022-04-12)
Supplement: Supplementary file 3 [file supp_ModelNet40_curves_with_sigmas.tex]

\begin{figure}[h]
    \centering
    \includegraphics[width=\linewidth]{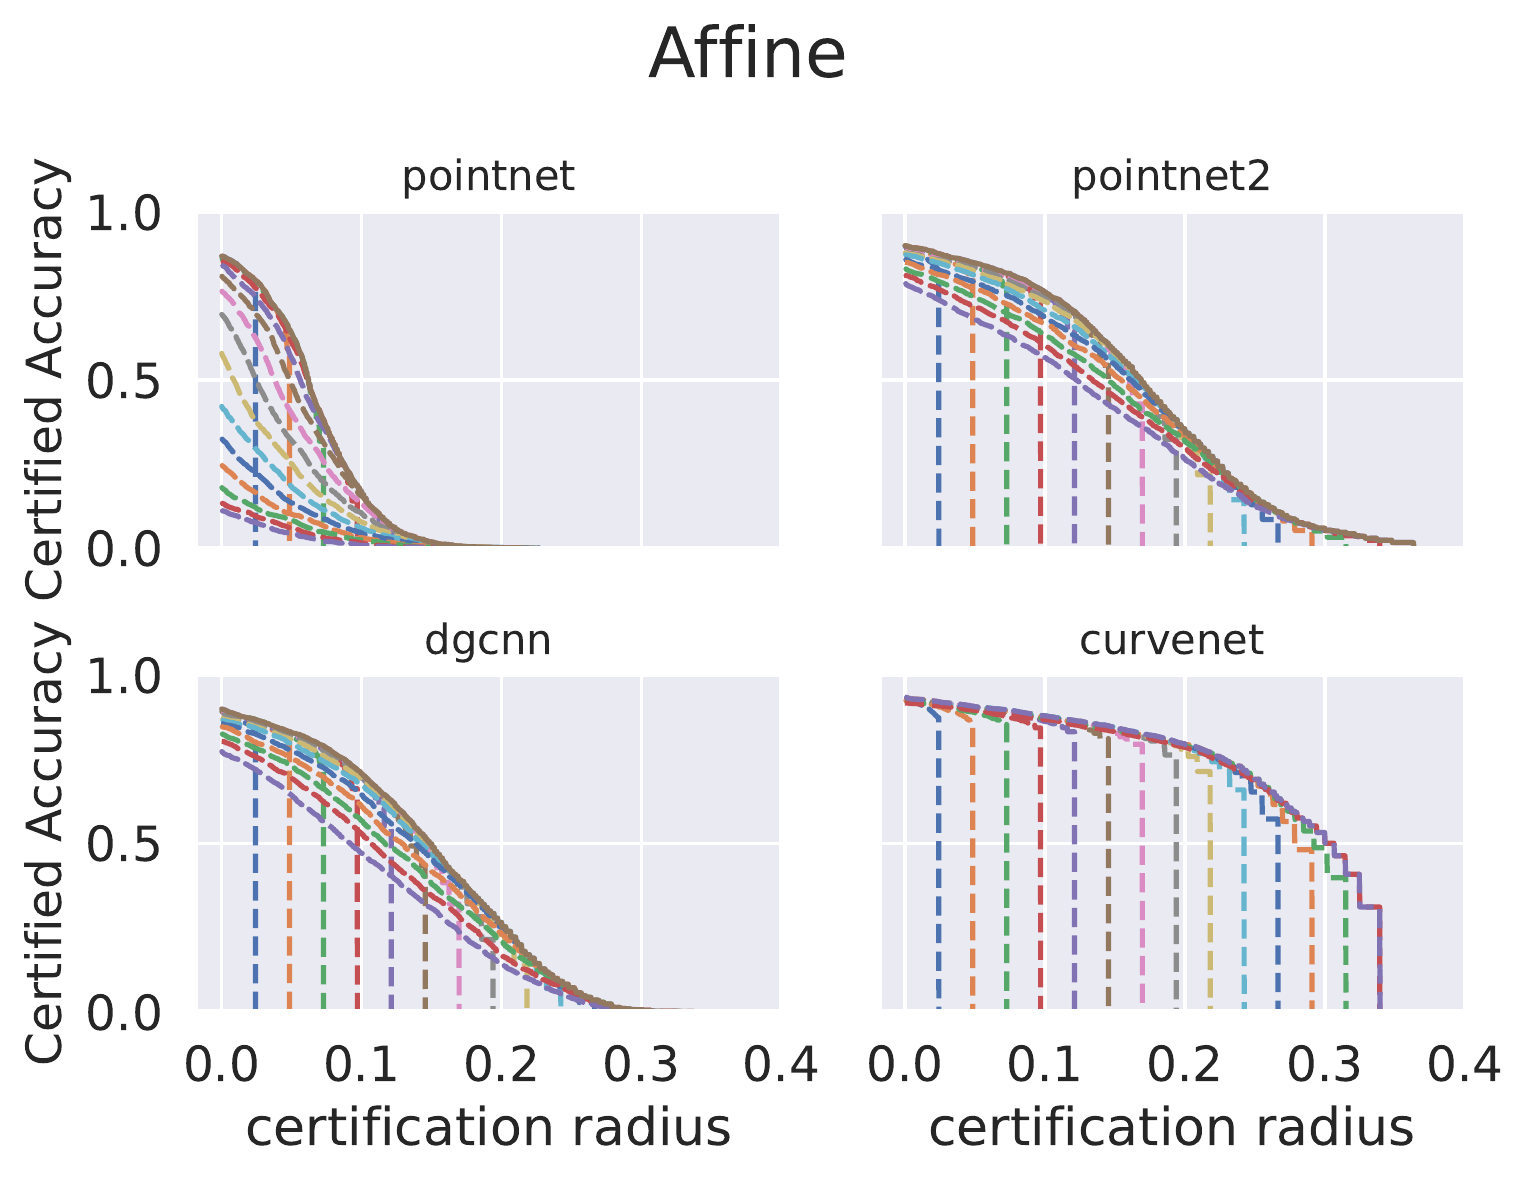}
    \includegraphics[width=\linewidth]{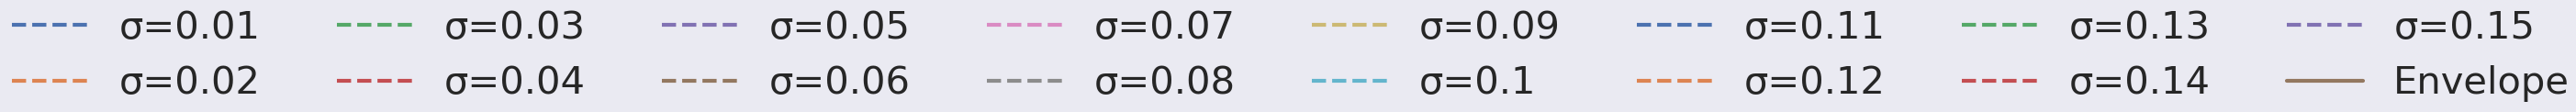}
    \caption{Certified Accuracy against Affine deformations for PointNet, PointNet++, DGCNN and CurveNet with the respective $\sigma$ values explored}
    \label{fig:SuppModelNet40Affine}
\end{figure}

\begin{figure}[h]
    \centering
    \includegraphics[width=\linewidth]{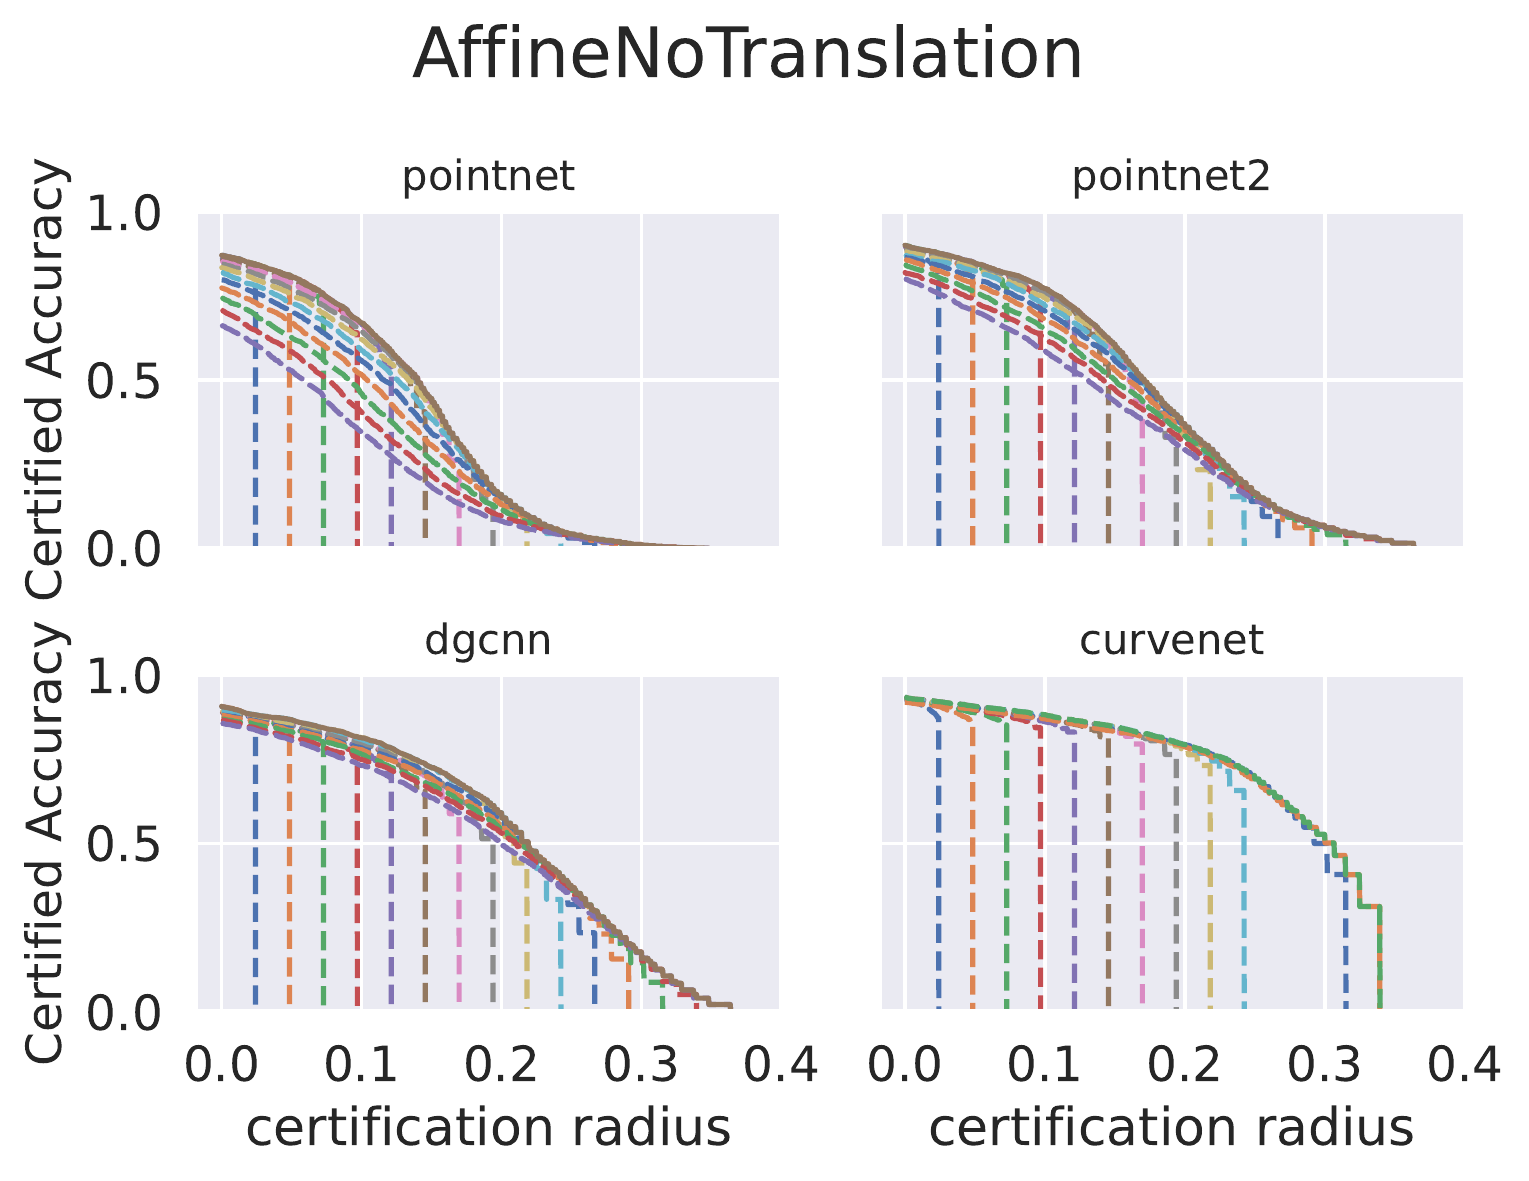}
    \includegraphics[width=\linewidth]{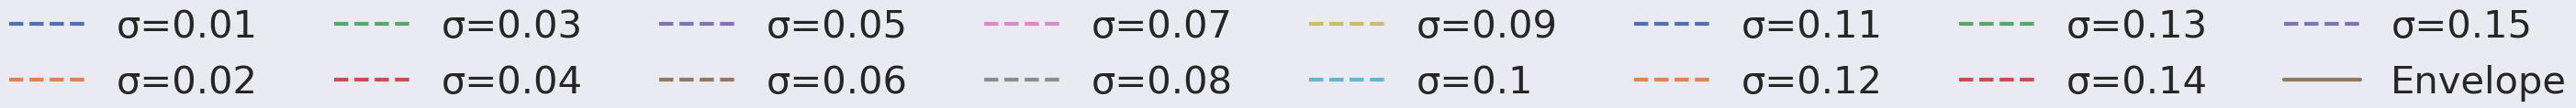}
    \caption{Certified Accuracy against Affine (NT) deformations for PointNet, PointNet++, DGCNN and CurveNet with the respective $\sigma$ values explored}
    \label{fig:SuppModelNet40AffineNT}
\end{figure}

\begin{figure}[h]
    \centering
    \includegraphics[width=\linewidth]{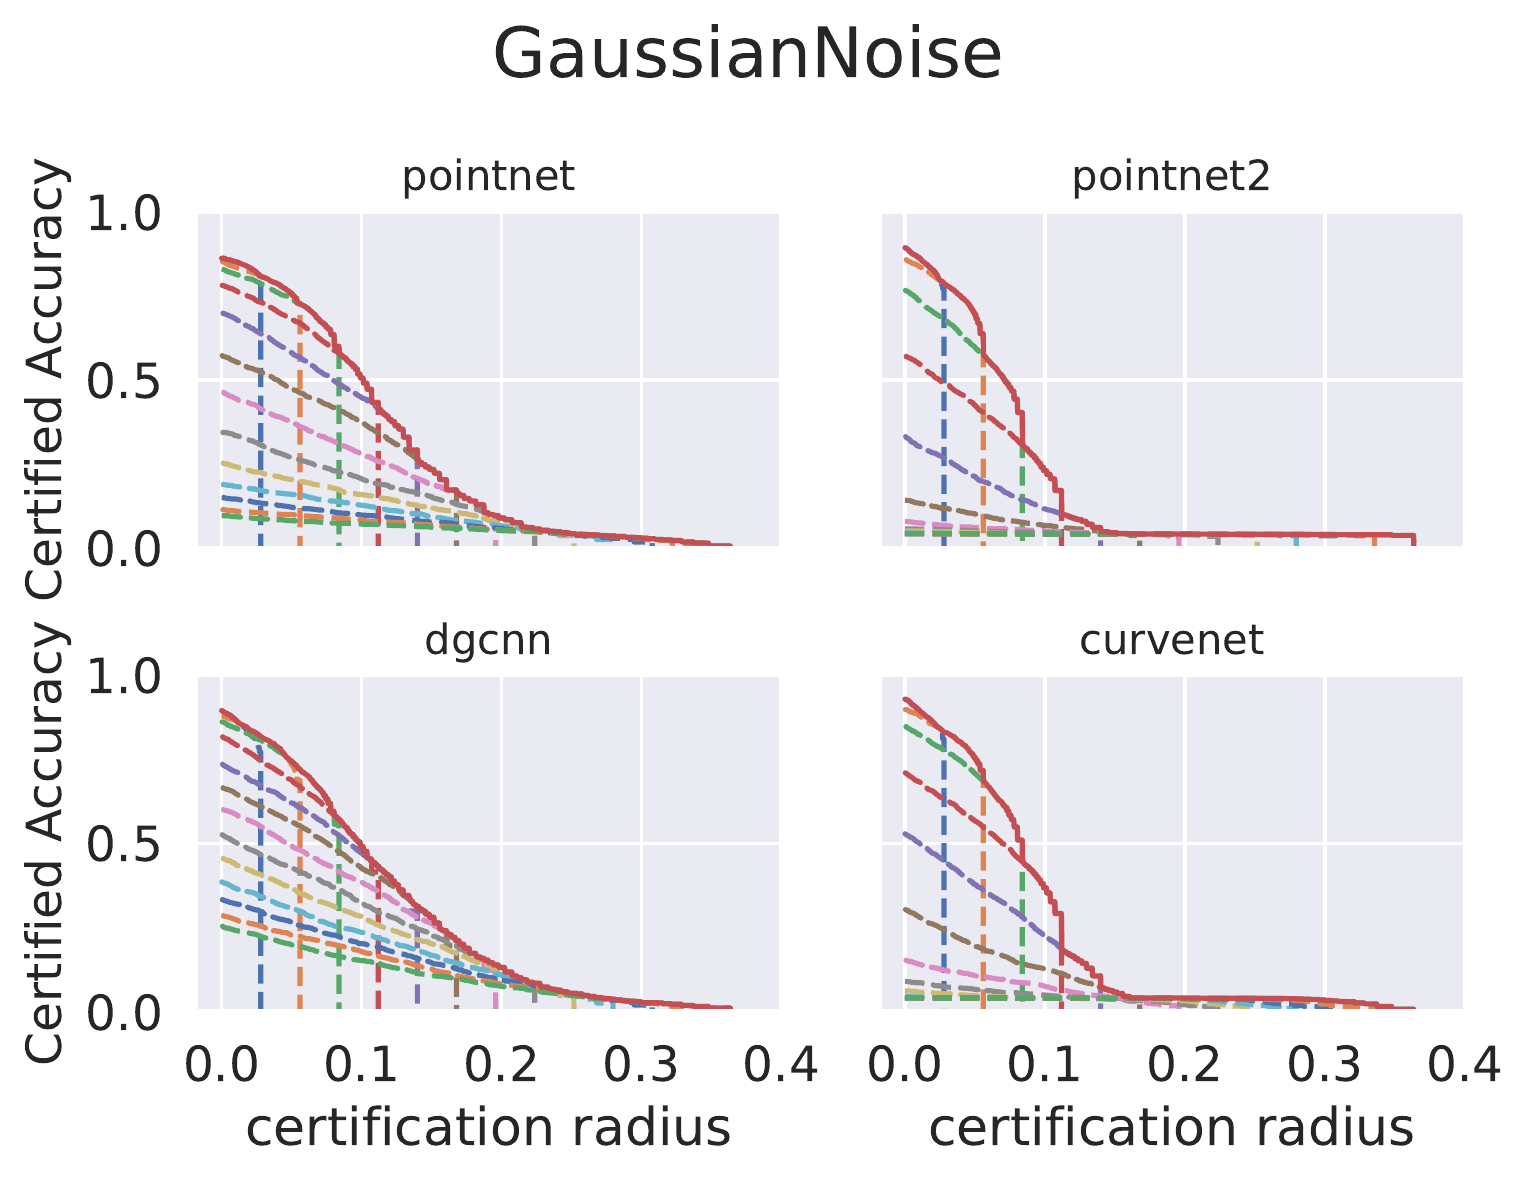}
    \includegraphics[width=\linewidth]{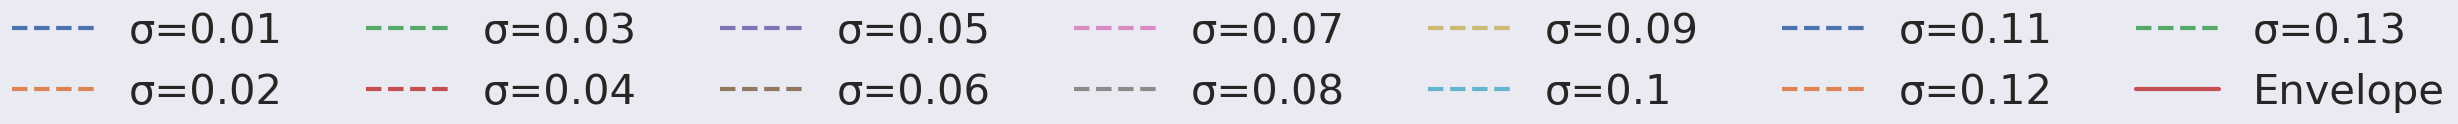}
    \caption{Certified Accuracy against Gaussian Noise deformations for PointNet, PointNet++, DGCNN and CurveNet with the respective $\sigma$ values explored}
    \label{fig:SuppModelNet40GaussianNoise}
\end{figure}

\begin{figure}[h]
    \centering
    \includegraphics[width=\linewidth]{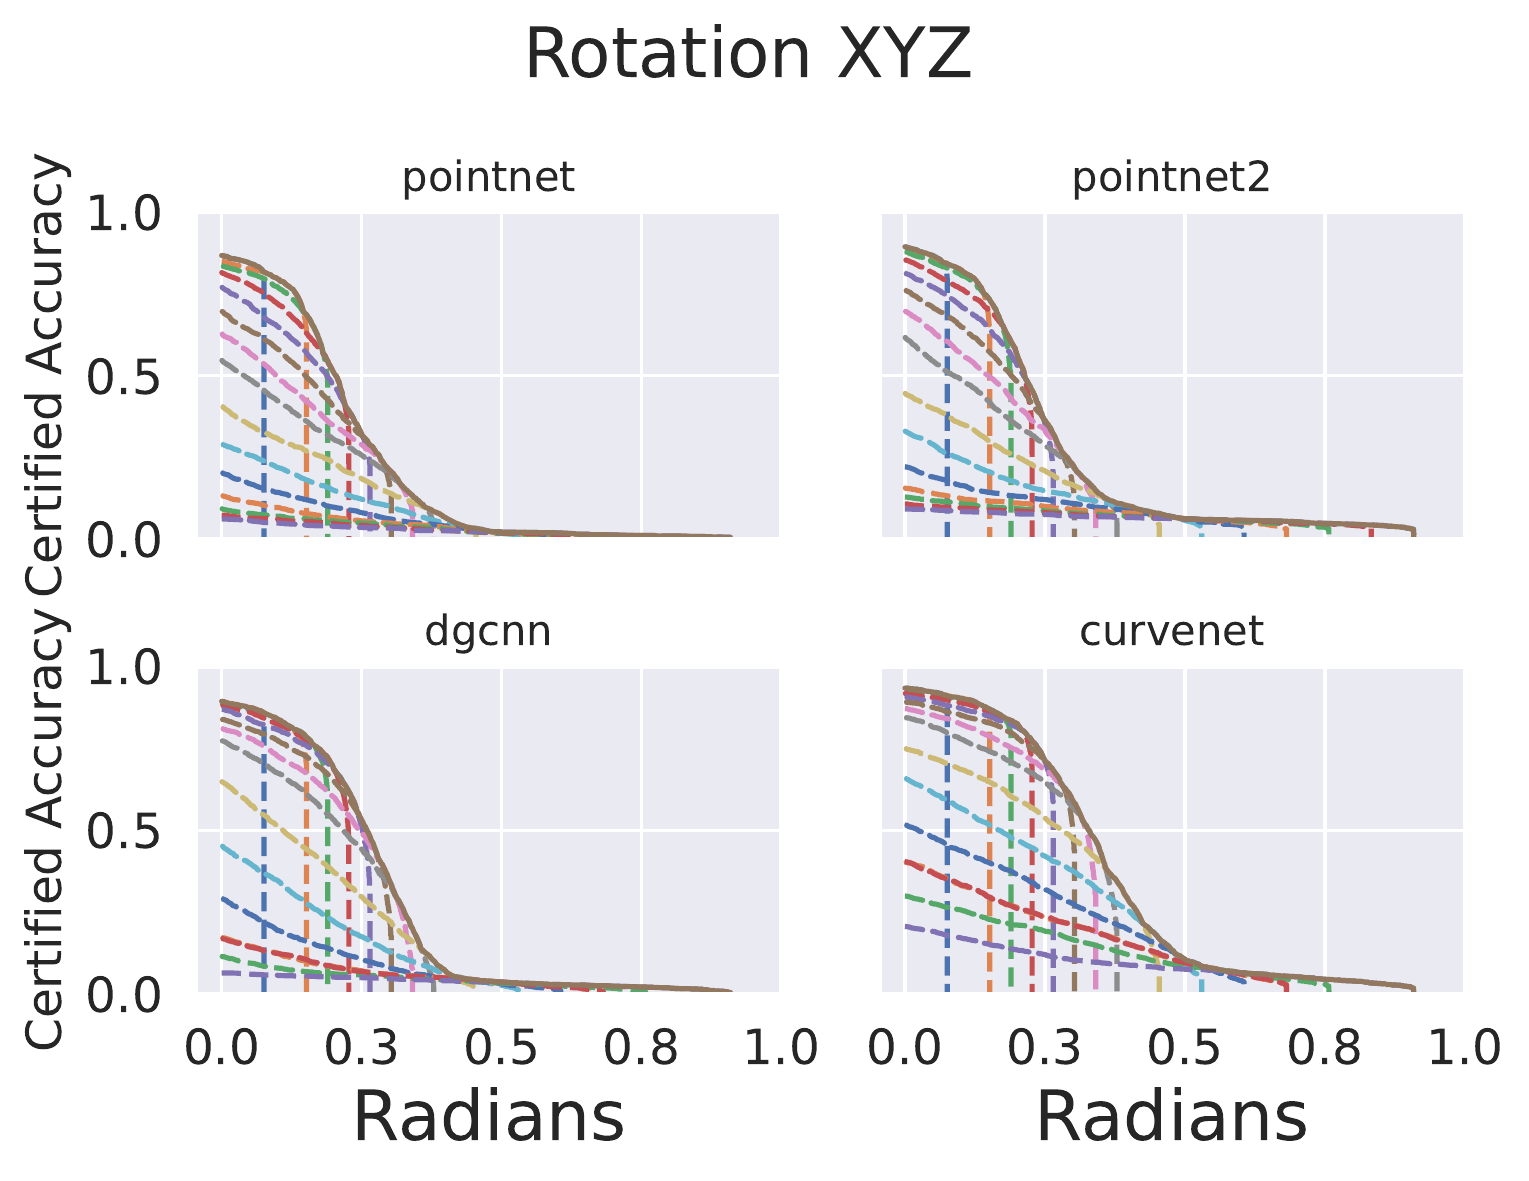}
    \includegraphics[width=\linewidth]{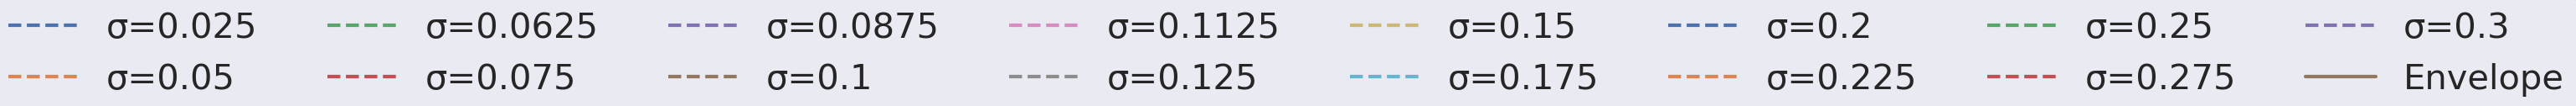}
    \caption{Certified Accuracy against Rotations XYZ deformations for PointNet, PointNet++, DGCNN and CurveNet with the respective $\sigma$ values explored}
    \label{fig:SuppModelNet40RotXYZ}
\end{figure}

\begin{figure}[h]
    \centering
    \includegraphics[width=\linewidth]{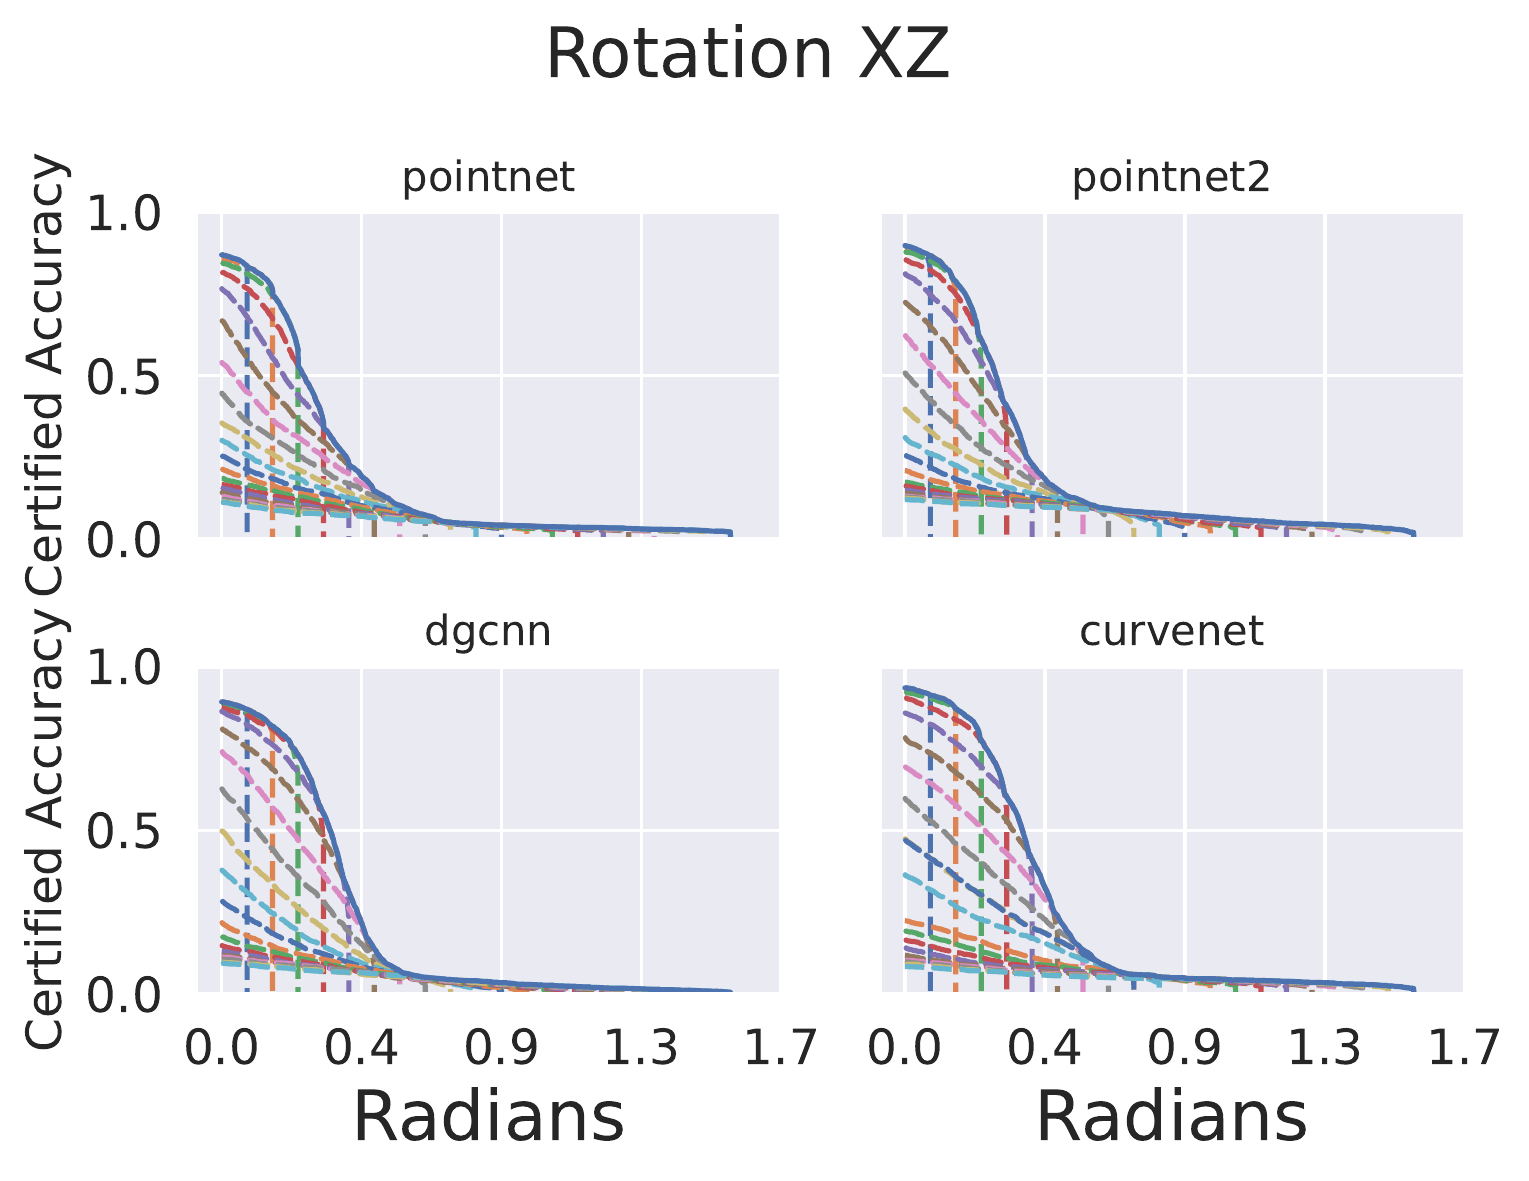}
    \includegraphics[width=\linewidth]{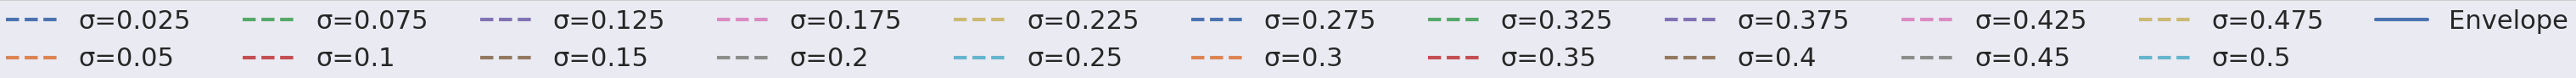}
    \caption{Certified Accuracy against Rotations XZ deformations for PointNet, PointNet++, DGCNN and CurveNet with the respective $\sigma$ values explored}
    \label{fig:SuppModelNet40RotXZ}
\end{figure}

\begin{figure}[h]
    \centering
    \includegraphics[width=\linewidth]{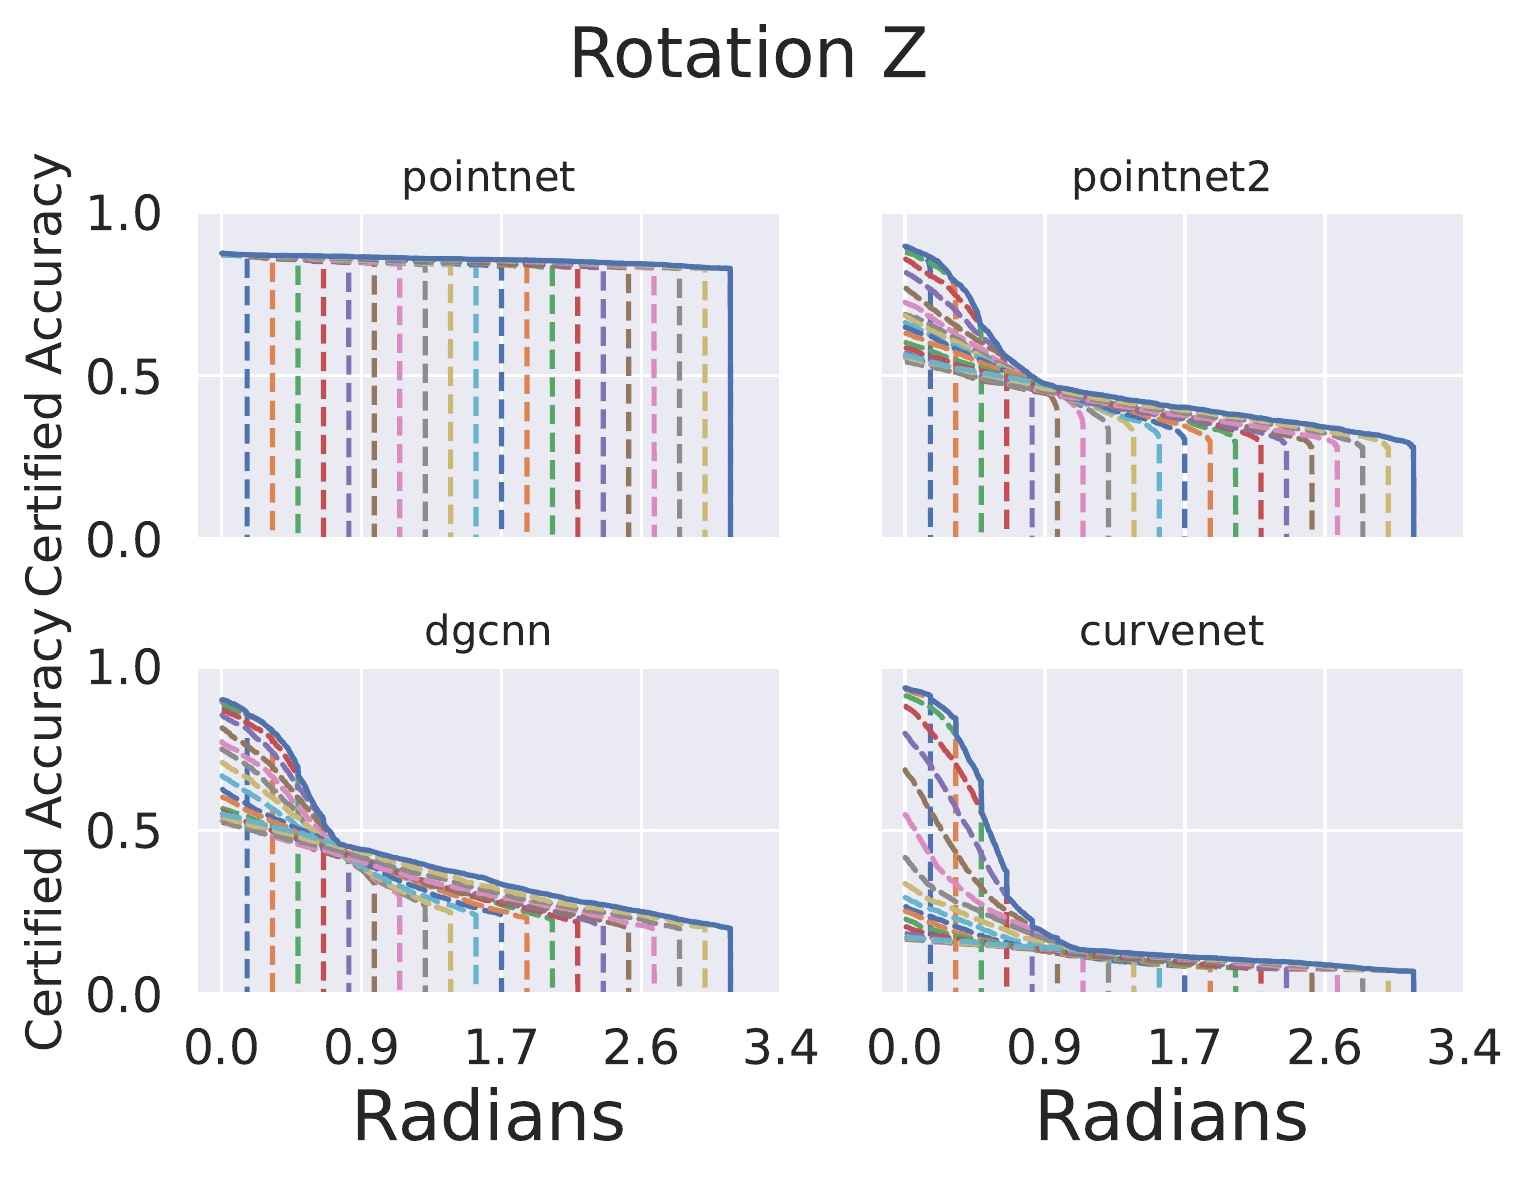}
    \includegraphics[width=\linewidth]{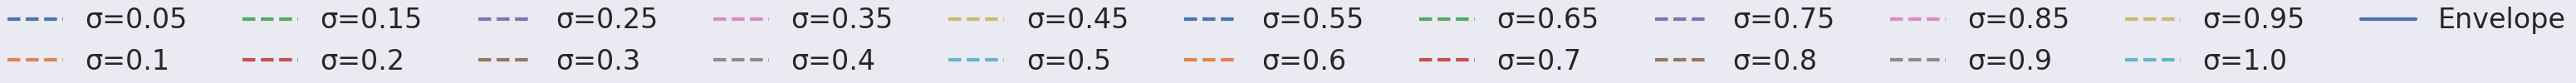}
    \caption{Certified Accuracy against Rotations XYZ deformations for PointNet, PointNet++, DGCNN and CurveNet with the respective $\sigma$ values explored}
    \label{fig:SuppModelNet40RotZ}
\end{figure}

\begin{figure}[h]
    \centering
    \includegraphics[width=\linewidth]{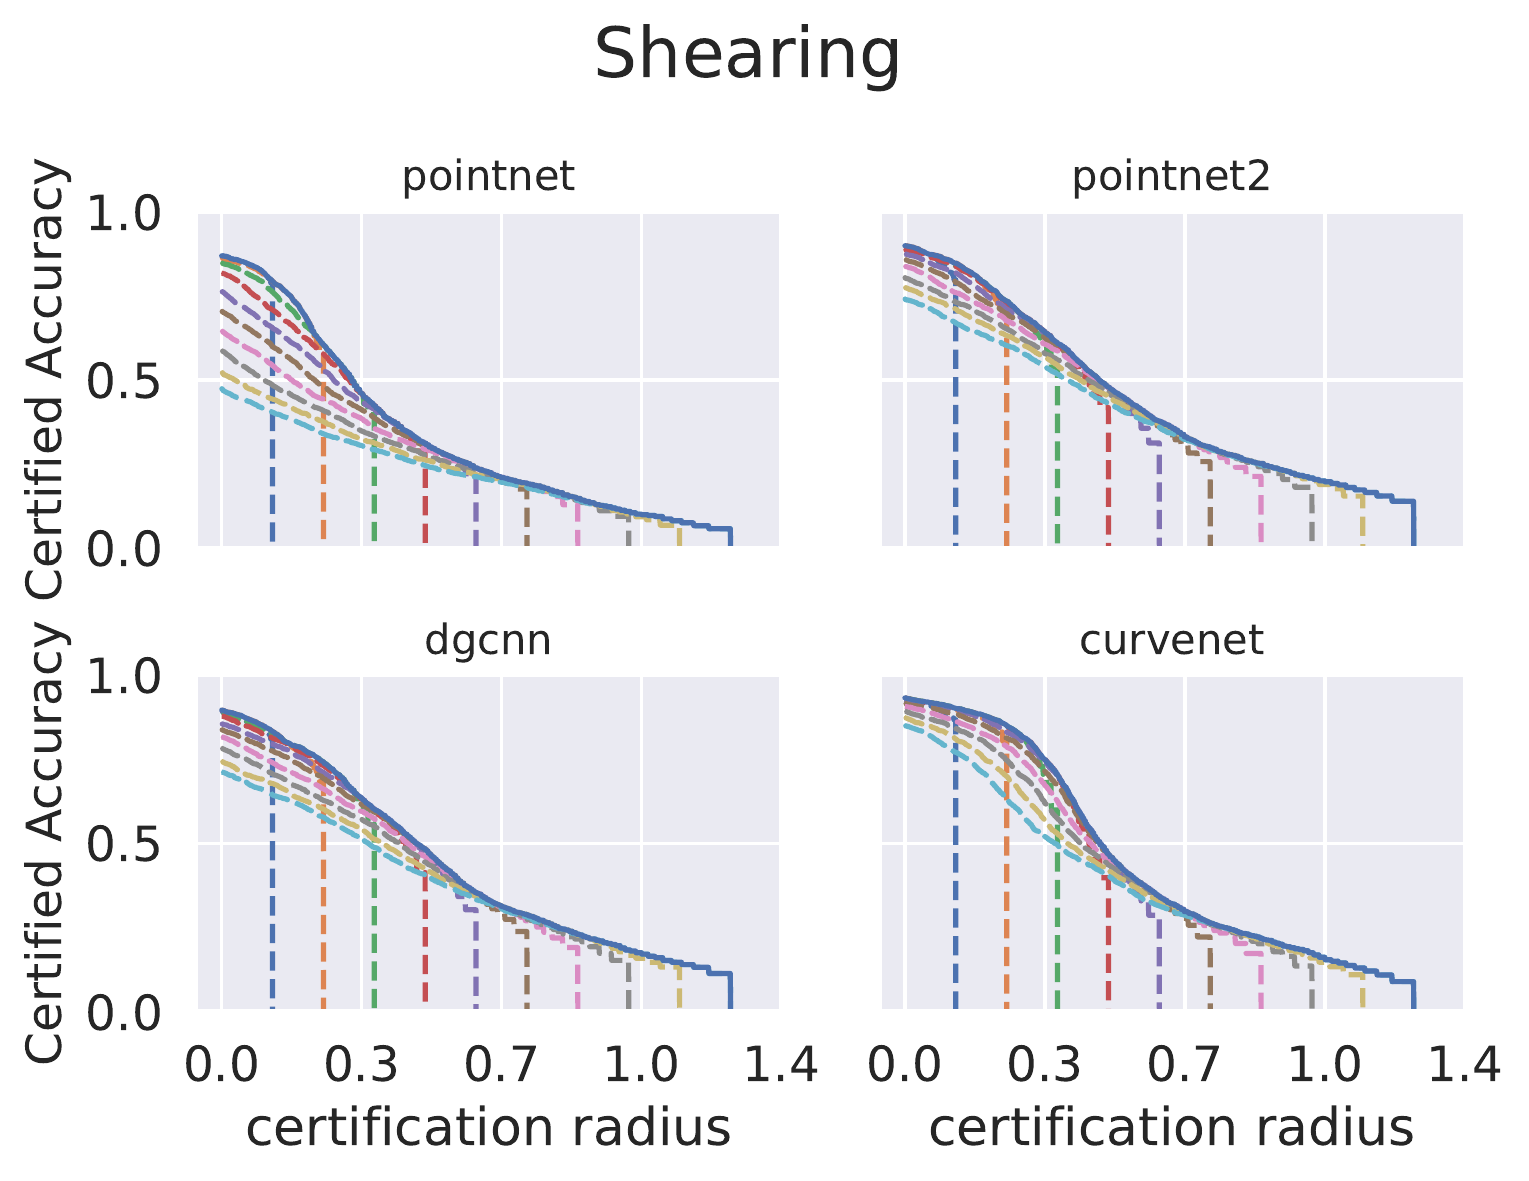}
    \includegraphics[width=\linewidth]{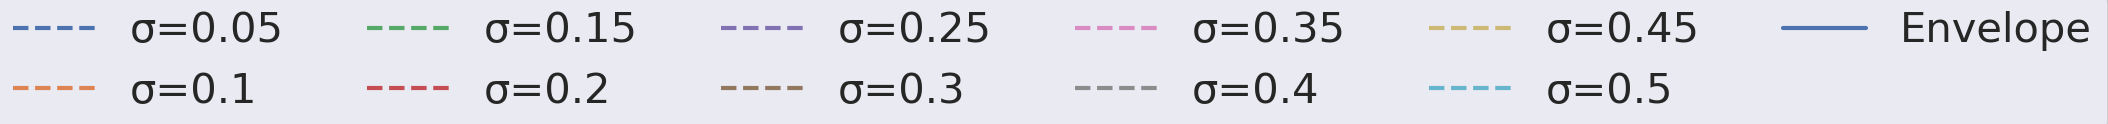}
    \caption{Certified Accuracy against Shearing deformations for PointNet, PointNet++, DGCNN and CurveNet with the respective $\sigma$ values explored}
    \label{fig:SuppModelNet40Shearing}
\end{figure}

\begin{figure}[h]
    \centering
    \includegraphics[width=\linewidth]{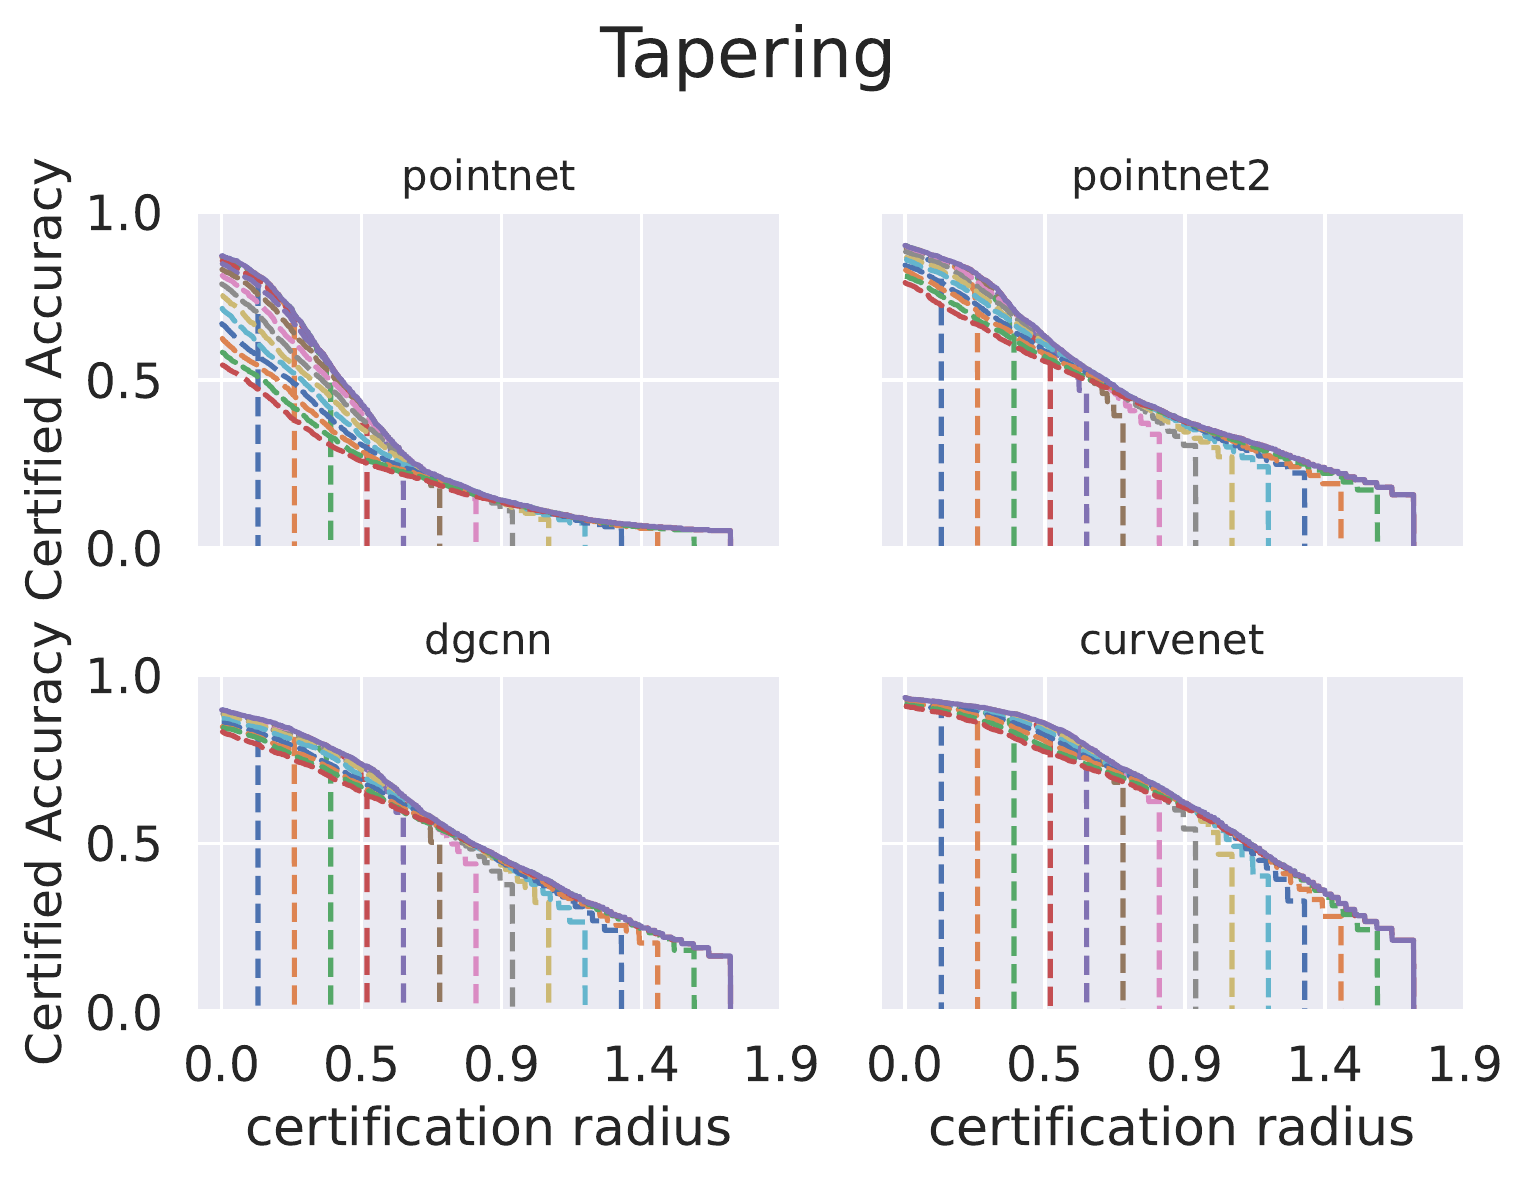}
    \includegraphics[width=\linewidth]{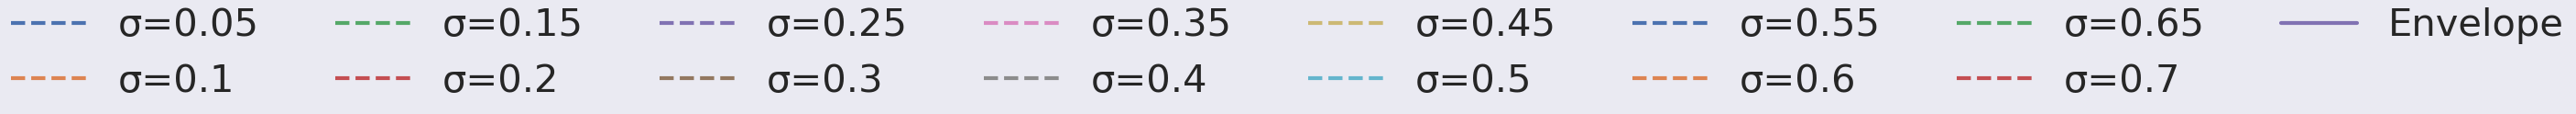}
    \caption{Certified Accuracy against Tapering deformations for PointNet, PointNet++, DGCNN and CurveNet with the respective $\sigma$ values explored}
    \label{fig:SuppModelNet40Tapering}
\end{figure}

\begin{figure}[h]
    \centering
    \includegraphics[width=\linewidth]{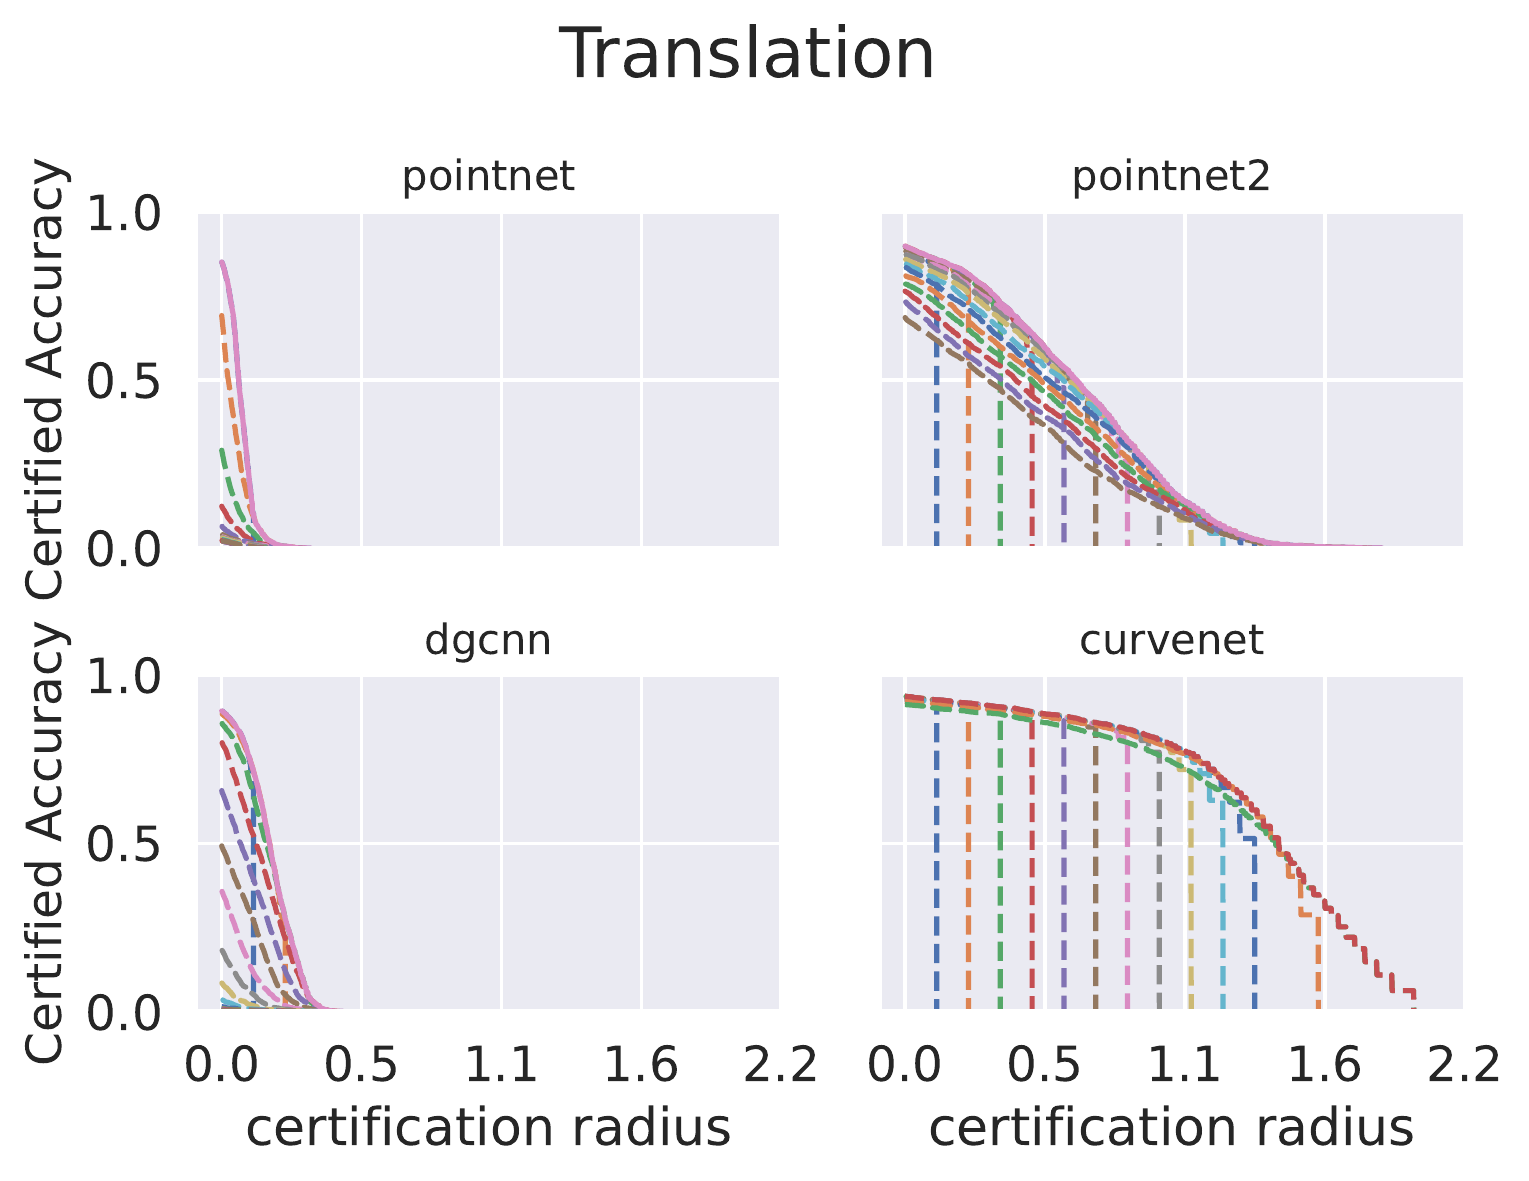}
    \includegraphics[width=\linewidth]{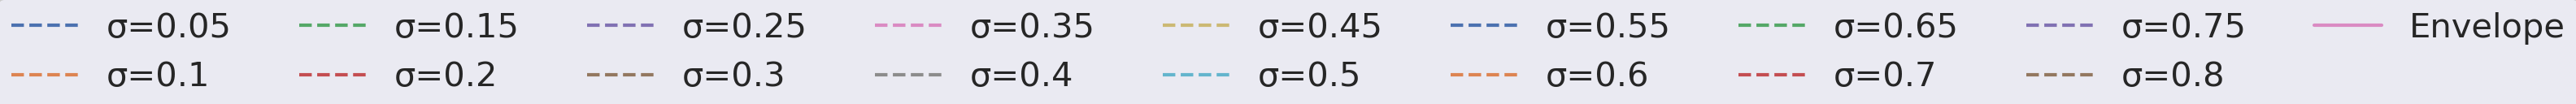}
    \caption{Certified Accuracy against Translation deformations for PointNet, PointNet++, DGCNN and CurveNet with the respective $\sigma$ values explored}
    \label{fig:SuppModelNet40Translation}
\end{figure}

\begin{figure}[h]
    \centering
    \includegraphics[width=\linewidth]{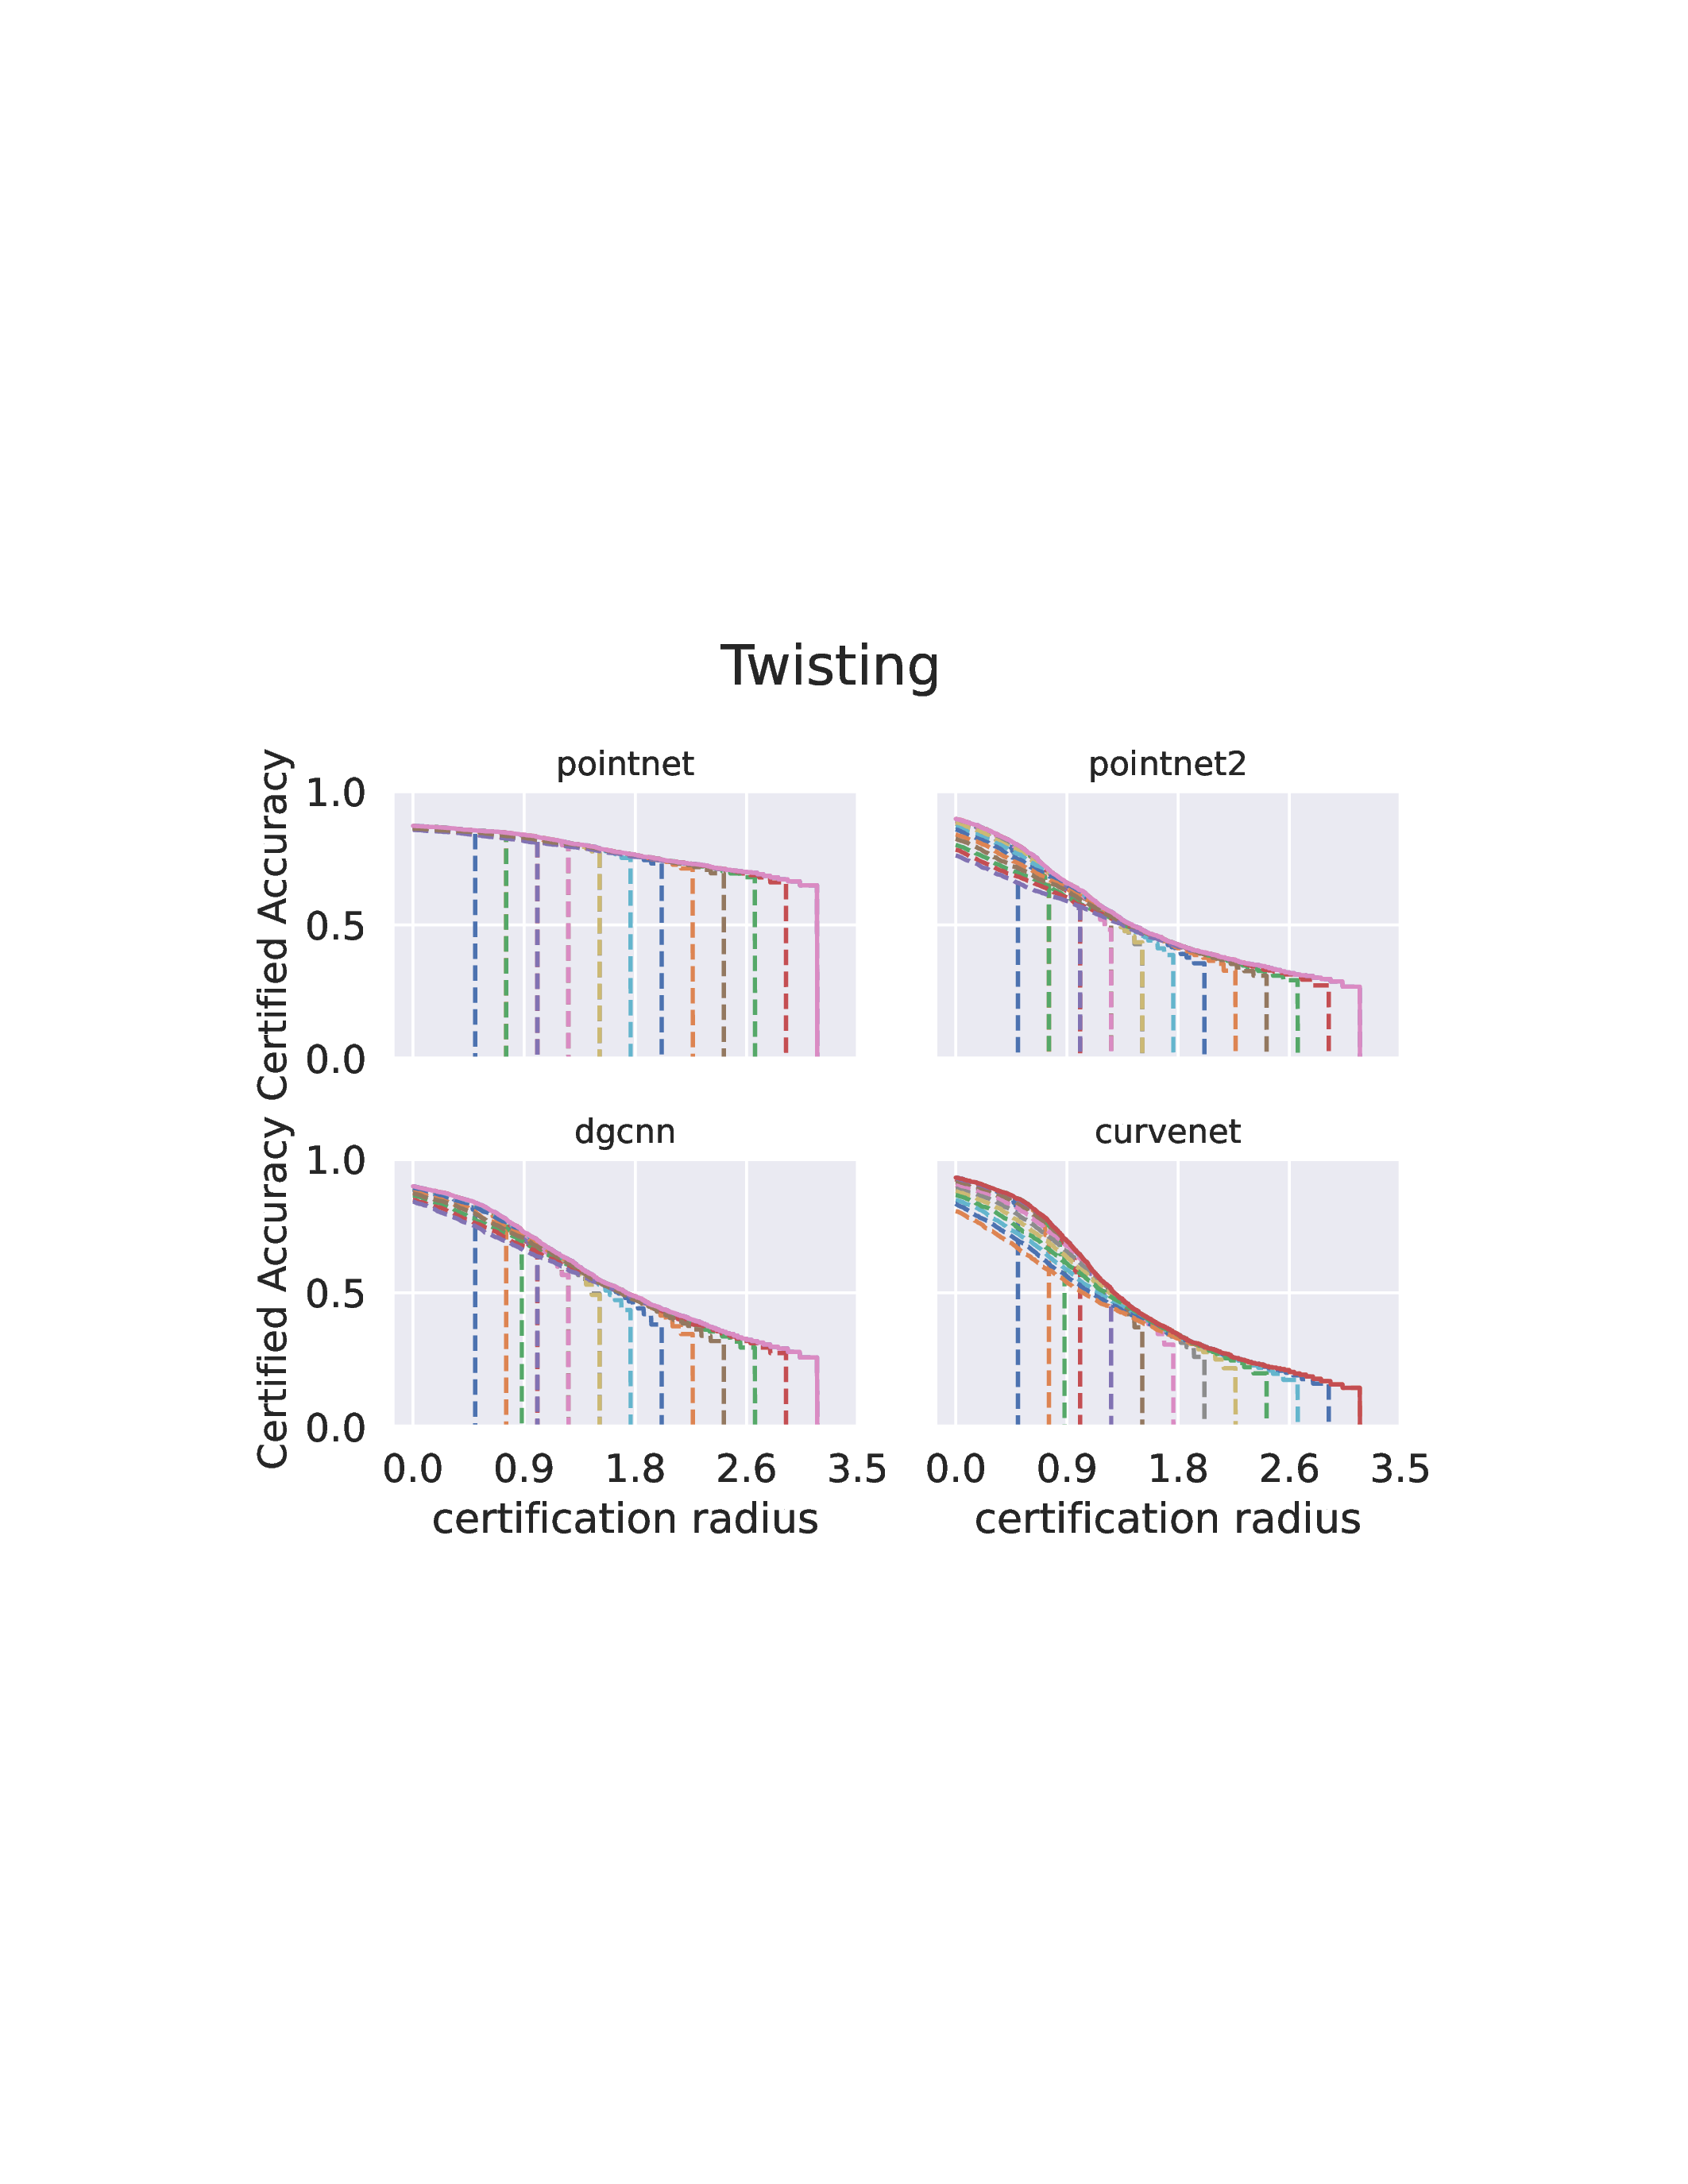}
    \includegraphics[width=\linewidth]{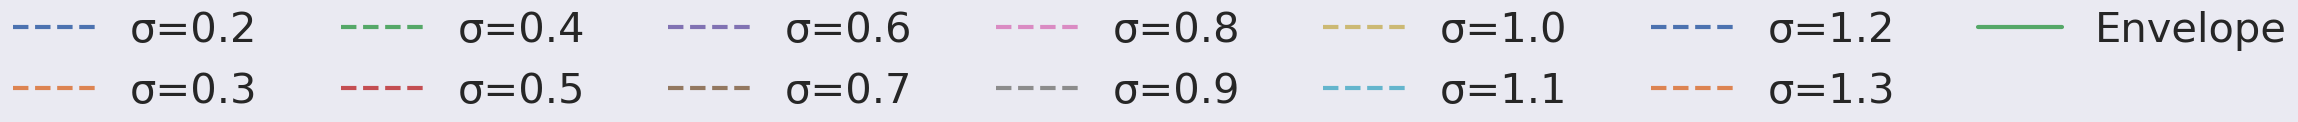}
    \caption{Certified Accuracy against Twisting deformations for PointNet, PointNet++, DGCNN and CurveNet with the respective $\sigma$ values explored}
    \label{fig:SuppModelNet40Twisting}
\end{figure}
