# Supplementary material for: 3DeformRS: Certifying Spatial Deformations on Point Clouds
Source: arXiv:2204.05687 source file (2022-04-12)
Supplement: Supplementary file 4 [file supp_specs.tex]

% \paragraph{lscpu}
\textbf{CPU:}
\begin{verbatim}
Architecture:        x86_64
CPU op-mode(s):      32-bit, 64-bit
Byte Order:          Little Endian
CPU(s):              64
On-line CPU(s) list: 0-63
Thread(s) per core:  2
Core(s) per socket:  16
Socket(s):           2
NUMA node(s):        2
Vendor ID:           GenuineIntel
CPU family:          6
Model:               63
Model name:          Intel(R) Xeon(R) CPU 
                     E5-2698 v3 @ 2.30GHz
Stepping:            2
CPU MHz:             1200.101
CPU max MHz:         3600.0000
CPU min MHz:         1200.0000
BogoMIPS:            4600.21
Virtualization:      VT-x
L1d cache:           32K
L1i cache:           32K
L2 cache:            256K
L3 cache:            40960K
NUMA node0 CPU(s):   0-15,32-47
NUMA node1 CPU(s):   16-31,48-63
\end{verbatim}

% \paragraph{lshw -C display}

\textbf{GPU:}
\begin{verbatim}
description: VGA compatible controller
product: GM200 [GeForce GTX TITAN X]
vendor: NVIDIA Corporation
physical id: 0
bus info: pci@0000:03:00.0
version: a1
width: 64 bits
clock: 33MHz
capabilities: pm msi pciexpress 
vga_controller bus_master cap_list rom
configuration: driver=nvidia latency=0
\end{verbatim}
